# Supplementary material for: Denotational Correctness of Forward-Mode Automatic Differentiation for Iteration and Recursion
Source: arXiv:2007.05282 source file (2024-05-27)
Supplement: Supplementary file 1 [file appendix.pdf]

# A FORWARD AD ON COARSE-GRAIN CBV

We recall that standard coarse-grain CBV, also known as the $\lambda_C$-calculus, computational $\lambda$-calculus, or, plainly, CBV, constructs [Moggi 1988] can be faithfully encoded in fine-grain CBV [Levy 2012; Levy et al. 2003]. This translation $(-)^\dagger$ operates on types and contexts as the identity. It translates terms $\Gamma \vdash t : \tau$ of coarse-grain CBV into computations $\Gamma \vdash^c t^\dagger : \tau$ of fine-grain CBV. This translation illustrates the main difference between coarse-grain and fine-grain CBV: in coarse-grain CBV, values are subset of computations, while fine-grain CBV is more explicit in keeping values and computations separate. This makes it slightly cleaner to formulate an equational theory, denotational semantics, and logical relations arguments.

We list the translation $(-)^\dagger$ below where all newly introduced variables are chosen to be fresh.

| coarse-grain CBV construct $t$ | fine-grain CBV translation $t^\dagger$ |
|---|---|
| $x$ | $\mathbf{return}\, x$ |
| $\underline{c}$ | $\mathbf{return}\, \underline{c}$ |
| $\mathbf{inl}\, t$ | $t^\dagger\ \mathbf{to}\, x.\ \mathbf{return}\ \mathbf{inl}\, x$ |
| $\mathbf{inr}\, t$ | $t^\dagger\ \mathbf{to}\, x.\ \mathbf{return}\ \mathbf{inr}\, x$ |
| $\langle\,\rangle$ | $\mathbf{return}\,\langle\,\rangle$ |
| $\langle t, s\rangle$ | $t^\dagger\ \mathbf{to}\, x.\ s^\dagger\ \mathbf{to}\, y.\ \mathbf{return}\,\langle x, y\rangle$ |
| $\lambda x.t$ | $\mathbf{return}\,\lambda x.t^\dagger$ |
| $\mathbf{roll}\, t$ | $x\ \mathbf{to}\ t^\dagger.\ \mathbf{roll}\, x$ |
| $\mathrm{op}(t_1, \ldots, t_n)$ | $t_1^\dagger\ \mathbf{to}\, x_1.\ \ldots t_n^\dagger\ \mathbf{to}\, x_n.\ \mathrm{op}(x_1, \ldots, x_n)$ |
| $\mathbf{case}\, t\ \mathbf{of}\,\{\,\}$ | $t^\dagger\ \mathbf{to}\, x.\ \mathbf{case}\, x\ \mathbf{of}\,\{\,\}$ |
| $\mathbf{case}\, t\ \mathbf{of}\,\{\mathbf{inl}\, x \to s \mid \mathbf{inr}\, y \to r\}$ | $t^\dagger\ \mathbf{to}\, z.\ \mathbf{case}\, z\ \mathbf{of}\,\{\mathbf{inl}\, x \to s^\dagger \mid \mathbf{inr}\, y \to r^\dagger\}$ |
| $\mathbf{case}\, t\ \mathbf{of}\,\langle\,\rangle \to s$ | $t^\dagger\ \mathbf{to}\, x.\ \mathbf{case}\, x\ \mathbf{of}\,\langle\,\rangle \to s^\dagger$ |
| $\mathbf{case}\, t\ \mathbf{of}\,\langle x, y\rangle \to s$ | $t^\dagger\ \mathbf{to}\, z.\ \mathbf{case}\, z\ \mathbf{of}\,\langle x, y\rangle \to s^\dagger$ |
| $t\, s$ | $t^\dagger\ \mathbf{to}\, x.\ s^\dagger\ \mathbf{to}\, y.\ x\, y$ |
| $\mathbf{iterate}\, t\ \mathbf{from}\, x = s$ | $s^\dagger\ \mathbf{to}\, y.\ \mathbf{iterate}\, t^\dagger\ \mathbf{from}\, x = y$ |
| $\mathbf{sign}\ t$ | $t^\dagger\ \mathbf{to}\, x.\ \mathbf{sign}\ x$ |
| $\mathbf{case}\, t\ \mathbf{of}\ \mathbf{roll}\, x \to s$ | $t^\dagger\ \mathbf{to}\, y.\ \mathbf{case}\, y\ \mathbf{of}\ \mathbf{roll}\, x \to s^\dagger$ |
| $\mu x.t$ | $\mu x.t^\dagger$ |
| $\mathbf{let}\, x = t\ \mathbf{in}\, s$ | $t^\dagger\ \mathbf{to}\, x.\ s^\dagger.$ |

This translation induces a semantics $[\![(-)^\dagger]\!]$ for coarse-grain CBV in $\omega\mathbf{Diff}$, in terms of the semantics $[\![-]\!]$ of fine-grain CBV.

Moreover, it induces the following forward-mode AD rules for coarse-grain CBV. The macro $\overrightarrow{\mathcal{D}}(-)$ on types is as for fine-grain CBV. On terms, we define a single macro $\overrightarrow{\mathcal{D}}(-)$ by

$$
\begin{aligned}
\overrightarrow{\mathcal{D}}(x) &\stackrel{\text{def}}{=} x\\
\overrightarrow{\mathcal{D}}(\underline{c}) &\stackrel{\text{def}}{=} \langle \underline{c}, \underline{0}\rangle\\
\overrightarrow{\mathcal{D}}(\mathbf{inl}\, t) &\stackrel{\text{def}}{=} \mathbf{inl}\, \overrightarrow{\mathcal{D}}(t)\\
\overrightarrow{\mathcal{D}}(\mathbf{inr}\, t) &\stackrel{\text{def}}{=} \mathbf{inr}\, \overrightarrow{\mathcal{D}}(t)\\
\overrightarrow{\mathcal{D}}(\langle\,\rangle) &\stackrel{\text{def}}{=} \langle\,\rangle\\
\overrightarrow{\mathcal{D}}(\langle t, s\rangle) &\stackrel{\text{def}}{=} \langle \overrightarrow{\mathcal{D}}(t), \overrightarrow{\mathcal{D}}(s)\rangle\\
\overrightarrow{\mathcal{D}}(\lambda x.t) &\stackrel{\text{def}}{=} \lambda x.\overrightarrow{\mathcal{D}}(t)\\
\overrightarrow{\mathcal{D}}(\mathbf{roll}\, t) &\stackrel{\text{def}}{=} \mathbf{roll}\, \overrightarrow{\mathcal{D}}(t)\\
\overrightarrow{\mathcal{D}}(\mathrm{op}(t_1, \ldots, t_n)) &\stackrel{\text{def}}{=} \begin{array}{l} \mathbf{case}\, \overrightarrow{\mathcal{D}}(t_1)\, \mathbf{of}\, \langle x_1, x_1'\rangle \to \\ \vdots \\ \mathbf{case}\, \overrightarrow{\mathcal{D}}(t_n)\, \mathbf{of}\, \langle x_n, x_n'\rangle \to \\ \langle \mathrm{op}(x_1, \ldots, x_n), x_1' * \partial_1 \mathrm{op}(x_1, \ldots, x_n) + \ldots + x_n' * \partial_n \mathrm{op}(x_n, \ldots, x_n)\rangle \end{array}\\
\overrightarrow{\mathcal{D}}(\mathbf{case}\, t\, \mathbf{of}\, \{\,\}) &\stackrel{\text{def}}{=} \mathbf{case}\, \overrightarrow{\mathcal{D}}(t)\, \mathbf{of}\, \{\,\}\\
\overrightarrow{\mathcal{D}}(\mathbf{case}\, t\, \mathbf{of}\, \{ \begin{array}{l} x \to s \\ \mid y \to r\} \end{array}) &\stackrel{\text{def}}{=} \mathbf{case}\, \overrightarrow{\mathcal{D}}(t)\, \mathbf{of}\, \{\mathbf{inl}\, x \to \overrightarrow{\mathcal{D}}(s) \mid \mathbf{inr}\, y \to \overrightarrow{\mathcal{D}}(r)\}\\
\overrightarrow{\mathcal{D}}(\mathbf{case}\, t\, \mathbf{of}\, \langle\,\rangle \to s) &\stackrel{\text{def}}{=} \mathbf{case}\, \overrightarrow{\mathcal{D}}(t)\, \mathbf{of}\, \langle\,\rangle \to \overrightarrow{\mathcal{D}}(s)\\
\overrightarrow{\mathcal{D}}(\mathbf{case}\, t\, \mathbf{of}\, \langle x, y\rangle \to s) &\stackrel{\text{def}}{=} \mathbf{case}\, \overrightarrow{\mathcal{D}}(t)\, \mathbf{of}\, \langle x, y\rangle \to \overrightarrow{\mathcal{D}}(s)\\
\overrightarrow{\mathcal{D}}(t\, s) &\stackrel{\text{def}}{=} \overrightarrow{\mathcal{D}}(t)\, \overrightarrow{\mathcal{D}}(s)\\
\overrightarrow{\mathcal{D}}(\mathbf{iterate}\, t\, \mathbf{from}\, x = s) &\stackrel{\text{def}}{=} \mathbf{iterate}\, \overrightarrow{\mathcal{D}}(t)\, \mathbf{from}\, x = \overrightarrow{\mathcal{D}}(s)\\
\overrightarrow{\mathcal{D}}(\mathbf{sign}\, t) &\stackrel{\text{def}}{=} \mathbf{sign}\, \overrightarrow{\mathcal{D}}(t)\\
\overrightarrow{\mathcal{D}}(\mathbf{case}\, t\, \mathbf{of}\, \mathbf{roll}\, x \to s) &\stackrel{\text{def}}{=} \mathbf{case}\, \overrightarrow{\mathcal{D}}(t)\, \mathbf{of}\, \mathbf{roll}\, x \to \overrightarrow{\mathcal{D}}(s)\\
\overrightarrow{\mathcal{D}}(\mu x.t) &\stackrel{\text{def}}{=} \mu x.\overrightarrow{\mathcal{D}}(t)\\
\overrightarrow{\mathcal{D}}(\mathbf{let}\, x = t\, \mathbf{in}\, s) &\stackrel{\text{def}}{=} \mathbf{let}\, x = \overrightarrow{\mathcal{D}}(t)\, \mathbf{in}\, \overrightarrow{\mathcal{D}}(s)
\end{aligned}
$$

where $x_1 : \mathbf{real}, \ldots, x_n : \mathbf{real} \vdash \partial_i \mathrm{op}(x_1, \ldots, x_n) : \mathbf{real}$ are chosen terms to represent the $i$-th partial derivative of the $n$-ary operation op. Then, $\overrightarrow{\mathcal{D}}(t)^{\dagger} = \overrightarrow{\mathcal{D}}_C(t^{\dagger})$.

The following correctness theorem for forward AD on coarse-grain CBV is a direct consequence of the corresponding correctness theorem for fine-grain CBV.

Theorem (Correctness of Fwd AD). *For any $x_1 : \tau_1, \ldots, x_n : \tau_n \vdash t : \sigma$, where $\tau_i, \sigma$ are first-order types, we have that $[\![\overrightarrow{\mathcal{D}}(t)^{\dagger}]\!](x, v) = ([\![t^{\dagger}]\!](x), \mathcal{T}_x [\![t^{\dagger}]\!] v)$, for all $x$ in the domain of $[\![t^{\dagger}]\!]$ and $v$ tangent vectors at $x$. Moreover, $[\![\overrightarrow{\mathcal{D}}(t)^{\dagger}]\!](x, v)$ is defined iff $[\![t^{\dagger}]\!](x)$ is.*

## B OPERATIONAL CONSIDERATIONS

The value of our correctness proof of forward AD based on a denotational semantics entirely depends on whether the reader believes that the specified semantics is in some sense correct. Recall that our category $\omega$**Diff** forms a conservative extension of the category **Man** of manifolds and smooth functions, while **p**$\omega$**Diff** is a conservative extension of that **pMan** of manifolds and smooth partial functions, completing them to bicartesian closed category with a bilimit compact expansion. As such, we can interpret a higher-order language with recursive types, while the first-order fragment of our language gets its standard interpretation in **Man** and **pMan**, possibly the most canonical setting for differential geometry. Note that even programs which contain higher-order sub-programs get interpreted in **Man** and **pMan**, as long as their types are first-order.

Still, however, some readers might be interested to understand the connection with the operational semantics of our language in order to be convinced that the specified denotational semantics is of value. We detail that correspondence here.

As a fine-grain CBV language, we have an uncontroversal operational semantics: as a small-step semantics $t \rightsquigarrow s$, we simply use a directed version of the $\beta$-rules of our language, supplemented with rules which specify how to evaluate basic operations.

$$
\begin{array}{lll}
\mathbf{return}\,v\,\mathbf{to}\,x.\,t \rightsquigarrow t[^v/_x] & & \mathbf{case\,inl}\,v\,\mathbf{of}\,\{\mathbf{inl}\,x \to t \mid \mathbf{inr}\,y \to s\} \rightsquigarrow t[^v/_x] \\
\mathbf{case}\,\langle v, w\rangle\,\mathbf{of}\,\langle x, y\rangle \to t \rightsquigarrow t[^v/_x, {}^w/_y] & & \mathbf{case\,inr}\,v\,\mathbf{of}\,\{\mathbf{inl}\,x \to t \mid \mathbf{inr}\,y \to s\} \rightsquigarrow s[^v/_y] \\
(\lambda x.t)\; v \rightsquigarrow t[^v/_x] & & \mathbf{case\,roll}\,v\,\mathbf{of\,roll}\,x \to t \rightsquigarrow t[^v/_x] \\
\mathrm{op}(\underline{c_1}, \ldots, \underline{c_n}) \rightsquigarrow \mathbf{return}\;\underline{[\![\mathrm{op}]\!](c_1, \ldots, c_n)} & & (\text{for } (c_1, \ldots, c_n) \in \mathrm{Dom}\,([\![\mathrm{op}]\!])) \\
\mathbf{sign}\,\underline{c} \rightsquigarrow \mathbf{return\,inl}\,\langle\,\rangle \quad \mathbf{sign}\,\underline{-c} \rightsquigarrow \mathbf{return\,inr}\,\langle\,\rangle & & (\text{for } c > 0).
\end{array}
$$

Observe that this immediately determines the operational semantics for our sugar **if** $v$ **then** $t$ **else** $s$, **iterate** $t$ **from** $x = v$, and $\mu x.t$ as well as for coarse-grain CBV.

From this small-step semantics, we can define a big-step semantics $t \Downarrow v \stackrel{\mathrm{def}}{=} t \rightsquigarrow^* \mathbf{return}\,v$, where we write $\rightsquigarrow^*$ for the transitive closure of $\rightsquigarrow$.

*Program contexts of type* $\sigma$ *with a hole* $-$ *of type* $\Gamma \vdash \tau$ are terms $C[\Gamma \vdash - : \tau]$ of type $\sigma$ with a single variable of type $\tau$, where this variable $-$ always occurs inside the term in contexts $\Gamma' \geq \Gamma$. Write $C[t]$ for the *capturing* substitution $C[\Gamma \vdash - : \tau][^t/_-]$.

Two computations $\Gamma \vdash^c t, s : \tau$ are in the *contextual preorder* $t \precsim s$ when for all program contexts $C[\Gamma \vdash - : \tau]$ of type **real**, we have that $C[t] \Downarrow v$ implies that $C[s] \Downarrow v$. We say that $t$ and $s$ are *contextually equivalent*, writing $t \approx s$, when $t \precsim s$ and $s \precsim t$

We can now state and prove adequacy of our denotational semantics with respect to this operational semantics.

Theorem B.1 (Adequacy). *Suppose that two computations* $\vdash t : \tau$ *and* $\vdash s : \tau$ *are comparable in our denotational semantics in* $\omega$**Diff** *in the sense that* $[\![t]\!] \leq [\![s]\!]$. *Then,* $t \approx s$ *in the observational preorder. In particular,* $[\![t]\!] = [\![s]\!]$ *implies that* $t \precsim s$.

Proof (Sketch). It is enough to show the corresponding statement for the induced denotational semantics $|[\![-]\!]|$ of our language in $\boldsymbol{\omega}$**CPO**, if we forget about the diffeology. Indeed, the bicartesian closed structure, as well as the bilimit compact expansion structures of $\omega$**Diff** lift those in $\boldsymbol{\omega}$**CPO** while also $[\![t]\!] \leq [\![s]\!]$ iff $|[\![t]\!]| \leq |[\![s]\!]|$. That is, what we need to do is a standard adequacy over a semantics in $\boldsymbol{\omega}$**CPO** of a standard CBV language. This is precisely the setting where the traditional methods of [Pitts 1996] apply. Indeed, we can simply use a minor extension of the adequacy proof given in [Pitts 1996]: we define the logical relation at **real** as $r \trianglelefteq^{\vdash \mathbf{real}} \underline{r}$ and we add two more cases to the induction for the fundamental lemma, one for **sign** and one for op. These two steps in the fundamental lemma go through almost tautologically because of our choice of denotational

semantics precisely matches the operational semantics for these constructs. Once the fundamental lemma is established, the adequacy theorem again follows because the interpretation of values in our semantics remains injective (faithful), even once we add the type **real** (indeed, values $\underline{c}$ of type **real** are in 1-1-correspondence with real numbers $c \in \mathbb{R}$). □

This shows that our denotational semantics is, in particular, a sound method for proving contextual equivalences of the operational semantics.

# C CHARACTERIZING $\omega$Diff

We describe three additional categories equivalent to $\omega$**Diff**. Each approaches the question of how to combine diffeological and $\omega$-cpo structures in a different way. We summarise the characterisations:

**Theorem 7.1.** We have equivalences of categories: $\omega\mathbf{Diff} \simeq \mathcal{E}_{\omega q} \simeq \boldsymbol{\omega}\mathbf{CPO}(\mathbf{Diff}) \simeq \boldsymbol{\omega}\mathbf{diff}\text{−}\mathbf{Mod}(\mathbf{Set})$.

We describe these equivalent categories. For our semantics, we only need these consequences:

**Corollary 7.2.** The category of $\omega$-diffeological spacees, $\omega$**Diff**, is locally $\mathfrak{c}^+$-presentable, where $\mathfrak{c}^+$ is the successor cardinal of the continuum. In particular, it has all small limits and colimits.

## C.1 $\mathcal{E}_{\omega q}$: a Domain-Theoretic Completion of Multivariate Calculus

Diffeological spaces are a quasi-topos completion of the category **Open** of open subsets of some $\mathbb{R}^n$ and smooth functions. Indeed [Baez and Hoffnung 2011] establish an equivalence $-^\sharp : \mathcal{E}_q \simeq \mathbf{Diff}$, where $\mathcal{E}_q$ is the full sub-category of presheaves $[\mathbf{Open}^{\mathrm{op}}, \mathbf{Set}]$ consisting of those functors $F : \mathbf{Open}^{\mathrm{op}} \to \mathbf{Set}$ that are:

- sheaves with respect to open covers; and
- separated: the functions $m_F \stackrel{\text{def}}{=} (F\underline{r})_{r\in U} : FU \to \prod_{r\in U} F\mathbb{1}$ are injective, for all $U \in \mathbf{Open}$.

This equivalence is given on objects by mapping $F$ to the diffeological space $F^\sharp$ whose carrier is $F\mathbb{1}$ and whose $U$-plots are the image $m_F[FU]$ under the injection from the separatedness condition. Therefore, $m_F : FU \to \prod_{r\in U} F\mathbb{1}$ restricts to a bijection $\xi_F : FU \cong S^U_{F^\sharp}$. The equivalence is given on morphisms $\alpha : F \to G$ by $\alpha^\sharp \stackrel{\text{def}}{=} \alpha_{\mathbb{1}}$. Given any **Diff**-morphism $f : F^\sharp \to G^\sharp$, by setting:

$$\alpha_U : FU \xrightarrow{\xi_F} S^U_{F^\sharp} \xrightarrow{(-);f} S^U_{G^\sharp} \xrightarrow{\xi_G} GU$$

we obtain the natural transformation $\alpha : F \to G$ for which $\alpha^\sharp = f$. As an adjoint equivalent to $-^\sharp$, we can choose, for every diffeological space $X$, the separated sheaf $X^\flat a := X^a$ where $a$ is either an object or a morphism, and the (co)unit of this adjoint equivalence is given by $\eta_X : X^{\flat\sharp} = X^\flat\mathbb{1} = X^{\mathbb{1}} \xrightarrow{\cong} X$. (See [Baez and Hoffnung 2011] for a more detailed discussion of this equivalence.)

We define a similar category $\mathcal{E}_{\omega q}$ to be the full subcategory of $[\mathbf{Open}^{\mathrm{op}}, \boldsymbol{\omega}\mathbf{CPO}]$ consisting of those functors $F : \mathbf{Open}^{\mathrm{op}} \to \boldsymbol{\omega}\mathbf{CPO}$ that are:

- sheaves; and
- $\boldsymbol{\omega}$**CPO**-separated: the functions $m_F \stackrel{\text{def}}{=} (F\underline{r})_{r\in U} : FU \to \prod_{r\in U} F\mathbb{1}$ are full monos for all $U \in \mathbf{Open}$.

Post-composing with the forgetful functor $|-| : \mathbf{Diff} \to \mathbf{Set}$ yields a forgetful functor $|-| : \mathcal{E}_{\omega q} \to \mathcal{E}_q$, as the underlying function of a full mono is injective.

We equip $\mathcal{E}_{\omega q}$ with an $\boldsymbol{\omega}$**CPO**-category structure by setting the order componentwise:

$$\alpha \leq \beta \qquad \Longleftrightarrow \qquad \forall U \in \mathbf{Open}.\alpha_U \leq \beta_U$$

Recall that an $\boldsymbol{\omega}$**CPO**-*equivalence* is an adjoint pair of locally-continuous functors whose unit and counit are isomorphisms. To specify an $\boldsymbol{\omega}$**CPO**-equivalence, it suffices to give a fully-faithful

locally-continuous essentially surjective functor in either way, together with a choice of sources and isomorphisms for the essential surjectivity.

**Proposition 7.3.** The equivalence $-^{\sharp} : \mathcal{E}_{\omega q} \simeq \omega\mathbf{Diff}$ of 7.1 is $\boldsymbol{\omega}$**CPO**-enriched, and given by:

$$F^{\sharp} := (|F\mathbb{1}|, m_F[F\mathbb{R}], \leq_{F\mathbb{1}}) \qquad\qquad (\alpha : F \to G)^{\sharp} := \alpha_{\mathbb{1}}$$

Moreover, the two forgetful functors $|-| : \mathcal{E}_{\omega q} \to \mathcal{E}_q$ and $|-| : \omega\mathbf{Diff} \to \mathbf{Diff}$ form a map of adjoints.

## C.2 $\boldsymbol{\omega}$CPO(Diff): $\omega$-cpos Internal to Diff

The category **Diff** is a Grothendieck quasi-topos, which means it has a canonical notion of a sub-space: *strong monos*. Sub-spaces let us define relations/predicates, and interpret a fragment of higher-order logic formulae as subspaces. In particular, we can interpret $\omega$-cpo's definition *internally* to **Diff** and Scott-continuous morphisms between such $\omega$-cpos as a subspace of the **Diff**-function space, to form the category $\boldsymbol{\omega}$**CPO**(**Diff**). We interpret functional operations, like the sup-operation of a $\omega$-cpo and the homorphisms of $\omega$-cpos, as internal functions, rather than as internal functional relations, as the two notions differ in a non-topos quasi-topos such as **Diff**.

## C.3 $\boldsymbol{\omega}$diff−Mod(Set): Models of an Essentially Algebraic Theory

Both $\boldsymbol{\omega}$**CPO** and **Diff** are locally presentable categories. Therefore, there are essentially algebraic theories $\boldsymbol{\omega}$**cpo** and **qbs** and equivalences $\boldsymbol{\omega}$**cpo**−**Mod**(**Set**) $\simeq$ $\boldsymbol{\omega}$**CPO** and **qbs**−**Mod**(**Set**) $\simeq$ **Diff** of their categories of set-theoretic algebras. We combine these two presentations into a presentation $\boldsymbol{\omega}$**diff** for $\omega$-diffeological space, given in the following subsections, by taking their union, identifying the element sorts and adding a sup operation for $\omega$-chains of the random elements, and a single axiom stating this sup is computed pointwise. Local presentability, for example, implies the existence of all small limits and colimits.

An $\omega$-cpo or a diffeological space are essentially algebraic, in a precise sense [Adámek et al. 1994, Chapter 3.D]. We will use this algebraic nature to analyse the diffeological domains and see how the diffeological structure interacts with the $\omega$-cpo structure.

*C.3.1 Presentations.* For the following, fix a regular cardinal $\kappa$. Given a set $\mathcal{S}$ with cardinality $|\mathcal{S}| < \kappa$, whose elements we call *sorts*, an $\mathcal{S}$*-sorted ($\kappa$-ary) signature* $\Sigma$ is a pair $\Sigma = (O, \text{arity})$ consisting of a set of *operations* and $\text{arity} : O \to \mathcal{S}^{<\kappa} \times \mathcal{S}$ assigns to each operation $\text{op} \in O$ a sequence $(s_i)_{i\in I}$, indexed by some set $I$ of cardinality $|I| < \kappa$, assigning to each index $i \in I$ its *argument sort*, together with another *result sort* $s$. We write $(\text{op} : \prod_{i\in I} s_i \to s) \in \Sigma$ for $\text{arity}(\text{op}) = ((s_i)_{i\in I}, s)$.

Given an $\mathcal{S}$-sorted signature $\Sigma$, and a $\mathcal{S}$-indexed sequence of sets $\mathbb{V} = (\mathbb{V}_s)_{s\in\mathcal{S}}$ of *variables* we define the collections of $\mathcal{S}$-sorted terms $\text{Term}^{\Sigma}\,\mathbb{V} = \left(\text{Term}^{\Sigma}_s\,\mathbb{V}\right)_{s\in\mathcal{S}}$ over $\mathbb{V}$ inductively as follows:

$$\frac{}{x \in \text{Term}_s\,\mathbb{V}}(x \in \mathbb{V}_s) \qquad \frac{\text{for all } i \in I,\, t_i \in \text{Term}_{s_i}\,\mathbb{V}}{\text{op}\,(t_i)_{n\in A} \in \text{Term}_s\,\mathbb{V}}((\text{op} : \prod_{i\in I} s_i \to s) \in \Sigma)$$

Given a signature $\Sigma$ and a sort $s$, an *equation of sort* $s$ is a pair of terms $(t_1, t_2) \in \text{Term}_s\,\mathbb{V}$ over some set of variables. As each term must involve less than $\kappa$-many variables, due to $\kappa$'s regularity we may fix the indexed set of variables $\mathbb{V}$ to be any specified collection of sets of cardinality $\kappa$.

*Definition C.1.* An *essentially algebraic presentation* $\mathcal{P}$ is a tuple $\left(\mathcal{S}, \Sigma_t, \Sigma_p, \text{Def}, \text{Eq}\right)$ containing:

- a set $\mathcal{S}$ of *sorts*;
- two $\mathcal{S}$-sorted signatures with disjoint sets of operations:
  - a signature $\Sigma_t$ of *total* operations;

  - a signature $\Sigma_p$ of *partial* operations;

  we denote their combined signature by $\Sigma \stackrel{\text{def}}{=} \left(O_{\Sigma_t} \cup O_{\Sigma_p}, [\text{arity}_{\Sigma_t}, \text{arity}_{\Sigma_p}]\right)$;
- for each $(\text{op} : \prod_{i \in I} s_i \longrightarrow s) \in \Sigma_p$, a set $\text{Def}(\text{op})$ of $\Sigma_t$-equations over the variables $\{x_i : s_i | i \in I\}$ which we call the *assumptions of* $\text{op}\,(x_i)_{i \in I}$; and
- a set Eq of $\Sigma$-equations which we call the *axioms*.

The point of this definition is just to introduce the relevant vocabulary. We will only be considering the following presentation for posets, then $\omega$-cpos, then diffeological spaces:

**Example 13** (poset presentation cf. [Adámek et al. 1994, Examples 3.35(1),(4)])**.** The presentation of *posets*, **pos**, has two sorts:

- element, which will be the carrier of the poset; and
- inequation, which will describe the poset structure.

The total operations are:

- $\text{lower} : \text{inequation} \longrightarrow \text{element}$, assigning to each inequation its lower element;
- $\text{upper} : \text{inequation} \longrightarrow \text{element}$, assigning to each inequation its upper element;
- $\text{refl} : \text{element} \longrightarrow \text{inequation}$, used to impose reflexivity;

The partial operations are:

- $\text{irrel} : \text{inequation} \times \text{inequation} \longrightarrow \text{inequation}$, used to impose proof-irrelevance on inequations, with $\text{Def}(\text{irrel}(e_1, e_2))$:
$$\text{lower}(e_1) = \text{lower}(e_2) \qquad \text{upper}(e_1) = \text{upper}(e_2)$$
- $\text{antisym} : \text{inequation} \times \text{inequation} \longrightarrow \text{element}$, used to impose anti-symmetry, with $\text{Def}(\text{antisym}(e, e^{\text{op}}))$:
$$\text{lower}(e) = \text{upper}(e^{\text{op}}) \qquad \text{upper}(e) = \text{lower}(e^{\text{op}})$$
- $\text{trans} : \text{inequation} \times \text{inequation} \longrightarrow \text{inequation}$, used to impose transitivity, with $\text{Def}(\text{trans}(e_1, e_2))$:
$$\text{upper}(e_1) = \text{lower}(e_2)$$

The axioms are:

$$e_1 = \text{irrel}(e_1, e_2) = e_2 \qquad \text{(proof irrelevance)}$$
$$\text{lower}(\text{refl}(x)) = x = \text{upper}(\text{refl}(x)) \qquad \text{(reflexivity)}$$
$$\text{lower}(e_1) = \text{antisym}(e_1, e_2) = \text{lower}(e_2) \qquad \text{(anti-symmetry)}$$
$$\text{lower}(\text{trans}(e_1, e_2)) = \text{lower}(e_1) \qquad \text{upper}(\text{trans}(e_1, e_2)) = \text{upper}(e_2) \qquad \text{(transitivity)}$$

□

**Example 14** ($\omega$-cpo presentation)**.** In addition to the operations and axioms for posets, the presentation $\boldsymbol{\omega}$**cpo** of $\omega$-cpos includes the following partial operations:

- $\bigvee : \prod_{n \in \mathbb{N}} \text{inequation} \longrightarrow \text{element}$, used to express lubs of $\omega$-chains, with $\text{Def}(\bigvee_{n \in \mathbb{N}} e_n)$:
$$\text{upper}(e_n) = \text{lower}(e_{n+1}), \text{for each } n \in \mathbb{N}$$
- for each $k \in \mathbb{N}$, $\text{ub}_k : \prod_{n \in \mathbb{N}} \text{element} \longrightarrow \text{inequation}$, collectively used to impose the lub being an upper-bound, with $\text{Def}(\text{ub}_k\,((e_n))_{n \in NN})$:
$$\text{upper}(e_n) = \text{lower}(e_{n+1}), \text{for each } n \in \mathbb{N}$$

- least : element $\times \prod_{n\in\mathbb{N}}$ inequation $\times \prod_{n\in\mathbb{N}}$ inequation $\longrightarrow$ inequation, used to express that the lub is the least bound, with $\mathrm{Def}(\mathrm{least}(x, (e_n)_{n\in\mathbb{N}}, (b_n)_{n\in\mathbb{N}}))$:

$$\mathrm{upper}(e_n) = \mathrm{lower}(e_{n+1}) \qquad \mathrm{upper}(b_n) = x \qquad \mathrm{lower}(e_n) = \mathrm{lower}(b_n), \text{for each } n \in \mathbb{N}$$

The axioms are:

$$\mathrm{lower}(\mathrm{ub}_k\,(e_n)_n) = \mathrm{lower}(e_k) \qquad \mathrm{upper}(\mathrm{ub}_k\,(e_n)_n) = \bigvee (e_n)_n \qquad \text{(upper bound)}$$

$$\mathrm{lower}(\mathrm{least}(x, (e_n)_n, (b_n)_n)) = \bigvee (e_n)_n \qquad \mathrm{upper}(\mathrm{least}(x, (e_n)_n, (b_n)_n)) = x \qquad \text{(least upper bound)}$$

□

**Example 15** (**diff** presentation)**.** The presentation of *diffeological spaces*, **diff**, has continuum many sorts:

- element, which will be the carrier of the diffeological space; and
- $\mathrm{plot}_U$, for each $U \in \mathbf{Open}$, which will be the $U$-indexed plots.

The total operations are:

- $\mathrm{ev}_r : \mathrm{plot}_U \longrightarrow$ element, for each $r \in U$, evaluating a plot at $r \in U$;
- const : element $\longrightarrow \mathrm{plot}_U$ assigning to each element $x$ the constantly-$x$ plot; and
- $\mathrm{rearrange}_\varphi : \mathrm{plot}_V \longrightarrow \mathrm{plot}_U$, for each smooth $\varphi : U \longrightarrow V$, precomposing plots with $\varphi$.

There are two partial operations:

- ext : $\mathrm{plot}_U \times \mathrm{plot}_U \longrightarrow \mathrm{plot}_U$, used for establishing that a plot is uniquely determined extensionally, with $\mathrm{Def}(\mathrm{ext}(\alpha, \beta))$ given by

$$\{\mathrm{ev}_r(\alpha) = \mathrm{ev}_r(\beta) : \mathrm{element} | r \in U\}$$

  and
- $\mathrm{match}_{\mathcal{U}} : \prod_{U\in\mathcal{U}} \mathrm{plot}_U \longrightarrow \mathrm{plot}_W$, for each open cover $\mathcal{U}$ of $W$, with $\mathrm{Def}(\mathrm{match}_{\mathcal{U}}\,(f_U)_{U\in\mathcal{U}})$ given by:

$$\{\mathrm{ev}_r(f_U) = \mathrm{ev}_r(f_V) | U, V \in \mathcal{U}, r \in U \cap V\}$$

  used for pasting together a $\mathcal{U}$-indexed family of compatible plots into a case split.

The axioms are:

$$\alpha = \mathrm{ext}(\alpha, \beta) = \beta \qquad \text{(extensionality)}$$

$$\{\mathrm{ev}_r(\mathrm{const}\,(x)) = x | r \in U\} \qquad \text{(constantly)}$$

$$\left\{\mathrm{ev}_r(\mathrm{rearrange}_\varphi\,\alpha) = \mathrm{ev}_{\varphi(r)}\,\alpha \middle| \varphi : U \longrightarrow V \in \mathbf{Open}, r \in U\right\} \qquad \text{(rearrange)}$$

$$\left\{\mathrm{ev}_r\left(\mathrm{match}_{\mathcal{U}}\,(\alpha_U)_{U\in\mathcal{U}}\right) = \mathrm{ev}_r(\alpha_U) \middle| \mathcal{U} \text{ open cover of } W, U \in \mathcal{U}, r \in U\right\} \qquad \text{(match)}$$

□

We can now present $\omega$-diffeological spacees:

**Example 16** ($\omega$-diffeological space presentation)**.** The presentation $\boldsymbol{\omega}$**diff** of $\omega$-diffeological spacees extends the presentations $\boldsymbol{\omega}$**cpo** and **diff**, identifying the element sort, with the following additional partial operations, for all $U \in \mathbf{Open}$:

- $\bigsqcup : \prod_{n\in\mathbb{N}} \mathrm{plot}_U \times \prod_{n\in\mathbb{N}, r\in U}$ inequation $\longrightarrow \mathrm{plot}_U$, used for establishing that the plots are closed under lubs w.r.t. the pointwise order, with $\mathrm{Def} \bigsqcup((\alpha_n)_{n\in\mathbb{N}}, (e_n^r)_{n\in\mathbb{N}, r\in U})$ given by:

$$\left\{\mathrm{lower}(e_n^r) = \mathrm{ev}_r(\alpha_n), \mathrm{upper}(e_n^r) = \mathrm{ev}_r(\alpha_{n+1}), \middle| n \in \mathbb{N}, r \in U\right\}$$

The additional axioms are:

$$\left\{\mathrm{ev}_r\left(\bigsqcup\left((\alpha_n)_{n\in\mathbb{N}}, (e^r_n)_{n\in\mathbb{N},r\in U}\right)\right) = \bigvee (e^r_n)_{n\in\mathbb{N}} \middle| r\in U\right\} \qquad \text{(pointwise lubs)}$$

□

*C.3.2 Algebras.* Every essentially algebraic presentation induces a category of set-theoretic models, and this category for the $\omega$-cpo presentation is equivalent to $\boldsymbol{\omega}$**CPO**. Moreover, we can interpret such presentations in any category with sufficient structure, namely countable products and equalisers (i.e., countable limits). We briefly recount how to do this.

Let $C$ be a category with $\lambda$-small limits, with $\lambda$ regular. As usual, if $\Sigma$ is any $\mathcal{S}$-sorted $\lambda$-ary signature, we define a (multi-sorted) $\Sigma$-*algebra* $A = \left(\left(\llbracket s\rrbracket\right)_{s\in\mathcal{S}}, \llbracket -\rrbracket\right)$ to consist of an $\mathcal{S}$-indexed family of objects $\left(\llbracket s\rrbracket\right)_{s\in\mathcal{S}}$, the *carrier* of the algebra, and an assignment, to each $\mathrm{op} : \prod_{i\in I} s_i \to s$ in $\Sigma$, of a morphism:

$$\llbracket \mathrm{op}\rrbracket : \prod_{i\in I}\llbracket s_i\rrbracket \to \llbracket s\rrbracket$$

Given such an algebra $A$, and an $\mathcal{S}$-indexed set $\mathbb{V}$ of variables with $|\mathbb{V}_s| < \lambda$ for each $s\in\mathcal{S}$, each term $t$ in $\mathrm{Term}_s\,\mathbb{V}$ denotes a morphism:

$$\llbracket t\rrbracket_s : \prod_{s\in\mathcal{S}}\llbracket s\rrbracket^{\mathbb{V}_s} \to \llbracket s\rrbracket$$

as follows:

$$\llbracket x\rrbracket_s : \prod_{s\in\mathcal{S}}\llbracket s\rrbracket^{\mathbb{V}_s} \xrightarrow{\pi_s} \llbracket s\rrbracket^{\mathbb{V}_s} \xrightarrow{\pi_x} \llbracket s\rrbracket \qquad \llbracket \mathrm{op}\,(t_i)_{i\in I}\rrbracket : \prod_{s\in\mathcal{S}}\llbracket s\rrbracket^{\mathbb{V}_s} \xrightarrow{(\llbracket t_i\rrbracket)_{i\in I}} \prod_{i\in I}\llbracket s_i\rrbracket \xrightarrow{\llbracket \mathrm{op}\rrbracket} \llbracket s\rrbracket$$

(When $|\mathbb{V}_s| \geq \lambda$, there are less than $\lambda$ different variables that actually appear in $t$, and so we can find a smaller set of sorts and variables for which to define as above.)

A $\Sigma$-*homomorphism* $h : A \to B$ between $\Sigma$-algebras $A$, $B$ is an $\mathcal{S}$-indexed family of functions $h_s : A\llbracket s\rrbracket \to B\llbracket s\rrbracket$ such that, for every operation symbol $\mathrm{op} : \prod_{i\in I} s_i \to s$ in $\Sigma$:

$$\begin{array}{ccc}
\prod_{i\in I} A\llbracket s_i\rrbracket & \xrightarrow{\prod_{i\in I} h_{s_i}} & \prod_{i\in I} B\llbracket s_i\rrbracket \\
{\scriptstyle A\llbracket \mathrm{op}\rrbracket}\downarrow & = & \downarrow{\scriptstyle B\llbracket \mathrm{op}\rrbracket} \\
A\llbracket s\rrbracket & \xrightarrow[h_s]{} & B\llbracket s\rrbracket
\end{array}$$

We denote the category of $\Sigma$-algebras in $C$ and their homomorphisms by $\Sigma\mathrm{-}\mathbf{Mod}(C)$.

# Some General Semantic Techniques for Term and Type Recursion, with an Application to the Correctness of Automatic Differentiation

ANONYMOUS AUTHOR(S)

In this note, we extend our correctness proofs of automatic differentiation to apply to languages with term and type recursion. In order to do so, we first develop a broad class of models of recursive types, arising from any Grothendieck quasitopos and a chosen full (internal) sub-cpo of its subobject classifier. This construction specializes to give rise to quasi-Borel predomains $\omega\mathbf{Qbs}$ and diffeological predomains $\omega\mathbf{Diff}$. Next, we develop a categorical treatment of logical relations for recursive types. That is, we extend sconing and subsconing techniques to bilimit compact categories and bilimit compact expansions. This should be a categorical reformulation and generalization of known techniques as formulated by [Pitts 1996]. Finally, once this machinery is in place, correctness of AD techniques for languages with term and type recursion falls out straightforwardly by following the same recipe as used for languages with iteration, but by replacing $\mathbf{Diff}$ with $\omega\mathbf{Diff}$ and $\mathbf{Sh}(\mathcal{O}_{\mathbb{R}})$ with $\mathbf{Sh}_{\omega\mathbf{CPO}}(\mathcal{O}_{\mathbb{R}})$.

Additional Key Words and Phrases: automatic differentiation, recursion, correctness, logical relations, recursive types

Contents


| | | |
|---|---|---|
| Abstract | | 1 |
| Contents | | 1 |
| 1 | Introduction | 1 |
| 2 | Models of Essentially Algebraic Theories | 2 |
| 3 | Bilimit Compact Categories | 5 |
| 4 | A Partiality Monad on Sheaves | 7 |
| 4.1 | An Aside: the "Wrong" Partiality Monad | 8 |
| 4.2 | The "Right" Partiality Monad – Some Intuition | 9 |
| 4.3 | The "Right" Partiality Monad – Construction | 10 |
| 5 | Axiomatic domain theory in $\mathbf{SSh}_{\omega\mathbf{CPO}}(\mathcal{C},\mathcal{J},\mathcal{K})$ | 15 |
| 5.1 | Domain structures | 15 |
| 5.2 | Axiomatic Structure | 15 |
| 5.3 | Axioms and Derived Structure | 18 |
| 6 | Two Orthogonal Factorization Systems on $\mathbf{SSh}_{\omega\mathbf{CPO}}(\mathcal{C},\mathcal{J},\mathcal{K})$ | 33 |
| 7 | Bilimit Compact Sconing | 42 |
| 8 | Correctness of AD for Recursive Types | 53 |
| References | | 57 |


## 1 INTRODUCTION

General recursion, a.k.a. term recursion, is a core programming technique used in functional languages, and, increasingly in mainstream languages to give concise formulations of algorithms. Recursion can also be applied at the type level. This is useful for modelling infinite, potentially lazy, data structures, such as trees and streams. Such recursive techniques could be of use in machine

2018. 2475-1421/2018/1-ART1 $15.00
https://doi.org/

learning and scientific computing applications. However, they currently cannot be used as such applications require that we perform automatic differentiation (AD) on our code. AD techniques for term and type recursion currently do not exist. In this note, we develop such techniques and prove their correctness.

We have elegant correctness proofs of AD, relying on categorical sconing arguments, embodying a suitably general notion of logical relation. A good theory of sconing for languages with recursion, and particularly recursive types, is missing. Therefore, we develop this.

Next, we give a general construction construction of models of languages with recursion in categories of $\omega$-cpos internal to (separated) sheaf categories. Particular examples are quasi-Borel predomains that [Vákár et al. 2019] successfully used to solve open questions in domain theory for probability, and diffeological predomains that we will use in this note to model automatic differentiation on languages with recursion. A key ingredient in this development is the definition of a suitably general partiality monad on such categories. We hope this construction may prove useful in future for developing models of language with recursive types and particular computational effects. For example, they immediately specialize to give a nominal domain theory and we imagine they are useful to extend any other separated sheaf models of programming languages to encompass term and type recursion.

With these ingredients in place, an elegant proof of correctness of automatic differentiation for languages with recursion rolls out, following our previous develops in this area.

We imagine our general development of (sub)sconing techniques for recursive types can give an attractive alternative to existing logical relations techniques for such settings. We hope they will prove useful in future applications when analyzing languages with recursive features.

Concretely, our core contributions are the following constructions:

- for any Grothendieck quasitopos $\mathbf{SSh}(\mathcal{C}, \mathcal{J}, \mathcal{K})$, we consider the $\boldsymbol{\omega}\mathbf{CPO}$-enriched category $\mathbf{SSh}_{\omega\mathbf{CPO}}(\mathcal{C}, \mathcal{J}, \mathcal{K})$ of internal $\omega$-cpos and show that it is cartesian closed and locally presentable (hence complete and cocomplete);
- in case we fix a full internal sub-$\omega$-cpo $\mathfrak{M}$ of its subobject classifier $\Omega$, whose elements will serve as domains of partial functions, we construct an axiomatic domain theory in $\mathbf{SSh}_{\omega\mathbf{CPO}}(\mathcal{C}, \mathcal{J}, \mathcal{K})$, generalizing the constructions of $\omega\mathbf{Qbs}$ and $\omega\mathbf{Diff}$;
- a partial map classifier which is a commutative strong locally continuous partiality monad on $\mathbf{SSh}_{\omega\mathbf{CPO}}(\mathcal{C}, \mathcal{J}, \mathcal{K})$;
- a proof that the induced category of partial maps gives a bilimit compact expansion $\mathbf{SSh}(\mathcal{C}, \mathcal{J}, \mathcal{K}) \hookrightarrow \mathbf{SSh}(\mathcal{C}, \mathcal{J}, \mathcal{K})_\perp$ which has sufficient structure to interpret (fine-grain) FPC;
- a proof that any $\boldsymbol{\omega}\mathbf{CPO}$-enriched reflective subcategory of a bilimit compact expansion (a category with sufficient structure to interpret recursive types), is itself a bilimit compact expansion;
- a general sconing and subsconing construction for bilimit compact expansions, giving a categorical account of logical relations for recursive types;
- two orthogonal factorization systems on $\mathbf{SSh}(\mathcal{C}, \mathcal{J}, \mathcal{K})$ that are suitable for subsconing for recursive types;
- once all of this general purpose machinery is in place, a straightforward correctness proof of forward-mode Automatic Differentiation on fine-grain real FPC.

## 2 MODELS OF ESSENTIALLY ALGEBRAIC THEORIES

We recall some basic facts about essentially algebraic theories and locally presentable categories. Let us fix some regular cardinal $\kappa$. In the following, suppose that we fix some $\kappa$-essentially algebraic theory $\mathbb{T}$. We identify this theory with its initial model, which is a $\kappa$-limit sketch. Given some

category $C$ with limits of size $\kappa$, we will denote by $\mathbb{T}-\mathbf{Mod}(C)$ the full subcategory of the functor $[\mathbb{T}, C]$ on the $\kappa$-limit preserving functors. Observe that we have an obvious forgetful functor $|\cdot| : \mathbb{T}-\mathbf{Mod}(C) \to C$ induced by evaluating a model at the terminal object of $\mathbb{T}$. The following is standard.

Proposition 2.1. *$|\cdot| : \mathbb{T}-\mathbf{Mod}(C) \to C$ creates all limits that exist in $C$. As a consequence, $\mathbb{T}-\mathbf{Mod}(C)$ has limits of all shapes that exist in $C$.*

The following is a straightforward consequence.

Proposition 2.2. *Suppose that $i : \mathcal{D} \hookrightarrow \mathcal{E}$ is a full embedding, such that $\mathcal{D}, \mathcal{E}$ have small limits and $i$ preserves limits. Then, $\mathbb{T}-\mathbf{Mod}(\mathcal{D})$ and $\mathbb{T}-\mathbf{Mod}(\mathcal{E})$ have small limits and $-; i : [\mathbb{T}, \mathcal{D}] \to [\mathbb{T}, \mathcal{E}]$ restricts to a full embedding $\mathbb{T}-\mathbf{Mod}(\mathcal{D}) \hookrightarrow \mathbb{T}-\mathbf{Mod}(\mathcal{E})$ which preserves them.*

Now, suppose that $\lambda$ is some other regular cardinal such that $\kappa \leq \lambda$.

Proposition 2.3. *If $C$ is locally $\lambda$-presentable, then so is $\mathbb{T}-\mathbf{Mod}(C)$.*

This gives us the following corollary, as long as we assume (weak) Vopěnka's principle.

Corollary 2.4. *For $\mathcal{D}, \mathcal{E}$, locally $\lambda$-presentable, and $\mathcal{D}$ a full subcategory of $\mathcal{E}$ that is closed under limits, $\mathbb{T}-\mathbf{Mod}(\mathcal{D})$ is a full reflective subcategory of $\mathbb{T}-\mathbf{Mod}(\mathcal{E})$.*

Proof. We have seen that $\mathbb{T}-\mathbf{Mod}(\mathcal{D})$ is a full subcategory of $\mathbb{T}-\mathbf{Mod}(\mathcal{E})$ that is closed under limits. By theorem 6.22 of [Adámek et al. 1994], the corollary now follows. □

Some particularly well-behaved theories $\mathbb{T}$ (such as commutative algebraic theories, the theory $\omega$cpo of $\omega$-cpos, or the presentations of Grothendieck quasi-toposes) allow us to endow homsets with a $\mathbb{T}$-model structure. We now turn our attention to such theories.

Proposition 2.5. *Let $i : \mathcal{D} \hookrightarrow \mathcal{E}$ as before. Suppose that $\mathbb{T}-\mathbf{Mod}(\mathcal{D})$, $\mathbb{T}-\mathbf{Mod}(\mathcal{E})$ are $\mathbb{T}-\mathbf{Mod}(\mathbf{Set})$-enriched and cotensored over $\mathbb{T}-\mathbf{Mod}(\mathbf{Set})$, such that $\mathbb{T}-\mathbf{Mod}(i) : \mathbb{T}-\mathbf{Mod}(\mathcal{D}) \hookrightarrow \mathbb{T}-\mathbf{Mod}(\mathcal{E})$ enriches and preserves cotensors. Then, then $\mathbb{T}-\mathbf{Mod}(\mathcal{D})$ is a reflective subcategory of $\mathbb{T}-\mathbf{Mod}(\mathcal{E})$ in the $\mathbb{T}-\mathbf{Mod}(\mathbf{Set})$-enriched sense.*

Proof. By proposition 6.7.6 in [Borceux 1994], we know that an enriched functor has an enriched left adjoint iff it preserves cotensors. □

Next, we turn our attention to models in Grothendieck quasitoposes.

Proposition 2.6. *For any category $C$, we have an isomorphism of categories*

$$\mathbb{T}-\mathbf{Mod}([C^{op}, \mathbf{Set}]) \cong [C^{op}, \mathbb{T}-\mathbf{Mod}(\mathbf{Set})].$$

*That is, internal $\mathbb{T}$-models in presheaf categories are precisely presheaves valued in $\mathbb{T}$-models. Further, if we equip $C$ with Grothendieck topologies $\mathcal{J} \subseteq \mathcal{K}$, this isomorphism restricts to one between $\mathbb{T}$-models in $\mathcal{J}$-sheaves and presheaves valued in $\mathbb{T}-\mathbf{Mod}(\mathbf{Set})$ which are $\mathcal{J}$-sheaves*

$$\mathbb{T}-\mathbf{Mod}(\mathbf{Sh}(C, \mathcal{J})) \cong \mathbf{Sh}_{\mathbb{T}-\mathbf{Mod}(\mathbf{Set})}(C, \mathcal{J})$$

*and to one between $\mathbb{T}$-models in $\mathcal{K}$-separated $\mathcal{J}$-sheaves and presheaves valued in $\mathbb{T}-\mathbf{Mod}(\mathbf{Set})$ which are $\mathcal{J}$-sheaves and $\mathcal{K}$-separated*

$$\mathbb{T}-\mathbf{Mod}(\mathbf{SSh}(C, \mathcal{J}, \mathcal{K})) \cong \mathbf{Sh}_{\mathbb{T}-\mathbf{Mod}(\mathbf{Set})}(C, \mathcal{J}, \mathcal{K}).$$

*Finally, $\mathbb{T}-\mathbf{Mod}(\mathbf{SSh}(C, \mathcal{J}, \mathcal{K})) \hookrightarrow \mathbb{T}-\mathbf{Mod}(\mathbf{Sh}(C, \mathcal{J})) \hookrightarrow \mathbb{T}-\mathbf{Mod}([C^{op}, \mathbf{Set}])$ are reflective embeddings.*

Proof. The claim about presheaves follows immediately seeing that limits are computed pointwise in presheaf categories, while models are defined as limit-preserving functors. The claims about sheaves and separated sheaves follow once we note that $\mathbf{SSh}(C, \mathcal{J}, \mathcal{K}) \hookrightarrow \mathbf{Sh}(C, \mathcal{J})$ and $\mathbf{Sh}(C, \mathcal{J}) \hookrightarrow [C^{op}, \mathbf{Set}]$ preserve limits (as they are reflective subcategories) [Garner and Lack 2012]. The claim about reflective embeddings follows form corollary 2.4. □

In this paper, we will be particularly interested in $\omega$-cpos internal to Grothendieck quasitoposes. We write $\boldsymbol{\omega}\mathbf{CPO} \stackrel{\text{def}}{=} \omega\text{cpo}-\mathbf{Mod}(\mathbf{Set})$ for the category of $\omega$-cpos (in $\mathbf{Set}$). Given a Grothendieck quasitopos $\mathcal{E}$, we write $\Gamma$ for the global sections functor $\Gamma = \mathcal{E}(1, -) : \mathcal{E} \to \mathbf{Set}$. Recall that this always has a left adjoint $\Delta$, called the *locally constant (separated) sheaf functor*. Recall that a Grothendieck quasitopos is called *locally connected* if $\Delta$ has a further left adjoint $\Pi_0$ called the *connected components functor*. $\Delta \dashv \Gamma$.

Proposition 2.7. *The category $\omega\text{cpo}-\mathbf{Mod}(\mathcal{E})$ of internal $\omega$-cpos in a Grothendieck quasitopos $\mathcal{E}$ is locally presentable, cartesian closed and $\boldsymbol{\omega}\mathbf{CPO}$-enriched. Moreover, for any subquasitopos $\mathcal{D}$, $\omega\text{cpo}-\mathbf{Mod}(\mathcal{D})$ is a full reflective subcategory of $\omega\text{cpo}-\mathbf{Mod}(\mathcal{E})$ in the enriched sense, if we assume that $\mathcal{D}, \mathcal{E}$ are locally connected. The same is true is we replace $\omega$-cpos and $\omega$-continuous functions with $\omega$-cpos with a bottom element and strict $\omega$-continuous functions.*

Proof. Grothendieck quasitoposes $\mathcal{E}$ are locally presentable [Garner and Lack 2012] and therefore the category $\omega\text{cpo}-\mathbf{Mod}(\mathcal{E})$ of models of the essentially algebraic theory $\omega$cpo is also locally presentable.

WLOG assume that $\mathcal{E} = \mathbf{SSh}(C, \mathcal{J}, \mathcal{K})$ is the category of $\mathcal{K}$-separated $\mathcal{J}$-sheaves on $C$. Then, by the above, $\omega\text{cpo}-\mathbf{Mod}(\mathbf{SSh}(C, \mathcal{J}, \mathcal{K})) \cong \mathbf{Sh}_{\omega\text{cpo}-\mathbf{Mod}(\mathbf{Set})}(C, \mathcal{J}, \mathcal{K})$. Therefore, $\mathbf{Sh}_{\omega\text{cpo}-\mathbf{Mod}(\mathbf{Set})}(C, \mathcal{J}, \mathcal{K})(X, Y)$ consists of the elements of $\mathbf{Sh}(C, \mathcal{J}, \mathcal{K})(|X|, |Y|)$ whose components are $\omega$-continuous. Therefore (working in the internal language), we can define $X \Rightarrow Y$ as the following subobject of the internal hom $|X| \Rightarrow |Y|$

$$|X \Rightarrow Y| \stackrel{\text{def}}{=} \left\{ f : |X| \Rightarrow |Y| \mid \forall a : C^{\omega}_X . f(\vee_X a) = \vee_Y(a; f) \right\},$$

where we write $C^{\omega}_X$ for the subobject of $\omega$-chains in $X^{\mathbb{N}}$. Observe that $|X \Rightarrow Y|$ naturally is an internal poset with order $\leq_{X \Rightarrow Y}$ defined as the following subobject of $|X \Rightarrow Y| \times |X \Rightarrow Y|$:

$$\leq_{X \Rightarrow Y} \stackrel{\text{def}}{=} \{(f, g) \mid \forall x : X. f(x) \leq_Y g(x)\} .$$

Then, we can next define $\vee_{X \Rightarrow Y} : C^{\omega}_{X \Rightarrow Y} \to X \Rightarrow Y$ as

$$\vee_{X \Rightarrow Y}(f) = \lambda x : X. \vee_Y (\lambda n : \mathbb{N}. f(n)(x))$$

to turn $X \Rightarrow Y$ into an internal $\omega$-cpo.

Finally, we show that the adjunction $\omega\text{cpo}-\mathbf{Mod}(a) \dashv \omega\text{cpo}-\mathbf{Mod}(i) : \omega\text{cpo}-\mathbf{Mod}(\mathcal{D}) \to \omega\text{cpo}-\mathbf{Mod}(\mathcal{E})$ enriches over $\boldsymbol{\omega}\mathbf{CPO}$, where we write $a \dashv i$ for the reflection of $\mathcal{D}$ in $\mathcal{E}$. Let us write $\Delta \dashv \mathcal{E}(1, -)$. Then, $\Delta; a \dashv \mathcal{D}(1, -)$. We have assumed that $\Delta$ and $\Delta; a$ have further left adjoints $\Pi^{\mathcal{E}}_0$ and $\Pi^{\mathcal{D}}_0$. Therefore, $\Delta$ and $\Delta; a$ preserve limits so they lift to give $\boldsymbol{\omega}\mathbf{CPO}$-enriched functors $\omega\text{cpo}-\mathbf{Mod}(\Delta) : \boldsymbol{\omega}\mathbf{CPO} \to \omega\text{cpo}-\mathbf{Mod}(\mathcal{E})$ and $\omega\text{cpo}-\mathbf{Mod}(\Delta; a) : \boldsymbol{\omega}\mathbf{CPO} \to \omega\text{cpo}-\mathbf{Mod}(\mathcal{D})$. We can easily check that they give $\boldsymbol{\omega}\mathbf{CPO}$-enriched left adjoints to $\omega\text{cpo}-\mathbf{Mod}(\mathcal{E})(1, -)$ and $\omega\text{cpo}-\mathbf{Mod}(\mathcal{D})(1, -)$, respectively. Then, we can note that

$$\begin{aligned} \omega\text{cpo}-\mathbf{Mod}(E)(E, \omega\text{cpo}-\mathbf{Mod}(\Delta)X \Rightarrow E') &\cong \omega\text{cpo}-\mathbf{Mod}(E)(\omega\text{cpo}-\mathbf{Mod}(\Delta)X, E \Rightarrow E') \\ &\cong \boldsymbol{\omega}\mathbf{CPO}(X, \omega\text{cpo}-\mathbf{Mod}(E)(1, E \Rightarrow E')) \\ &\cong \boldsymbol{\omega}\mathbf{CPO}(X, \omega\text{cpo}-\mathbf{Mod}(E)(E, E')), \end{aligned}$$

so $\omega$cpo$-$**Mod**$(E)$ is cotensored over $\boldsymbol{\omega}$**CPO** with cotensor $X \pitchfork E \stackrel{\text{def}}{=} \omega\text{cpo}-\mathbf{Mod}(\Delta)X \Rightarrow E$. For similar reasons, $\omega$cpo$-$**Mod**$(D)$ is cotensored over $\boldsymbol{\omega}$**CPO** with cotensor $X \pitchfork D \stackrel{\text{def}}{=} \omega\text{cpo}-\mathbf{Mod}(\Delta;a)X \Rightarrow D$. Observe that $\omega\text{cpo}-\mathbf{Mod}(i)(\omega\text{cpo}-\mathbf{Mod}(\Delta;a)(X) \Rightarrow D) \cong \omega\text{cpo}-\mathbf{Mod}(\Delta)(X) \Rightarrow iD$ to see that $\omega$cpo$-$**Mod**$(i)$ preserves cotensors. The claim now follows from proposition 2.7. □

It is well-known (see theorem C1.5.9 in [Johnstone 2002]) that a topos $\mathbf{Sh}(O_X)$ of sheaves on a locally connected space (like an open subset of $\mathbb{R}^n$) $X$ is locally connected, meaning that the previous theorem applies. Moreover, any presheaf topos is locally connected as

$$[C^{op}, \mathbf{Set}](X, \Delta S) \cong \mathbf{Set}(\mathrm{colim} X, S).$$

Next, any subquasitopos $a \dashv i : \mathcal{D} \hookrightarrow \mathcal{E}$ of a locally connected quasitopos $\mathcal{E}$ is locally connected (with $\Pi_0^{\mathcal{D}} = i; \Pi_0^{\mathcal{E}}$) if $\Delta = \Delta; a; i$:

$$\mathcal{D}(D, a\Delta S) \cong \mathcal{E}(iD, ia\Delta S) \cong \mathcal{E}(iD, \Delta S) \cong \mathbf{Set}(\Pi_0(iD), S).$$

This is, in particular, the case for the topos of sheaves $\mathbf{Sh}(\mathbf{Open}, J)$ on the category **Open** of open subsets of Euclidean spaces and smooth functions with their usual Grothendieck topology generated by open covers. Another example is that a topos of concrete $\mathcal{J}$ sheaves $\mathbf{SSh}(C, \mathcal{J}, \mathcal{K})$ is locally connected if $\mathbf{Sh}(C, \mathcal{J})$ is. As a consequence, the category $\mathbf{Diff} \hookrightarrow \mathbf{Sh}(\mathbf{Open}, J)$ of diffeological spaces is also locally connected[1]. (In this case, $\Pi_0 X = |X|/\sim$ where $x \sim x'$ if there exists a smooth path $\gamma \in \mathcal{P}_X^{\mathbb{R}}$ connecting $x$ and $x'$.) Because of this, the previous theorem applies to **Diff** and $\mathbf{Sh}(O^k_{\mathbb{R}})$.

## 3 BILIMIT COMPACT CATEGORIES

We recall some basic machinery for solving recursive domain equations[Levy 2012]. Recall that an embedding-projection-pair (ep-pair) $u : A \rightleftharpoons B$ in an $\boldsymbol{\omega}$**CPO**-enriched category $\mathcal{B}$ is a pair consisting of a $\mathcal{B}$-morphism $u^{\mathrm{e}} : A \to B$, the *embedding*, and a $\mathcal{B}$-morphism $u^{\mathrm{p}} : B \to A$, the *projection*, such that $p; e \leq \mathrm{id}$ and $e; p = \mathrm{id}$. An *embedding* $u : A \hookrightarrow B$ is the embedding part of some ep-pair $A \rightleftharpoons B$.

An *$\omega$-chain of ep-pairs* $((A_n)_{n\in\mathbb{N}}, (a_n)_{n\in\mathbb{N}})$ in $\mathcal{B}$ consists of a countable sequence of objects $A_n$ and a countable sequence of ep-pairs $a_n : A_n \rightleftharpoons A_{n+1}$. A *bilimit* $(D, d)$ of such an $\omega$-chain consists of an object $D$ and a countable sequence of ep-pairs $d_n : A_n \rightleftharpoons D$ such that, for all $n \in \mathbb{N}$, $a_n; d_{n+1} = d_n$, and $\bigvee_{n\in\mathbb{N}} d_n^{\mathrm{p}}; d_n^{\mathrm{e}} = \mathrm{id}_D$. The celebrated *limit-colimit coincidence* [Smyth and Plotkin 1982] states that the bilimit structure is equivalent to a colimit structure $(D, d^{\mathrm{e}})$ for $(*, (A_n))\left(a_n^{\mathrm{e}}\right)$, in which case $d_n^{\mathrm{p}}$ are uniquely determined, and similarly equivalent to a limit structure $(*, D)\, d^{\mathrm{p}}$ for $(*, (A_n))\left(a_n^{\mathrm{p}}\right)$, in which case $d_n^{\mathrm{e}}$ are uniquely determined.

A *zero object* is an object that is both initial and terminal. An *ep-zero object* in an $\boldsymbol{\omega}$**CPO**-category is a zero object such that every morphism into it is a projection and every morphism out of it is an embedding.

A *bilimit compact category* is an $\boldsymbol{\omega}$**CPO**-category $\mathcal{B}$ with an ep-zero and ep-pair $\omega$-chain bilimits. When $\mathcal{A}, \mathcal{B}$ are bilimit compact, every locally continuous, mixed-variance functor $F : \mathcal{A}^{\mathrm{op}} \times \mathcal{B}^{\mathrm{op}} \times \mathcal{A} \times \mathcal{B} \to \mathcal{B}$ has a parameterised solution to the recursive equation $\mathsf{roll} : F(A, X, A', X) \xrightarrow{\cong} X$, for every $A, A'$ in $\mathcal{A}$, qua the bilimit $\left(\mu B.F(A, B, A', B), d_{F,A,A'}\right)$ of

$$\mathbb{0} \rightleftharpoons F(A, \mathbb{0}, A', \mathbb{0}) \xrightleftharpoons{F^{\mathrm{ep}}(A, \rightleftharpoons, A', \rightleftharpoons)} F(A, F(A, \mathbb{0}, A', \mathbb{0}), A', F(A, \mathbb{0}, A', \mathbb{0})) \rightleftharpoons \cdots \rightleftharpoons F^n(A, A') \rightleftharpoons \cdots$$

[1]Quasi-borel spaces are sadly not locally connected. There, the construction of $\mathbb{T}-\mathbf{Mod}(\Delta; a)$ is more subtle. $\Delta; a(|X|)$ has the measurable step functions as plots. We still need to complete under sups of $\omega$-chains to get $\mathbb{T}-\mathbf{Mod}(\Delta; a)(X)$ here.

The solution is minimal in the sense of Pitts [1996], and we denote the inverse to roll by unroll. The assignments $\mu B.F(A, B, A', B)$ extend to a mixed-variance functor $\mu B.F(-, B, -, B) : \mathcal{A}^{\mathrm{op}} \times \mathcal{A} \to \mathcal{B}$ by $\mu B.F(f, B, g, B) := \bigvee_n d_n^{\mathrm{p}}; F^n(f, g); d_n^{\mathrm{e}}$.

Finally, a *bilimit compact expansion* $J : \mathcal{C} \hookrightarrow \mathcal{B}$ is a triple consisting of an **$\omega$CPO**-category $\mathcal{C}$, a bilimit compact category $\mathcal{B}$; and an identity-on-objects, locally continuous, order reflecting functor $J : \mathcal{C} \to \mathcal{B}$ such that, for every ep-pair $\omega$-chains $(A, a)$, $(B, b)$ in $\mathcal{B}$, their bilimits $(D, d)$, $(E, e)$, and countable collection of $\mathcal{C}$-morphisms $(\alpha_n : A_n \to B_n)_{n\in\mathbb{N}}$ such that for all $n$:

$$a_n^{\mathrm{e}}; J\alpha_{n+1} = J\alpha_n; b_n^{\mathrm{e}}, \qquad a_n^{\mathrm{p}}; J\alpha_n = J\alpha_{n+1}; b_n^{\mathrm{p}}$$

(i.e., $J\alpha : (A, a^{\mathrm{e}}) \to (B, b^{\mathrm{e}})$ and $J\alpha : (A, a^{\mathrm{p}}) \to (B, b^{\mathrm{p}})$ are natural transformations), there is a $\mathcal{C}$-morphism $f : D \to E$ such that $Jf = \bigvee_n d_n^{\mathrm{p}}; \alpha_n; e_n^{\mathrm{e}}$. The motivation for this definition: given two bilimit compact expansions $I : \mathcal{D} \hookrightarrow \mathcal{A}$, $J : \mathcal{C} \hookrightarrow \mathcal{B}$, and two locally continuous functors

$$F : \mathcal{D}^{\mathrm{op}} \times \mathcal{C}^{\mathrm{op}} \times \mathcal{D} \times \mathcal{C} \to \mathcal{C} \quad G : \mathcal{A}^{\mathrm{op}} \times \mathcal{B}^{\mathrm{op}} \times \mathcal{A} \times \mathcal{B} \to \mathcal{B} \quad \text{s.t.} \quad I^{\mathrm{op}} \times J^{\mathrm{op}} \times I \times J; G = F; J$$

the functor $\mu B.G(-, B, -, B) : \mathcal{A}^{\mathrm{op}} \times \mathcal{A} \to \mathcal{B}$ restricts to $\mu B.G(J^{\mathrm{op}}-, B, J-, B) : \mathcal{D}^{\mathrm{op}} \times \mathcal{D} \to \mathcal{C}$. Bilimit compact expansions are closed under small products, opposites, and exponentiation with small categories [Levy 2012].

The following is new. In some ways it will be the crucial lemma of our development, as we invoke it in several different places.

Lemma 3.1. *Suppose we are given a commutative diagram (i.e. $J_{\mathcal{E}}; a' = a; J_{\mathcal{D}}$ and $i; J_{\mathcal{E}} = J_{\mathcal{D}}; i'$)*

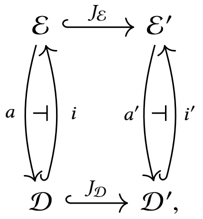

*where $J_{\mathcal{E}} : \mathcal{E} \hookrightarrow \mathcal{E}'$ is a bilimit compact expansion, $J_{\mathcal{D}} : \mathcal{D} \hookrightarrow \mathcal{D}'$ is a lluf (identity on objects) subcategory, and $a \dashv i : \mathcal{D} \leftrightarrows \mathcal{E}$ and $a' \dashv i' : \mathcal{D}' \leftrightarrows \mathcal{E}'$ are full reflective subcategories in the* **$\omega$CPO**-*enriched sense. Then $J_{\mathcal{D}} : \mathcal{D} \hookrightarrow \mathcal{D}'$ is a bilimit compact expansion.*

Proof. First, we show that $\mathcal{D}'$ is a bilimit compact category. $\mathcal{D}$ is a **$\omega$CPO**-category, by assumption. As $\mathcal{D}'$ is a full reflective subcategory, it contains the terminal object $\mathbb{1}$ of $\mathcal{E}$ which is also a terminal object in $\mathcal{D}$. That is, $a'\mathbb{1} = \mathbb{1}$. As $\mathbb{1}$ is also the initial object of $\mathcal{E}'$ and the left adjoint functor $a'$ preserves colimits, it follows that $a'\mathbb{1} = \mathbb{1}$ is also the initial object in $\mathcal{D}'$, so $\mathcal{D}'$ has a zero object. As $\mathcal{D}'$ is a full subcategory in the **$\omega$CPO**-enriched sense, it follows that any morphism into $\mathbb{1}$ is a projection and any morphism out of it is a embedding, hence $\mathcal{D}'$ is an ep-zero object. Next, we show that $\mathcal{D}'$ has bilimits of $\omega$-chains of ep-pairs. Consider an $\omega$-chain of ep-pairs $(a_n)_{n\in\mathbb{N}}$ in $\mathcal{D}'$. Then, $(i'a_n)_{n\in\mathbb{N}}$ is an $\omega$-chain of ep-pairs in $\mathcal{E}'$, by assumption of $i'$ being an enriched full subcategory. By assumption of $\mathcal{E}'$ being bilimit compact, $(i'a_n)_{n\in\mathbb{N}}$ has a bilimit $(B, (b_n)_{n\in\mathbb{N}})$ in $\mathcal{E}'$. As bilimits are preserved by any locally continuous functor, $a'$ preserves this bilimit: $(a'B, (a'b_n)_{n\in\mathbb{N}})$ is a bilimit for $(a'i'a_n)_{n\in\mathbb{N}} \cong (a_n)_{n\in\mathbb{N}}$. It follows that $\mathcal{D}'$ is bilimit compact.

Second, we show that $J_{\mathcal{D}} : \mathcal{D} \hookrightarrow \mathcal{D}'$ is a bilimit compact expansion. Observe that $\mathcal{D}$ is **$\omega$CPO**-enriched and is a **$\omega$CPO**-enriched lluf subcategory by assumption. Moreover, $J_{\mathcal{D}}$ is equal to $\mathcal{D}(D, D') \cong \mathcal{E}(iD, iD') \xrightarrow{J_{\mathcal{E}}} \mathcal{E}'(iD, iD') \cong \mathcal{D}'(D, D')$ on homsets, which we know to be an $\omega$-continuous order reflecting function. Let $(A, a)$, $(B, b)$ be ep-pair $\omega$-chains in $\mathcal{D}'$ with bilimits $(D, d)$,

$(E, e)$ and countable collection of $\mathcal{D}$-morphisms $(\alpha_n : A_n \to B_n)_{n\in\mathbb{N}}$ such that for all $n$:

$$a^{\mathrm{e}}_n; J_{\mathcal{D}}\alpha_{n+1} = J_{\mathcal{D}}\alpha_n; b^{\mathrm{e}}_n, \qquad a^{\mathrm{p}}_n; J_{\mathcal{D}}\alpha_n = J_{\mathcal{D}}\alpha_{n+1}; b^{\mathrm{p}}_n.$$

We show that there is some $\mathcal{D}$-morphism $f : A \to B$ such that $J_{\mathcal{D}} f = \bigvee_n d^{\mathrm{p}}_n; \alpha_n; e^{\mathrm{e}}_n$. Indeed, $(i'A, i'a)$, $(i'B, i'b)$ are ep-pair $\omega$-chains in $\mathcal{E}'$ with bilimits $(i'D, i'd)$, $(i'E, i'e)$, as $\mathcal{D}'$ is full subcategory of $\mathcal{E}'$ in the $\boldsymbol{\omega}$**CPO**-enriched sense, and we have $\mathcal{E}$-morphisms $(i\alpha_n : iA_n \to iB_n)_{n\in\mathbb{N}}$ such that for all $n$ (applying $i'$, and noting that $i; J_{\mathcal{E}} = J_{\mathcal{D}}; i'$ and $i$ is locally continuous and order reflecting):

$$i'a^{\mathrm{e}}_n; J_{\mathcal{E}} i\alpha_{n+1} = J_{\mathcal{E}} i\alpha_n; i'b^{\mathrm{e}}_n, \qquad i'a^{\mathrm{p}}_n; J_{\mathcal{E}} i\alpha_n = J_{\mathcal{E}} i\alpha_{n+1}; i'b^{\mathrm{p}}_n.$$

As, $J_{\mathcal{E}} : \mathcal{E} \to \mathcal{E}'$ is a bilimit compact expansion, there is some $\mathcal{E}$-morphism $g : iD \to iE$ such that $J_{\mathcal{E}} g = \bigvee_n i'd^{\mathrm{p}}_n; i\alpha_n; i'e^{\mathrm{e}}_n$. As $i$ is a full functor, it follows that $g = if$ for some $f : D \to E$ and as $i, i'$ are locally continuous order reflecting functors, we get that $J_{\mathcal{D}} f = \bigvee_n d^{\mathrm{p}}_n; \alpha_n; e^{\mathrm{e}}_n$. We conclude that $J_{\mathcal{D}} : \mathcal{D} \to \mathcal{D}'$ is a bilimit compact expansion. □

## 4 A PARTIALITY MONAD ON SHEAVES

We construct a partiality monad and domain theory on categories of $\omega$-cpos internal to separated sheaves on a bisite. The most general level of generality at which this development goes through is the following: consider Grothendieck quasitopos $\mathbf{SSh}(C, \mathcal{J}, \mathcal{K})$. Observe that the strong subobject classifier $\Omega$ is always an internal $\omega$-cpo with a bottom element $\bot$ and top element $\top$. Recall that $\Omega C$ contains precisely the $\mathcal{K}$-closed sieves on $C$. Let $\mathfrak{M}$ be any internal full sub-cpo of $\Omega$ containing both $\bot$ and $\top$. That is, it is an internal cpo in $\mathbf{SSh}(C, \mathcal{J}, \mathcal{K})$ whose elements are $\mathcal{K}$-closed sieves with the inclusion order. Then, this defines a canonical locally continuous commutative partiality monad $(-)_\bot$ on $\mathbf{SSh}_{\omega\mathbf{CPO}}(C, \mathcal{J}, \mathcal{K})$ such that its Kleisli adjunction gives a bilimit compact expansion that models FPC. In this development, to avoid excessive abstraction, we will focus on the more concrete case where $\mathfrak{M}$ merely consists of principal sieves (i.e. sieves of the form $\{g; m \mid g \in C\}$ where $m : U \rightarrowtail C \in C$ is some mono). Indeed, this case suffices to understand both quasi-Borel predomains and diffeological predomains.

However, we do not lose any generality in making this assumption. Indeed, all proofs still go through whenever we replace subobjects $m : U \hookrightarrow C$ with closed sieves $S$ and elements $\alpha \in FU$ with natural transformations $\beta \in \mathbf{Nat}(S, F)$ [2]. Alternatively, one could equivalently pass from $C$ to a larger site giving rise to the same quasitopos such that more closed sieves become principal. E.g. all $\mathcal{K}$-closed sieves become principal if we pass to the canonical site $\mathbf{Sh}(C, \mathcal{K})$ (where the covers are jointly epimorphic families): given a closed sieve $S \subseteq \mathbf{y}_C$ let $T \stackrel{\text{def}}{=} \left\{E \xrightarrow{g} D \in C \mid \forall E \xrightarrow{s} C, D \xrightarrow{s'} C \in S. s = g; s'\right\}$. Take some colimiting cocone $(F, \mu)$ of $T$. Then, $\mu$ is jointly epimorphic, hence a cover. Observe that $S$ defines another cocone on $T$, so we get a unique $u : F \to C$ which is a map of cocones, meaning that every $f \in S$ factors over $u$. Now, factor $u = e; m$ using the epi-mono factorization on the site. Then, $m^*S = \mu; e$ is also jointly epimorphic, hence a cover. As $S$ is closed, it follows that $m \in S$. As all of $S$ factors over $u$, it factors over $m$, so we see that $S$ is the principal sieve generated by $m$.

The more general case is not any different, conceptually, and might be of interest in quasitoposes where the natural site of definition does not have sufficiently many interesting suprema of $\omega$-chains of subobjects to define an interesting $\mathfrak{M}$ consisting merely of principal sieves.

[2] To be precise, when working at the level of generality of $\mathfrak{M}$ a full sub-cpo of $\Omega$, we define $F_\bot C \stackrel{\text{def}}{=} \{(S, \alpha) \mid S \in \mathfrak{M}C,\ \alpha \in \mathbf{Nat}(S, F)\}$. We then define $F_\bot(f)(S, \alpha, \stackrel{\text{def}}{=})(f^*S, \alpha(-; f))$, where we write $f^*S$ for the pullback sieve $\{g \mid g; f \in S\}$. Further, $(\mathrm{return}_F)_C(\alpha) \stackrel{\text{def}}{=} (\mathbf{y}_C, F(-)(\alpha))$ and $(S, \alpha)(\gg\!=_{F,G})_C\gamma \stackrel{\text{def}}{=} (S, \Delta_S; (\alpha \times \mathrm{id}_{\mathbf{y}_C}); \gamma)$, where we write $\Delta_S$ for the map $S \to S \times \mathbf{y}_C$ which sends $f \mapsto (f, f)$. None of the proofs are conceptually different.

### 4.1 An Aside: the "Wrong" Partiality Monad

Let us write $\omega$cpo for the limit sketch of $\omega$-cpos and $\omega$-continuous functions and $\omega\text{cpo}_\perp$ for the limit sketch of $\omega$-cpos with a bottom element and $\omega$-continuous strict functions. Observe that we have a continuous functor (embedding) from $\omega\text{cpo} \to \omega\text{cpo}_\perp$, which induces a functor $\omega\text{cpo}_\perp\text{–}\mathbf{Mod}(\mathcal{E}) \to \omega\text{cpo}\text{–}\mathbf{Mod}(\mathcal{E})$, by precomposition, for any category $\mathcal{E}$. In case $\mathcal{E} = [\mathcal{C}^{op}, \mathbf{Set}]$, this functor $[\mathcal{C}^{op}, \boldsymbol{\omega}\mathbf{CPO}_\perp] \to [\mathcal{C}^{op}, \boldsymbol{\omega}\mathbf{CPO}]$ corresponds to postcomposition with the usual forgetful functor $\boldsymbol{\omega}\mathbf{CPO}_\perp \to \boldsymbol{\omega}\mathbf{CPO}$. In particular, this has a left adjoint given by postcomposition with the usual lifting functor $\boldsymbol{\omega}\mathbf{CPO} \to \boldsymbol{\omega}\mathbf{CPO}_\perp$. Moreover, any category separated sheaves on $\mathcal{C}$, we have a (not necessarily commutative) square

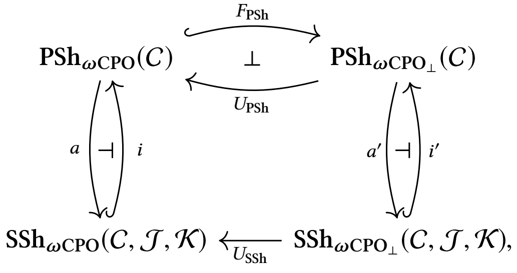


such that $i'; U_{\text{PSh}} = U_{\text{SSh}}; i$. A quick calculation shows that $F_{\text{SSh}} \stackrel{\text{def}}{=} i; F_{\text{PSh}}; a'$ gives a left adjoint to $U_{\text{SSh}}$. This induces a partiality monad $i; F_{\text{PSh}}; a'; U_{\text{SSh}} = i; F_{\text{PSh}}; a'; i'; U_{\text{PSh}}; a = i; F_{\text{PSh}}; U_{\text{PSh}}; a$ on $\mathbf{SSh}_{\omega\text{CPO}}(\mathcal{C}, \mathcal{J}, \mathcal{K})$. As usual, both of these adjunctions $F_{\text{SSh}} \dashv U_{\text{SSh}}$ and $F_{\text{PSh}} \dashv U_{\text{SSh}}$ are monadic, by Beck's monadicity theorem. Indeed, $F_{\text{PSh}} \dashv U_{\text{PSh}}$ inherits monadicity from the usual adjunction $\boldsymbol{\omega}\mathbf{CPO} \leftrightarrows \boldsymbol{\omega}\mathbf{CPO}_\perp$, as the monad and adjunction are taken pointwise. Moreover, $U_{\text{SSh}}$ clearly reflects isomorphisms. To see that it preserves coequalizers of reflexive pairs, note that $a' \dashv i'$ is monadic (as any reflective subcategory is), so $i'$ preserves coequalizers of reflexive pairs. $U_{\text{PSh}}$ does too as a monadic functor, as does $a$ as a left adjoint. Therefore, $U_{\text{SSh}} = i'; U_{\text{PSh}}; a$ preserves them as well, showing that $F_{\text{SSh}} \dashv U_{\text{SSh}}$ is monadic.

Observe that $|U_{\text{SSh}}(F_{\text{SSh}} G)| = |G| + 1$, where $|\cdot| : \mathbf{SSh}_{\omega\text{CPO}}(\mathcal{C}, \mathcal{J}, \mathcal{K}) \to \mathbf{SSh}(\mathcal{C}, \mathcal{J}, \mathcal{K})$ is the usual forgetful functor. Moreover, for a connected object $F$, we have that $\mathbf{SSh}_{\omega\text{CPO}}(\mathcal{C}, \mathcal{J}, \mathcal{K})(F, G_\perp) \cong \mathbf{SSh}_{\omega\text{CPO}}(\mathcal{C}, \mathcal{J}, \mathcal{K})(F, G)_\perp$. Suppose that $\mathcal{E} = \mathbf{SSh}_{\omega\text{CPO}}(\mathcal{C}, \mathcal{J}, \mathcal{K})$ is locally connected. Then, writing $G_\perp \stackrel{\text{def}}{=} U_{\text{SSh}}(F_{\text{SSh}} F)$, we have that $\mathcal{E}(F, G_\perp) = \mathcal{E}(\sum_{i \in \Pi_0 F} F_i, G_\perp) = \prod_{i \in \Pi_0 F} \mathcal{E}(F_i, G_\perp) = \prod_{i \in \Pi_0 F} \mathcal{E}(F_i, G)_\perp$, where $F \cong \sum_{i \in \Pi_0 F} F_i$ is the usual decomposition of $F$ into a coproduct of connected objects (which always exists in a locally connected quasitopos by taking the coproduct over the family given by the unit of the adjunction $\Pi_0 \dashv \Delta; a$).

We see that this definition of a partiality monad, in a locally connected quasitopos, models a notion of partiality in which total morphisms into $G_\perp$ are precisely partial morphisms into $G$ whose domain of definition is a union of connected components. This is far too limited a notion of partiality for our purposes. Indeed, when considering sheaves over topological spaces or over the category **Open**, we are interested in the larger class of partial functions whose domain of definition is an arbitrary open subset. It happens that the definitions above, do give correct notion of partiality for sheaves over the category **Sbs** of standard Borel spaces and in the category **Qbs** of quasi-Borel spaces (concrete sheaves over **Sbs**), as any measurable subset (rather than merely a connected component) of a standard Borel space can be classified by a measurable function into $1 + 1$. (Note that these quasitoposes are not locally connected, however.)

## 4.2 The "Right" Partiality Monad – Some Intuition

Therefore, we now turn towards a more general notion of partiality monad on categories of (separated) sheaves on $\mathcal{C}$. The prime intuition to have for sheaves is that they are supposed to generalize sheaves of functions on a space. That is, we can think of a sheaf $F$ as a generalized space, where $FC$ represents the set (or $\omega$-cpo) of functions from $C$ into the space $F$. As such, we would expect a partiality monad to produce a generalized space $F_\perp$, such that $F_\perp C$ represents the set of (or $\omega$-cpo) of *total* functions from $C$ into the space $F_\perp$, or equivalently, of *partial* functions from $C$ into the space $F$. A natural notion of partial function to $F$ can be obtained once we fix some class of subobjects $\mathfrak{M}C$ of $C$ in $\mathcal{C}$, which we judge suitable as serving as the domain of a well-behaved partial function from $C$ to $F$, on which it restricts to a total function to $F$. Then, we can define $F_\perp$ using a dependent sum

$$F_\perp C \stackrel{\text{def}}{=} \Sigma_{m:U \hookrightarrow C \in \mathfrak{M}C} FU,$$

which we can equip with the $\Sigma$-type (or product) order. If we choose $\mathfrak{M}C$ to consist of the connected components of $C$, presuming that we are working with a locally connected site, we should get the previous "wrong" partiality monad. We are free to make other choices for $\mathfrak{M}C$, however, that might be more suited for the application at hand.

For this definition of $F_\perp$ to be a well-behaved notion of partiality on $\mathbf{Sh}_{\omega\mathbf{CPO}}(\mathcal{C}, \mathcal{J})$, we need to impose some conditions on $\mathfrak{M}$. Indeed:

- if $F_\perp$ is to again be a presheaf on $\mathcal{C}$, we need to demand that $\mathfrak{M}$ is closed under (chosen) pullback;
- because of the natural order on $\mathfrak{M}C$, $F_\perp C$ is always a poset; if $F_\perp C$ is to be an $\omega$-cpo, however, we need to demand that $\mathfrak{M}C$ defines an $\omega$-cpo and that $F$ defines an $\omega$-continuous function on $\mathfrak{M}C$ as this lets us compute the sups as one would for a $\Sigma$-type of $\omega$-cpos (see [Palmgren and Stoltenberg-Hansen 1990]); one way of achieving this is to demand that $F$ is a sheaf with respect to a topology $\mathcal{J}$ for which every $\omega$-chain of elements of $\mathfrak{M}C$ covers its supremum;
- if $F_\perp$ is again to be a $\mathcal{J}$-sheaf, $\mathfrak{M}$ needs to be a $\mathcal{J}$-sheaf; this means that we can glue subobjects in $\mathfrak{M}$ along covers in $\mathcal{J}$;
- if $F_\perp C$ is to have a bottom element $\perp$, $\mathfrak{M}C$ needs to have a bottom element and the empty collection needs to be a $\mathcal{J}$-cover of this bottom element;
- if $F_\perp$ is to be a presheaf valued in $\boldsymbol{\omega}\mathbf{CPO}_\perp$, the pullback map $\mathfrak{M}f$ needs to be $\omega$-continuous and strict for any $f : C \to C' \in \mathcal{C}$;
- if $(-)_\perp$ is to define a (locally continuous) strong monad, we need to demand that $\mathfrak{M}$ contains all identities (hence, a top element) and is closed under composition, i.e. it needs to be a (lluf) subcategory of $\mathcal{C}$.

In case we additionally want $F_\perp$ to be a well-behaved notion of partiality on $\mathbf{SSh}_{\omega\mathbf{CPO}}(\mathcal{C}, \mathcal{J}, \mathcal{K})$, we need one further condition:

- $\mathfrak{M}$ is $\mathcal{K}$-separated.

One obvious class of examples to keep in mind for $\mathfrak{M}$ are a (composition closed) collection of subobjects, containing the top and bottom subobject, closed under pullbacks and sups of $\omega$-chains, such that covers in $\mathcal{J}$ are precisely the joins (unions) that exist in $\mathfrak{M}$. We could, for example, take $\mathcal{C} = \mathbf{Open}$ and $\mathfrak{M}$ inclusions of open subsets or $\mathcal{C} = \mathbf{Sbs}$ and $\mathfrak{M}$ inclusions of measurable subsets.

A different perspective on the construction of $F_\perp C$ is that we restrict $F$ to $\mathfrak{M}C \subseteq \mathcal{C}$, giving us an $\omega$-continuous presheaf of $\omega$-cpos on a $\omega$-cpo (i.e. a $\omega$-cpo-indexed $\omega$-cpo), and we apply the Grothendieck (category of elements) construction to this to get a single $\omega$-cpo (fibred over $\mathfrak{M}C$). We can further index this whole construction by the base point $C$ to pass from a $\mathcal{C}$-indexed, $\mathfrak{M}$-indexed $\omega$-cpo $F$ to a $\mathcal{C}$-indexed $\omega$-cpo $F_\perp$.

### 4.3 The "Right" Partiality Monad – Construction

Let us consider a category $\mathcal{C}$ together with a class $\mathfrak{M}$ of monos in $\mathcal{C}$ such that

- we have a chosen pullback $m^*U \xrightarrow{m^*f} U \in \mathcal{C}$, $m^*U \xrightarrow{f^*m} C' \in \mathfrak{M}$ for each $C' \xrightarrow{f} C \in \mathcal{C}$ and $U \xrightarrow{m} C \in \mathfrak{M}$;
- for each $C \in \mathcal{C}$, $\mathfrak{M}C$ forms an $\omega$-cpo with a bottom element and the embedding into the poset $\mathrm{Sub}(C)$ of all monos into $C$ in $\mathcal{C}$ is a full mono;
- the pullback map $\mathfrak{M}(f) \stackrel{\text{def}}{=} f^* : \mathfrak{M}C \to \mathfrak{M}C'$ is $\omega$-continuous and strict (preserves bottom elements) for each $C' \xrightarrow{f} C \in \mathcal{C}$.

In particular, $\mathfrak{M}$ then defines a functor $\mathcal{C}^{op} \to \boldsymbol{\omega}\mathbf{CPO}_\perp$.

Further suppose that $\mathcal{C}$ is equipped with a Grothendieck topology $\mathcal{J}$ such that for any $\omega$-chain $U_n \xrightarrow{m_n} C$ in $\mathfrak{M}C$ with supremum $U \xrightarrow{m} C$ in $\mathfrak{M}C$, the collection $(m_n \le m)_{n\in\mathbb{N}}$ is a cover of $U$, and such that the empty collection is a cover of the bottom element of $\mathfrak{M}C$.

We can then define a partiality monad $(-)_\perp$ on the category $\mathbf{Sh}_{\boldsymbol{\omega}\mathbf{CPO}}(\mathcal{C}, \mathcal{J})$ of internal $\omega$-cpos in $\mathcal{J}$-sheaves, by defining

$$F_\perp(C) \stackrel{\text{def}}{=} \left\{(m, \alpha) \mid U \xrightarrow{m} C \in \mathfrak{M}C, \alpha \in F(U)\right\}$$

with order

$$(m, \alpha) \le (m', \alpha') \stackrel{\text{def}}{=} m \le m' \wedge \alpha \le F(m \le m')(\alpha'),$$

where we note that $m \le m'$ consists by definition of a (unique) mono $n \in \mathcal{C}$ such that $n; m' = m$. For a morphism $C' \xrightarrow{f} C$, we can define

$$F_\perp(f)(m, \alpha) = (f^*m, F(m^*f)(\alpha)).$$

Lemma 4.1. *$F_\perp$ defines a functor from $\mathcal{C}^{op}$ to* $\boldsymbol{\omega}\mathbf{CPO}_\perp$.

Proof. Clearly, $F_\perp(C)$ forms a partial order.

First, observe that $\mathfrak{M}C$ has a bottom element $\perp : U_\perp \to C$ and by assumption the empty collection is a cover of $\perp$. Now, as $F$ is a sheaf, the empty collection has a unique amalgamation $\perp$, meaning that $F(U_\perp) = \{\perp\}$. (Indeed, any element of $F(U_\perp)$ is the amalgamation of the matching family induced on the empty cover, by definition of being a sheaf.) We show that $(\perp, \perp)$ is the bottom element of $F_\perp(C)$. Suppose that $(m, \alpha) \in F_\perp(C)$. Then $\perp \le m$ and $F(\perp \le m)(\alpha) \in F(U_\perp) = \{\perp\}$, so $F(\perp \le m)(\alpha) = \perp$. It follows that $(\perp, \perp) \le (m, \alpha)$.

Suppose we are given an $\omega$-chain $(m_n, \alpha_n)$ in $F_\perp(C)$ with $U_n \xrightarrow{m_n} C$. Then, $(F(m_{n'} \le m_n)(\alpha_n))_{n\in\mathbb{N}_{\ge n'}}$ defines an $\omega$-chain in $F(U_{n'})$. It therefore has a supremum $\alpha_{n'\omega}$. Now,

$$\begin{aligned} F(m_{n''} \le m_{n'})(\alpha_{n'\omega}) &= F(m_{n''} \le m_{n'})(\sup_n F(m_{n'} \le m_n)(\alpha_n)) \\ &= \sup_n F(m_{n''} \le m_{n'})(F(m_{n'} \le m_n)(\alpha_n)) \\ &= \sup_n F(m_{n''} \le m_n)(\alpha_n) \\ &= \alpha_{n''\omega}. \end{aligned}$$

That is, $(\alpha_{n\omega})_{n\in\mathbb{N}}$ forms a matching family for the cover $(m_n \le m_\omega)_{n\in\mathbb{N}}$ of $m_\omega \stackrel{\text{def}}{=} \sup_n m_n$. As $F$ is a sheaf, by assumption, it follows that $\alpha_{n\omega}$ has a unique amalgamation $\alpha_\omega$. We show that $(m_\omega, \alpha_\omega)$

forms a supremum for the $\omega$-chain $(m_n, \alpha_n)$. As $m_n \leq m_\omega$ by construction and

$$\begin{aligned}F(m_n \leq m_\omega)(\alpha_\omega) &= \alpha_{\omega n}\\ &= \sup_{n'\geq n} F(m_n \leq m_{n'})(\alpha_{n'})\\ &\geq \alpha_n,\end{aligned}$$

we have that $(m_n, \alpha_n) \leq (m_\omega, \alpha_\omega)$. Suppose that $(m, \alpha) \geq (m_n, \alpha_n)$ for all $n \geq 0$. Then $m \geq m_n$, so $m \geq \sup_n m_n = m_\omega$. Moreover, $\alpha_{n'} \leq F(m_{n'} \leq m)(\alpha)$, so, using monotonicity of $F$,

$$\begin{aligned}F(m_n \leq m_{n'})(\alpha_{n'}) &\leq F(m_n \leq m_{n'})(F(m_{n'} \leq m)(\alpha))\\ &= F(m_n \leq m)(\alpha)\\ &\leq F(m_n \leq m_\omega)(F(m_\omega \leq m)(\alpha)).\end{aligned}$$

Therefore, also

$$\begin{aligned}\alpha_{\omega n} &= \sup_{n'} F(m_n \leq m_{n'})(\alpha_{n'})\\ &\leq F(m_n \leq m_\omega)(F(m_\omega \leq m)(\alpha)).\end{aligned}$$

So, as gluing is monotone for a internal poset in sheaves like $F$,

$$\begin{aligned}\alpha_\omega &= \mathrm{glue}_n \alpha_{\omega n}\\ &\leq \mathrm{glue}_n F(m_n \leq m_\omega)(F(m_\omega \leq m)(\alpha))\\ &= F(m_\omega \leq m)(\alpha).\end{aligned}$$

We conclude that $(m_\omega, \alpha_\omega) \leq (m, \alpha)$, so $(m_\omega, \alpha_\omega)$ is the supremum of $((m_n, \alpha_n))_{n\in\mathbb{N}}$. To summarize, we can define

$$\sup_n (m_n, \alpha_n) \stackrel{\text{def}}{=} (\sup_n m_n, \mathrm{glue}_{n'}(\sup_n F(m_{n'} \leq m_n)(\alpha_n))).$$

Next, $F_\perp(f)$ is $\omega$-continuous and strict as $\mathfrak{M}(f)$ is by assumption while $F$ is $\omega$-continuous. Indeed,

$$\begin{aligned}F_\perp(\perp, \perp) &= (f^*\perp, F(\perp^* f)(\alpha))\\ &= (\perp, F(\perp^* f)(\alpha))\end{aligned}$$

(as $f^*$ is strict by assumption). Here, $F(\perp^* f)(\alpha) \in F(V_\perp) \cong \{\perp\}$, where $V_\perp$ is the domain of $\perp$, so $F(\perp^* f)(\alpha) = \perp$. Further

$$\begin{aligned}F_\perp(f)(\sup_n(m_n, \alpha_n)) &= (f^* m_\omega, F(m_\omega^* f)(\alpha_\omega))\\ &= (f^* \sup_n m_n, F(m_\omega^* f)(\mathrm{glue}_n \sup_{n'\geq n} F(m_n \leq m_{n'})(\alpha_{n'})))\\ &= (\sup_n f^* m_n, F(m_\omega^* f)(\mathrm{glue}_n \sup_{n'\geq n} F(m_n \leq m_{n'})(\alpha_{n'})))\\ &= (\sup_n f^* m_n, \mathrm{glue}_n F(m_n^* f)(\sup_{n'\geq n} F(m_n \leq m_{n'})(\alpha_{n'})))\\ &= (\sup_n f^* m_n, \mathrm{glue}_n \sup_{n'\geq n} F(m_n^* f)(F(m_n \leq m_{n'})(\alpha_{n'})))\\ &= (\sup_n f^* m_n, \mathrm{glue}_n \sup_{n'\geq n} F(f^* m_n \leq f^* m_{n'})(F(m_{n'}^* f)(\alpha_{n'})))\\ &= \sup_n(f^* m_n, F(m_n^* f)(\alpha_n))\\ &= \sup_n(F_\perp(f)(m_n, \alpha_n)).\end{aligned}$$

We see that $F_\perp(f)$ is $\omega$-continuous.

Finally, $F_\perp$ is automatically a functor as $F$ and our chosen pullback are both functors.

□

Now, let us further assume that $\mathfrak{M} \in \mathbf{Sh}_{\omega\text{CPO}}(C, \mathcal{J})$.

Lemma 4.2. *$F_\perp$ is an internal $\omega$-cpo in $\mathbf{Sh}(C, \mathcal{J})$.*

Proof. Let $(f_i : C_i \to C)_{i \in I}$ be a cover and $\left((U_i \xrightarrow{m^i} C_i, \alpha^i \in FU_i)\right)_{i \in I}$ a matching family for that cover. Then, in particular, $(m_i)_{i \in I}$ is a matching family for $\mathfrak{M}$ for this cover, so we get a unique amalgamation $U \xrightarrow{m} C \in \mathfrak{M}C$. Then, by the axioms of a Grothendieck topology (i.e. covers are closed under pullbacks), it follows that $\left(U_i \xrightarrow{m^* f_i} U\right)_{i \in I}$ is a cover of $U$. Now, observe that we have the following commutative diagram, where each of the eight faces is a pullback square

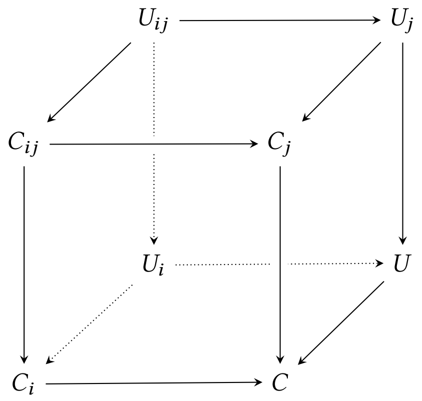


As $\left((U_i \xrightarrow{m^i} C_i, \alpha^i \in FU_i)\right)_{i \in I}$ is a matching family, we know that

$$\begin{aligned}((f_i^* f_j)^* m_i, F(m_i^*(f_i^* f_j))(\alpha_i)) &= F_\perp(f_i^* f_j)(m_i, \alpha_i) \\ &= F_\perp(f_j^* f_i)(m_j, \alpha_j) \\ &= ((f_j^* f_i)^* m_i, F(m_j^*(f_j^* f_i))(\alpha_j)).\end{aligned}$$

Therefore, it also follows that $F((m^* f_i) m^* f_j)(\alpha_i) = F((m^* f_j) m^* f_i)(\alpha_j)$. That is, $(\alpha_i)_{i \in I}$ is a matching family for $F$ with respect to the cover $\left(U_i \xrightarrow{m^* f_i} U\right)_{i \in I}$. It follows that we obtain a unique amalgamation $\alpha \in FU$. We have now constructed the unique amalgamation $(m, \alpha)$ of $\left((m_i, \alpha^i)\right)_{i \in I}$, so it follows that $F_\perp$ is a sheaf.

Moreover, as both $\mathfrak{M}$ and $F$ are internal posets in $\mathbf{Sh}(C, \mathcal{J})$, it follows that $F_\perp$ is an internal poset. Indeed, let $R \in \mathcal{J}C$ and let $(m, \alpha), (n, \beta) \in F_\perp C$ such that $F_\perp(f)(m, \alpha) \leq^{F_\perp} F_\perp(f)(n, \beta)$ for all $f \in R$. We show that also $(m, \alpha) \leq^{F_\perp} (n, \beta)$. Now,

$$(f^* m, F(m^* f)(\alpha)) = F_\perp(f)(m, \alpha) \leq^{F_\perp} F_\perp(f)(n, \beta) = (f^* n, F(n^* f)(\beta))$$

means that

$$f^* m \leq^{\mathfrak{M}} f^* n \text{ and } F(m^* f)(\alpha) \leq^F F(f^* m \leq f^* n)(F(n^* f)(\beta)) = F(m^* f)(F(m \leq n)(\beta))$$

As $\mathfrak{M}$ is an internal poset in $\mathbf{Sh}(C, \mathcal{J})$ and $R \in \mathcal{J}C$, it follows that $m \leq^{\mathfrak{M}} n$. As $F$ is an internal poset in $\mathbf{Sh}(C, \mathcal{J})$ and $m^* R \in \mathcal{J}$ (covers are closed under pullback), it follows that $\alpha \leq^F F(m \leq n)(\beta)$. We conclude that $(m, \alpha) \leq^{F_\perp} (n, \beta)$. It follows that $F_\perp$ is an internal poset and hence an internal $\omega$-cpo in $\mathbf{Sh}(C, \mathcal{J})$. □

Let us further assume that $\mathrm{id}_C \in \mathfrak{M}C$ and that $\mathfrak{M}$ is closed under composition (so $\mathfrak{M}$ is a full subcategory of $C$). Then, observe that we can define $\omega$-continuous natural transformations $\mathrm{return}_F : F \longrightarrow F_\perp$ by

$$\mathrm{return}_{FC}(\alpha) \stackrel{\mathrm{def}}{=} (\mathrm{id}_{FC}, \alpha)$$

and $\gg\!=_{F,G}$: $F_\perp \times G_\perp^F \longrightarrow G_\perp$ as follows. Given $(m, \alpha) \in F_\perp C$, where $U \xrightarrow{m} C \in \mathfrak{M}$, and $\gamma \in G_\perp^F C = \mathbf{Nat}(\mathbf{y}_C \times F, G_\perp)$, we observe that $\gamma_U(m, \alpha) \in G_\perp U$. Therefore, it is of the form $(n, \beta)$ for $V \xrightarrow{n} U \in \mathfrak{M}U$ and $\beta \in GV$. We can now define $(m, \alpha) \gg\!=_{F,G} \gamma \stackrel{\mathrm{def}}{=} (n; m, \beta)$. Put differently, $(m, \alpha) \gg\!=_{F,G} \gamma \stackrel{\mathrm{def}}{=} (\mathsf{fst}((m, \alpha); \gamma); m, \mathsf{snd}((m, \alpha); \gamma))$.

Lemma 4.3. *$(-)_\perp$ defines a locally continuous strong monad.*

Proof. First, we show $\omega$-continuity.
Clearly, $\mathrm{return}(\sup_n \alpha_n) = (\mathrm{id}, \sup_n \alpha_n) = \sup_n(\mathrm{id}, \alpha_n)$, so return is $\omega$-continuous.
Similarly,

$$\begin{aligned}(\sup_n(m_n, \alpha_n)) \gg\!= (\sup_k \gamma_k) &= (m_\omega, \alpha_\omega) \gg\!= (\sup_k \gamma_k)\\ &= (\mathsf{fst}((m_\omega, \alpha_\omega); (\sup_k \gamma_k)); m, \mathsf{snd}((m_\omega, \alpha_\omega); (\sup_k \gamma_k)))\\ &= \sup_k(\mathsf{fst}((m_\omega, \alpha_\omega); \gamma_k); m, \mathsf{snd}((m_\omega, \alpha_\omega); \gamma_k))\\ &= \sup_k(((m_\omega, \alpha_\omega); \gamma_k); m).\end{aligned}$$

Now,

$$\begin{aligned}(m_\omega, \alpha_\omega); \gamma &= (\mathrm{glue}_n m_n, \mathrm{glue}_n \alpha_{\omega n}); \gamma\\ &= (\mathrm{glue}_n(m_n, \alpha_{\omega n})); \gamma\\ &= \mathrm{glue}_n((m_n, \alpha_{\omega n}); \gamma)\\ &= \mathrm{glue}_n((m_n, \sup_{n' \geq n} F(m_{n'} \geq m_n)(\alpha_{n'})); \gamma)\\ &= \mathrm{glue}_n sup_{n' \geq n}((m_n, F(m_{n'} \geq m_n)(\alpha_{n'})); \gamma)\\ &= (\mathrm{glue}_n sup_{n' \geq n}((m_n, F(m_{n'} \geq m_n)(\alpha_{n'})))); \gamma\\ &= (\sup_n(m_n, \alpha_n)); \gamma\\ &= \sup_n((m_n, \alpha_n); \gamma)\end{aligned}$$

Second, we show that the strong monad laws hold:

$$\begin{aligned}\mathrm{return}(\alpha) \gg\!= \gamma &= (\mathsf{fst}((\mathrm{id}, \alpha); \gamma); \mathrm{id}, \mathsf{snd}((\mathrm{id}, \alpha); \gamma))\\ &= (\mathsf{fst}((\mathrm{id}, \alpha); \gamma), \mathsf{snd}((\mathrm{id}, \alpha); \gamma))\\ &= (\mathrm{id}, \alpha); \gamma\end{aligned}$$

and

$$\begin{aligned}(m, \alpha) \gg\!= \mathrm{return} &= (\mathsf{fst}((m, \alpha); \mathrm{return}); m, \mathsf{snd}((m, \alpha); \mathrm{return}))\\ &= (\mathrm{id}; m, \alpha)\\ &= (m, \alpha)\end{aligned}$$

and

$$\begin{aligned}((m,\alpha) \gg\!= \gamma) \gg\!= \delta &= (\mathsf{fst}((m,\alpha);\gamma);m, \mathsf{snd}((m,\alpha);\gamma)) \gg\!= \delta \\ &= (\mathsf{fst}((\mathsf{fst}((m,\alpha);\gamma);m, \mathsf{snd}((m,\alpha);\gamma));\delta); \mathsf{fst}((m,\alpha);\gamma);m, \mathsf{snd}((\mathsf{fst}((m,\alpha);\gamma);m, \mathsf{snd}((m,\alpha \\ &= (\mathsf{fst}(((\gamma(m,\alpha)) \gg\!= \delta)); m, \mathsf{snd}(((\gamma(m,\alpha)) \gg\!= \delta))) \\ &= (\mathsf{fst}((m,\alpha);(\lambda x.(\gamma x) \gg\!= \delta)); m, \mathsf{snd}((m,\alpha);(\lambda x.(\gamma x) \gg\!= \delta))) \\ &= (m,\alpha) \gg\!= (\lambda x.(\gamma x) \gg\!= \delta).\end{aligned}$$

□

Proposition 4.4. *$(-)_\perp$ is a commutative monad.*

Proof. Let $(m,\alpha),(n,\beta) \in F_\perp C$. We calculate

$$\begin{aligned}(m,\alpha) \gg\!= \lambda x.(n,\beta) \gg\!= \lambda y.\mathrm{return}(x,y) &= (m,\alpha) \gg\!= \lambda x.(n,\beta) \gg\!= \lambda y.(\mathrm{id},(x,y)) \\ &= (m,\alpha) \gg\!= \lambda x.(\mathrm{id};n,(x,\beta)) \\ &= (m,\alpha) \gg\!= \lambda x.(n,(x,\beta)) \\ &= (n^* m; n, (F(m^* n)\alpha, F(n^* m)\beta)) \\ &= (m^* n; m, (F(m^* n)\alpha, F(n^* m)\beta)) \\ &= (n,\beta) \gg\!= \lambda y.(m,(\alpha,y)) \\ &= (n,\beta) \gg\!= \lambda y.(\mathrm{id};m,(\alpha,y)) \\ &= (n,\beta) \gg\!= \lambda y.(m,\alpha) \gg\!= \lambda x.(\mathrm{id},(x,y)) \\ &= (n,\beta) \gg\!= \lambda y.(m,\alpha) \gg\!= \lambda x.\mathrm{return}(x,y).\end{aligned}$$

□

Corollary 4.5. *Let us fix some infinite regular cardinal $\lambda$. Let $C$ be a small category and let $\mathfrak{M}$ be a class of monos in $C$ such that*

- *for all $C$, the subset $\mathfrak{M}C$ is contains lubs of any size $\leq \lambda$ (including the empty lub);*
- *$\mathfrak{M}$ is closed under (chosen) pullbacks along arbitrary morphisms in $C$ and these pullbacks respect lubs of size $\leq \lambda$;*
- *$\mathfrak{M}$ contains all identities and is closed under composition;*

*where $\mathfrak{M}C$ is the subset of $\mathfrak{M}$ of monos into $C$. Then, if $\mathcal{J}$ is the smallest Grothendieck topology in which all sets of size $\leq \lambda$ of elements of $\mathfrak{M}C$ cover their lub, we get a locally continuous strong monad $(-)_\perp$ on $\mathbf{Sh}_{\omega\mathbf{CPO}}(C,\mathcal{J})$ where*

$$F_\perp C \stackrel{\text{def}}{=} \Sigma_{m:U\to C\in\mathfrak{M}C} FU.$$

*Note that this Grothendieck topology $\mathcal{J}$ is generated by a coverage (even a basis) $\mathcal{J}_{\mathfrak{M}}$ consisting exclusively of $\mathfrak{M}$. Later we will see that this leads to further desirable properties of $(-)_\perp$.*

Particular examples for $(C,\mathfrak{M},\lambda)$ are

- any frame $C = O_X$ of open subsets of a topological space (or locale), $\mathfrak{M}$ all morphisms in $C$, and $\lambda$ the cardinality of $\mathfrak{M}$;
- (any frame $C = O_X$ of open subsets of a topological space (or locale), $\mathfrak{M}$ the inclusions of connected components in $C$, and $\lambda$ the cardinality of $\mathfrak{M}$);
- the category $C = \mathbf{Open}$ of open subsets of Euclidean spaces and smooth functions between them, $\mathfrak{M}$ all smooth open embeddings, and $\lambda$ the cardinality of $\mathfrak{M}$;
- (the category $C = \mathbf{Open}$ of open subsets of Euclidean spaces and smooth functions between them, $\mathfrak{M}$ all smooth embeddings of connected components, and $\lambda$ the cardinality of $\mathfrak{M}$);

- the category $C$ = **Sbs** of standard Borel spaces and measurable functions, $\mathfrak{M}$ all measurable embeddings of measurable subsets, and $\lambda = \aleph_0$.

We will be less interested in the examples in parentheses.

Proposition 4.6. *Suppose that* $\mathfrak{M}$ *is* $\mathcal{K}$*-separated. Then,* $(-)_\perp$ *restricts to* $\mathbf{SSh}_{\omega\mathbf{CPO}}(C, \mathcal{J}, \mathcal{K})$*.*

Proof. Suppose that $F$ is $\mathcal{K}$-separated. We show that $F_\perp$ is as well.

Observe that for any $\mathcal{K}$-cover $R$ of $C$, for any matching family $((m_i, \alpha_i))_{i\in I}$ for $F_\perp$, any amalgamation $(m, \alpha)$ has the property that $m$ is an amalgamation for the $m_i$ is a matching family for $\mathfrak{M}$. Indeed, the first projection is a natural transformation $F_\perp \to \mathfrak{M}$. Now, as $\mathfrak{M}$ is $\mathcal{K}$-separated by assumption, there is at most one such $m : U \to C$. If there is no such $m$ for our particular matching family, we are done as this shows that our matching family does not have an amalgamation. Suppose that there is such an $m$ (at which point it is necessarily unique). Then $m^*R$ is a $\mathcal{K}$-cover of $U$ (by the axioms of a Grothendieck topology) and $\alpha_i$ is a matching family for $F$ with respect to $m^*R$ and $\alpha$ will be an amalgamation for it. This determines $\alpha$ uniquely as $F$ is $\mathcal{K}$-separated by assumption.

That means that amalgamations $(m, \alpha)$ for $((m_i, \alpha_i))_{i\in I}$ are unique, so $F_\perp$ is $\mathcal{K}$-separated. □

Corollary 4.7. *For a concrete site* $(C, \mathcal{J})$*,* $(-)_\perp$ *restricts to the category* $\mathbf{SSh}_{\omega\mathbf{CPO}}(C, \mathcal{J}, \mathcal{K})$ *of concrete sheaves, where* $\mathcal{K}$ *is the topology generated by jointly epimorphic families of maps which factor over* 1*.*

Proof. In this case, $\mathfrak{M}$ is $\mathcal{K}$-separated. Indeed, for a concrete site, a subset $m \in \mathfrak{M}(C)$ is uniquely determined by the elements it contains. The corollary now follows from proposition 4.6. □

Corollary 4.8. *The "good" partiality monads* $(-)_\perp$ *on* $\mathbf{Sh}_{\omega\mathbf{CPO}}(\mathbf{Open}, \text{open covers})$ *and* $\mathbf{Sh}_{\omega\mathbf{CPO}}(\mathbf{Sbs}, \text{countable}$ *restrict to partiality monads* $(-)_\perp$ *on diffeological predomains* $\omega\mathbf{Diff}$ *and quasi-Borel predomains* $\omega\mathbf{Qbs}$*.*

## 5 AXIOMATIC DOMAIN THEORY IN $\mathbf{SSh}_{\omega\mathbf{CPO}}(C, \mathcal{J}, \mathcal{K})$

In the following we suppose that $\mathbf{SSh}_{\omega\mathbf{CPO}}(C, \mathcal{J}, \mathcal{K})$ is equipped with a "good" partiality monad $(-)_\perp$.

### 5.1 Domain structures

Domain theory develops order-theoretic techniques for solving recursive domain equations. The theorems guaranteeing such solutions exist are technically involved. [Fiore 2004]'s *axiomatic domain theory* axiomatises categorical structure sufficient for solving such equations. They aggregate axioms of different strengths dealing with the same domain-theoretic aspects of the category at hand; the strength of one axiom can compensate for the weakness of another. This theory allows us to treat recursive domain equations in $\mathbf{SSh}_{\omega\mathbf{CPO}}(C, \mathcal{J}, \mathcal{K})$ methodically.

This section is technical, and the main result is that $\mathbf{SSh}_{\omega\mathbf{CPO}}(C, \mathcal{J}, \mathcal{K})$ has an expansion to a category $\mathbf{SSh}_{\omega\mathbf{CPO}}(C, \mathcal{J}, \mathcal{K})_\perp$ of separated sheaves of $\omega$-cpos and *partial maps* between them, supporting the solution of recursive domain equations. The type-formers of FPC, that will denote locally continuous mixed-variance functors over $\mathbf{SSh}_{\omega\mathbf{CPO}}(C, \mathcal{J}, \mathcal{K})$, then have a locally continuous extension to $\mathbf{SSh}_{\omega\mathbf{CPO}}(C, \mathcal{J}, \mathcal{K})_\perp$, allowing us to use the solutions of recursive domain equations as denotations of recursive types.

### 5.2 Axiomatic Structure

We begin by isolating the structure Fiore postulates as it applies to $\mathbf{SSh}_{\omega\mathbf{CPO}}(C, \mathcal{J}, \mathcal{K})$. For the full account, see Fiore's thesis. A *(***Pos***)-domain structure* $\mathfrak{D}$ is a pair $\left(C_{\mathfrak{D}}, \overline{\mathfrak{M}}_{\mathfrak{D}}\right)$ consisting of a **Pos**-enriched category $C_{\mathfrak{D}}$, and a locally small full-on-objects subcategory $\overline{\mathfrak{M}}_{\mathfrak{D}}$ consisting solely of monomorphisms such that for every $m : D \rightarrowtail Y$ in $\overline{\mathfrak{M}}_{\mathfrak{D}}$ and $f : X \to Y$ in $C_{\mathfrak{D}}$:

- the pullback of $m$ along $f$ exists in $C_{\mathfrak{D}}$; and
- in every pullback diagram, the pulled back morphism $f^*m : f^*D \rightarrowtail X$ is in $\overline{\mathfrak{M}}_{\mathfrak{D}}$.

We call $C_{\mathfrak{D}}$ the category of *total maps* and the monos in $\overline{\mathfrak{M}}_{\mathfrak{D}}$ *admissible*.

**Example 1** ($\mathfrak{M}$-Classifiable Mono)**.** We call a mono $n : D \hookrightarrow F$ $\mathfrak{M}$*-classifiable* if it arises as a pullback

$$\begin{array}{ccc} D & \longrightarrow & \mathbb{1} \\ {\scriptstyle n}\big\downarrow & \lrcorner & \big\downarrow{\scriptstyle \top} \\ F & \xrightarrow{\chi_n} & \mathfrak{M}, \end{array}$$

where we write $\top$ for the morphism $\top_C(\alpha) = \mathrm{id}_C$. Here, $\chi_n$ is called the *characteristic function* of $n$. □

Lemma 5.1. *Given a $\mathfrak{M}$-classifiable mono $n : D \hookrightarrow F$. Its characteristic function is uniquely determined.*

Proof. Indeed,

$$\begin{aligned} (\chi_n)_C(\alpha) &= \bigvee\{U \xrightarrow{m} C \in \mathfrak{M}C \mid m \leq (\chi_n)_C(\alpha)\} \\ &= \bigvee\{U \xrightarrow{m} C \in \mathfrak{M}C \mid m^*(\chi_n)_C(\alpha) = \mathrm{id}_U\} \\ &\overset{\substack{\text{naturality } \chi_n \\ \downarrow}}{=} \bigvee\{U \xrightarrow{m} C \in \mathfrak{M}C \mid (\chi_n)_U(F(m)(\alpha)) = \mathrm{id}_U\} \\ &= \bigvee\{U \xrightarrow{m} C \in \mathfrak{M}C \mid F(m)(\alpha) \in n[DU]\}. \end{aligned}$$

That is, the characteristic function $\chi_n$ of $D$ sends $\alpha \in FC$ to the greatest $m \in \mathfrak{M}C$, such that $F(m)(\alpha)$ lies in $D$. □

Proposition 5.2. *$\mathfrak{M}$-classifiable monos define a domain structure on* $\mathbf{SSh}_{\omega\mathbf{CPO}}(C, \mathcal{J}, \mathcal{K})$.

Proof. To see that admissible monos are closed under pullback, note that monos are while pullback squares can be pasted.

To see that $\mathrm{id}_F$ is an admissible mono, note that it has characteristic function $!_F; \top$.

Suppose that $n : H \hookrightarrow G$ and $m : G \hookrightarrow F$ are admissible monos. We show that $n; m$ is as well. WLOG we may assume that $n_C$ and $m_C$ consist of subset embeddings. Observe that $\chi_m(\alpha)$ is the greatest $m' \in \mathfrak{M}$ such that $F(m')(\alpha) \in G$. In particular, $F(\chi_m(\alpha))(\alpha) \in G$. We claim that $\chi_{n;m}(\alpha) \overset{\text{def}}{=} \chi_n(F(\chi_m(\alpha))(\alpha)); \chi_m(\alpha)$ is its characteristic function. To see that this defines the desired characteristic functions, observe that

$$\begin{aligned} \big\{\alpha \in FC \mid \chi_{n;m}(\alpha) = \mathrm{id}\big\} &= \{\alpha \in FC \mid \chi_n(F(\chi_m(\alpha))(\alpha)); \chi_m(\alpha) = \mathrm{id}\} \\ &= \{\alpha \in FC \mid \chi_m(\alpha) = \mathrm{id} \wedge \chi_n(F(\chi_m(\alpha))(\alpha)) = \mathrm{id}\} \\ &= \{\alpha \in FC \mid \chi_m(\alpha) = \mathrm{id} \wedge \chi_n(F(\mathrm{id})(\alpha)) = \mathrm{id}\} \\ &= \{\alpha \in FC \mid \chi_m(\alpha) = \mathrm{id} \wedge \chi_n(\alpha) = \mathrm{id}\} \\ &= \{\alpha \in GC \mid \chi_n(\alpha) = \mathrm{id}\} \\ &= HC \end{aligned}$$

We show that $\chi_{n;m}$ is a natural transformation. Indeed, given $g : C' \to C$ and $\alpha \in FC$ such that $(\chi_m)_C(\alpha) : U \to C$, using the fact that pullbacks composed, together with the naturality[3] of $\chi_m$ and $\chi_n$, we have

$$\begin{aligned}
(\chi_{n;m})_{C'}(F(g)(\alpha)) &= (\chi_n)_{g^*U}(F((\chi_m)_{C'}(F(g)(\alpha)))(F(g)(\alpha))); (\chi_m)_{C'}(F(g)(\alpha)) \\
&= (((\chi_m)_C(\alpha))^* g)^*((\chi_n)_U(F((\chi_m)_U(\alpha))(\alpha))); (\chi_m)_{C'}(F(g)(\alpha)) \\
&= (((\chi_m)_C(\alpha))^* g)^*((\chi_n)_U(F((\chi_m)_U(\alpha))(\alpha))); g^*(\chi_m)_C(\alpha) \\
&= g^*((\chi_n)_U(F((\chi_m)_U(\alpha))(\alpha)); (\chi_m)_C(\alpha)) \\
&= g^*((\chi_n)_U(F((\chi_m)_U(\alpha))(\alpha)); (\chi_m)_C(\alpha)) \\
&= g^*((\chi_{n;m})_C(\alpha)) \\
&= \mathfrak{M}(g)((\chi_{n;m})_C(\alpha)).
\end{aligned}$$

[3]We are also using the fact that $G$ and $H$ are subpresheaves of $F$ here, meaning that they have the same functorial action.

We show that $\chi_{n;m}$ is $\omega$-continuous to complete the proof. Let $(\alpha_k)_{k\in\mathbb{N}}$ be an $\omega$-chain in $FC$.

$$\begin{aligned}
\chi_{n;m}(\sup_i \alpha_i) &= \chi_n(F(\chi_m(\sup_i \alpha_i))(\sup_i \alpha_i)); \chi_m(\sup_i \alpha_i) \\
&\quad \text{$\omega$-continuity } \chi_m \downarrow \\
&= \chi_n(F(\sup_i \chi_m(\alpha_i))(\sup_i \alpha_i)); (\sup_i \chi_m(\alpha_i)) \\
&\quad \text{$\alpha$-renaming} \downarrow \\
&= \chi_n(F(\sup_i \chi_m(\alpha_i))(\sup_j \alpha_j)); (\sup_i \chi_m(\alpha_i)) \\
&\quad \text{$\omega$-continuity } F(g) \text{ for any } g \downarrow \\
&= \chi_n(\sup_j F(\sup_i \chi_m(\alpha_i))(\alpha_j)); (\sup_i \chi_m(\alpha_i)) \\
&\quad \text{$\omega$-continuity } \chi_n \downarrow \\
&= (\sup_j \chi_n(F(\sup_i \chi_m(\alpha_i))(\alpha_j))); (\sup_i \chi_m(\alpha_i)) \\
&\quad \text{$\omega$-continuity } -; m' \text{ for any } m' \in \mathfrak{M} \text{ as it has a right adjoint } m'^{*} \downarrow \\
&= \sup_j(\chi_n(F(\sup_i \chi_m(\alpha_i))(\alpha_j)); (\sup_i \chi_m(\alpha_i))) \\
&\quad (\chi_m(\alpha_i))_{i\in\mathbb{N}} \text{ covers } \sup_i \chi_m(\alpha_i) \text{ while } \big(\chi_n(F(\chi_m(\alpha_i))(\alpha_j))\big)_{i\in\mathbb{N}} \text{ is a matching family with amalgamation} \\
&\quad \chi_n(F(\sup_i \chi_m(\alpha_i))(\alpha_j)); (\sup_i \chi_m(\alpha_i)) \downarrow \\
&= \sup_j(\mathrm{glue}_i(\chi_n(F(\chi_m(\alpha_i))(\alpha_j)))) \\
&\quad \text{amalgamations of matching families are unique} \downarrow \\
&= \sup_j \sup_i(\chi_n(F(\chi_m(\alpha_i))(\alpha_j)); (\chi_m(\alpha_i))) \\
&\quad \text{sup of sup of $\omega$-chain of $\omega$-chains} \downarrow \\
&= \sup_i \chi_n(F(\chi_m(\alpha_i))(\alpha_i)); \chi_m(\alpha_i) \\
&= \sup_i (\chi_{n;m})_C(\alpha_i)
\end{aligned}$$

□

### 5.3 Axioms and Derived Structure

We develop the domain theory following Fiore's development and describe the axioms it validates, summarised in 1. While doing so, we recall the structure Fiore derives from these axioms.

*Partial maps.* Each domain structure $\mathfrak{D} = \left(C, \overline{\mathfrak{M}}\right)$ constructs a *category* $\mathbf{p}\mathfrak{D}$ *of partial maps*. Let $X$, $Y$ be $C$-objects. A *partial map description* $u : X \rightharpoonup Y$ from $X$ to $Y$, is a pair $u = (\partial_u, \overline{u})$ consisting of an admissible mono $\partial_u : D_u \rightarrowtail X$ and a $C$-morphism $\overline{u} : D_u \longrightarrow Y$. Two descriptions $u$ and $v$ are *equivalent*, $u \equiv v$, when there is an isomorphism $i : D_u \xrightarrow{\cong} D_v$ satisfying: $i; \overline{v} = \overline{u}$ and $i; \partial_v = \partial_u$.

A *partial map* $u : X \rightharpoonup Y$ is the equivalence class of a description, bearing in mind that $\overline{\mathfrak{M}}$ is locally small. E.g., our category of sheaves, choose natural transformations consisting of inclusions as the canonical representatives $\partial_u : D_u \subset X$, which uniquely determine the description. Partial

**Structure**

| | |
|---|---|
| $C_\mathfrak{D}$ | total map category $\omega$**Qbs** |
| $f \leq g$ | **Pos**-enrichment pointwise order |
| $\overline{\mathfrak{M}}_\mathfrak{D}$ | admissible monos $\mathfrak{M}$-classifiable monos |

**Axioms**

| | |
|---|---|
| $(\dashv)$ | every object has a partial map classifier $\downarrow_X : X \to X_\perp$ |
| (fup) | every admissible mono is full and upper-closed |
| $(\dashv_\leq)$ | $\llcorner - \lrcorner$ is locally monotone |
| $(C_\bigvee)$ | $C_\mathfrak{D}$ is $\omega$**CPO**-enriched |
| $(U)$ | $\omega$-colimits behave uniformly (lemma 5.9) |
| $(\mathbb{1})$ | $C_\mathfrak{D}$ has a terminal object |
| $(\to_\leq)$ | $C_\mathfrak{D}$ has locally monotone exponentials |
| $(+)$ | locally continuous total coproducts |
| $(?!)$ | $\mathbb{0} \to \mathbb{1}$ is admissible |
| $(\times_\bigvee)$ | $C_\mathfrak{D}$ has a locally continuous products |
| $(CL)$ | $C_\mathfrak{D}$ is cocomplete |

**Derived axioms/structure**

| | |
|---|---|
| $\mathbf{p}\mathfrak{D}$ | partial map category |
| $-_\perp$ | partiality monad |
| $(\dashv_\bigvee)$ | the adjunction $J \dashv L$ is locally continuous |
| $(\mathbf{p}_\bigvee)$ | $\mathbf{p}\mathfrak{D}$ is $\omega$**CPO**-enriched |
| $(\mathbb{1}_\leq)$ | $\mathbf{p}\mathfrak{D}$ has a partial terminal |
| $(\otimes)$ | $\mathbf{p}\mathfrak{D}$ has partial products |
| $(\otimes_\bigvee)$ | $(\otimes)$ is locally continuous |
| $(\to_\bigvee)$ | $C_\mathfrak{D}$ has locally continuous exponentials |
| $(\rightharpoonup_\bigvee)$ | $\mathbf{p}\mathfrak{D}$ has locally continuous partial exponentials |
| $(\mathbf{p}CL)$ | $\mathbf{p}\mathfrak{D}$ is cocomplete |
| $(\mathbf{p}+_\bigvee)$ | $\mathbf{p}\mathfrak{D}$ has locally continuous partial coproducts |
| $(BC)$ | $J : C \hookrightarrow \mathbf{p}\mathfrak{D}$ is a bilimit compact expansion |

Fig. 1. The axiomatic domain theory of $\mathbf{SSh}_{\omega\mathbf{CPO}}(C, \mathcal{J}, \mathcal{K})$ and its probabilistic power-domain

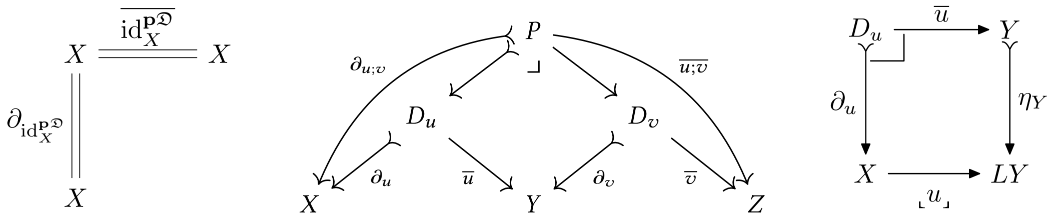


Fig. 2. Partial identities and composition (left) and characteristic maps (right).

maps form a category $\mathbf{p}\mathfrak{D}$, with identities given by $[\mathrm{id}, \mathrm{id}]$, and the composition $u; v : X \overset{u}{\rightharpoonup} Y \overset{v}{\rightharpoonup} Z$ via pullback (see 2, left). We have an identity-on-objects, faithful functor $J : C \to \mathbf{p}\mathfrak{D}$ mapping each total map $f : X \to Y$ to $[\mathrm{id}, f] : X \rightharpoonup Y$.

*Representability.* Given a domain structure, a *classifier of partial maps* is a collection of admissible monos $(\downarrow_X : X \rightarrowtail LX)_{X \in C}$, indexed by the objects of $C$, such that for every $Y$, and every partial map $f : X \rightharpoonup Y$, there is a unique (total) map $\llcorner f \lrcorner : X \to LY$ such that 2 (right) is a pullback square. We call $\llcorner f \lrcorner$ the *total representation* of $f$. Each classifier $\downarrow$ of partial maps induces a right adjoint $J \dashv L : \mathbf{p}\mathfrak{D} \to C$ with $\downarrow$ as unit.

Theorem 5.3. *In* $\mathbf{SSh}_{\omega\mathbf{CPO}}(C, \mathcal{J}, \mathcal{K})$*, the morphisms* $\mathrm{return}_C : C \hookrightarrow C_\perp$ *give a classifier of partial maps. (Axiom* $(\dashv)$*is satisfied.)*

Proof. Given $F \xrightarrow{f} G_\perp$, we can define $\partial_f : D_f \hookrightarrow F$ and $D_f \xrightarrow{\overline{f}} G$ by taking the following pullback. (In fact, this is the only choice we have.)

$$\begin{array}{ccc} D_f & \xrightarrow{\overline{f}} & G \\ {\scriptstyle \partial_f}\big\downarrow & \lrcorner & \big\downarrow{\scriptstyle \mathrm{return}_G} \\ F & \xrightarrow{f} & G_\perp. \end{array}$$

Then, we have a pullback diagram obtained by the composition of pullbacks

$$\begin{array}{ccccc} D_f & \xrightarrow{\overline{f}} & G & \longrightarrow & \mathbb{1} \\ {\scriptstyle \partial_f}\big\downarrow & \lrcorner & \big\downarrow{\scriptstyle \mathrm{return}_G} & \lrcorner & \big\downarrow{\scriptstyle \top} \\ F & \xrightarrow{f} & G_\perp & \xrightarrow{\mathsf{fst}} & \mathfrak{M}. \end{array}$$

The left diagram is a pullback by construction of $\partial_f$ and $\overline{f}$. The right diagram is a pullback as $\mathsf{fst}(\psi(\alpha)) = \psi^1(\alpha)$ for any $\psi : H \to G_\perp$. Therefore, $\mathsf{fst}(\psi(\alpha)) = \top(!_H(\alpha))$ implies that $\psi^1(\alpha) = \mathrm{id}$. This shows that $\psi$ factors over $\mathrm{return}_G$, so the right diagram is a pullback. We see that we can use the characteristic function $\chi_{\partial_f} \stackrel{\mathrm{def}}{=} f; \mathsf{fst} = f^1$. We conclude that $\partial_f$ is an admissible mono.

Conversely, suppose we are given an admissible mono $\partial_f : D_f \hookrightarrow F$ with characteristic function $\chi_{\partial_f}$. and $\overline{f} : D_f \to G$. We show how to construct $f$ and demonstrate its uniqueness. First, observe that by the pasting of pullback diagrams above $f^1 = f; \mathsf{fst}$ has to be a characteristic function for $\partial_f$. By uniqueness and existence of that characteristic function, we get that $f^1 = \chi_{\partial_f}$. Next, we turn to $f^2$. By naturality of $f$, we have that for any $g : C' \to C$, $f_{C'}(F(g)(\alpha)) = G_\perp(g)(f_C(\alpha)) = (g^* f_C^1(\alpha), G(f_C^1(\alpha)^* g)(f_C^2(\alpha)))$. In particular, for $g = f_C^1(\alpha) : U_\alpha \hookrightarrow C$, we have that $f_{U_\alpha}(F(f_C^1(\alpha))(\alpha)) = (\mathrm{id}_{U_\alpha}, f_C^2(\alpha))$. Therefore, $F(f_C^1(\alpha))(\alpha) \in D_f$ and $\overline{f}_{U_\alpha}(F(f_C^1(\alpha))(\alpha)) = f_C^2(\alpha)$. By naturality of $\overline{f}$, also $f_C^2(\alpha) = G(f_C^1(\alpha))(\overline{f}_C(\alpha))$. We see that $f^2$ is uniquely determined by $f^1$ and $\overline{f}$. To see that

$$f_C^2(\alpha) \stackrel{\mathrm{def}}{=} G(f_C^1(\alpha))(\overline{f}_C(\alpha))$$

can be taken as a definition, we verify that this makes $f$ into an $\omega$-continuous natural transformation $F \to G_\perp$. $\omega$-continuity follows by the following argument, using the $\omega$-continuity of $f^1$, $\overline{f}$ and $G(g)$, and the fact that $\left(f_C^1(\alpha_n)\right)_{n\in\mathbb{N}}$ covers $\sup_n f_C^1(\alpha_n) = f_C^1(\sup_n \alpha_n)$ while $G$ is a $\mathcal{J}$-sheaf:

$$\begin{aligned}
&\sup_n (f_C^1(\alpha_n), G(f_C^1(\alpha_n))(\overline{F}_C(\alpha_n))) \\
&= (\sup_n f_C^1(\alpha_n), \mathrm{glue}_{n'}(\sup_n G(f_C^1(\alpha_{n'}) \leq f_C^1(\alpha_n))(G(f_C^1(\alpha_n))(\overline{F}_C(\alpha_n))))) \\
&= (\sup_n f_C^1(\alpha_n), \mathrm{glue}_{n'}(\sup_n G(f_C^1(\alpha_{n'}))(\overline{F}_C(\alpha_n)))) \\
&= (\sup_n f_C^1(\alpha_n), \mathrm{glue}_{n'}(G(f_C^1(\alpha_{n'}))(\sup_n \overline{F}_C(\alpha_n)))) \\
&= (\sup_n f_C^1(\alpha_n), \mathrm{glue}_{n'}(G(f_C^1(\alpha_{n'}))(\overline{F}_C(\sup_n \alpha_n)))) \\
&= (f_C^1(\sup_n \alpha_n), G(f_C^1(\sup_n \alpha_n))(\overline{F}_C(\sup_n \alpha_n)))
\end{aligned}$$

Finally, we show naturality of this definition of $f$. Suppose we are given $C' \xrightarrow{g} C$ and $\beta \in FC'$. Then, by naturality of $f^1$ and $\overline{f}$,

$$
\begin{aligned}
f_C(F(g)(\beta)) &= (f^1_C(F(g)(\beta)), G(f^1_C(F(g)(\beta)))(\overline{f}_C(F(g)(\beta)))) \\
&= (f^1_C(F(g)(\beta)), G(f^1_C(F(g)(\beta)))(G(g)(\overline{f}_{C'}(\beta)))) \\
&= (g^* f^1_{C'}(\beta), G(g^* f^1_{C'}(\beta))(G(g)(\overline{f}_{C'}(\beta)))) \\
&= (g^* f^1_{C'}(\beta), G(g^* f^1_{C'}(\beta); g)(\overline{f}_{C'}(\beta))) \\
&= (g^* f^1_{C'}(\beta), G(f^1_{C'}(\beta)^* g; f^1_{C'}(\beta))(\overline{f}_{C'}(\beta))) \\
&= (g^* f^1_{C'}(\beta), G(f^1_{C'}(\beta)^* g)(G(f^1_{C'}(\beta))(\overline{f}_{C'}(\beta)))) \\
&= G_\perp(g)((f^1_{C'}(\beta), G(f^1_{C'}(\beta))(\overline{f}_{C'}(\beta)))) \\
&= G_\perp(g)(f_{C'}(\beta)).
\end{aligned}
$$

□

Proposition 5.4. *In fact, we get an equivalence of categories between* $\mathbf{p}\mathfrak{D}$ *and* $\mathbf{SSh}_{\omega\mathrm{CPO}}(C, \mathcal{J}, \mathcal{K})_\perp$.

Proof. First, observe that we have a pullback square

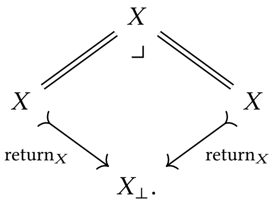


This shows that $\llcorner \mathrm{id} \lrcorner = \mathrm{return}$.

Next, suppose we are given two partial map descriptions $u = (\partial_u, \overline{u})$ from $X$ to $Y$ and $v = (\partial_v, \overline{v})$ from $Y$ to $Z$. We claim that $\llcorner u \lrcorner ; \gg\!= \llcorner v \lrcorner = \llcorner u; v \lrcorner$ where we compose $u; v$ in $\mathbf{p}\mathfrak{D}$. To show this, we need to show that we have a pullback:

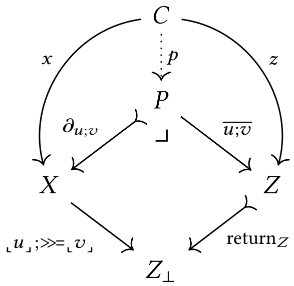


meaning that for each $x$ and $z$ such that $x; \llcorner u \lrcorner ; \gg\!= \llcorner v \lrcorner = z; \mathrm{return}_Z$ we get a unique $p$ such that $p; \partial_{u;v} = x$ and $p; \overline{u;v} = z$.

To see that we in fact get this unique $p$, observe that $x; \llcorner u \lrcorner ; \gg\!= \llcorner v \lrcorner = z; \mathrm{return}_Z$ implies that there exists some $y$ such that $x; \llcorner u \lrcorner = y; \mathrm{return}_Y$. Indeed, $(g^1(f^2(a)); f^1(a), g^2(f^2(a))) = (f^1(a), f^2(a)) \gg\!= g = f(a) \gg\!= g = \mathrm{return}(z(a)) = (\mathrm{id}, z(a))$ implies that $f^1(a)$ is an iso, as $f^1(a)$ is a mono by assumption and $g^1(f^2(a)); f^1(a) = \mathrm{id}$ implies it is split epi. As $\mathrm{return}_Y$ is a mono, this $y$ is uniquely determined. Then, $y; \mathrm{return}_Y = x; \llcorner u \lrcorner$, so we get a unique $d_u$ such that $d_u; \partial_u = x$ and $d_u; \overline{u} = y$ Similarly, as $y; \llcorner v \lrcorner = y; \mathrm{return}_Y; \gg\!= \llcorner v \lrcorner = x; \llcorner u \lrcorner ; \gg\!= \llcorner v \lrcorner = z; \mathrm{return}_Z$, we get a unique $d_v$ such that $d_v; \overline{v} = z$ and $d_v; \partial_v = y$. Now, finally, $d_u; \overline{u} = y = d_v; \partial_v$, so we get our desired unique $p$.

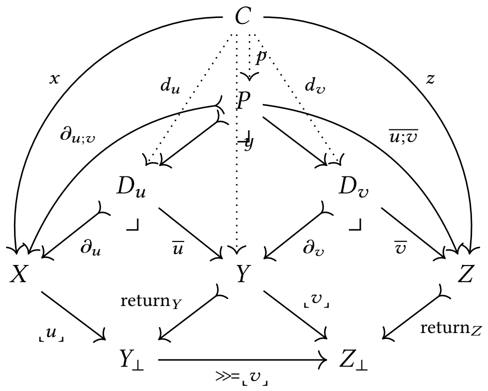


□

In fact, one easily sees that the induced adjunction $J \dashv L$ is the Kleisli resolution of the monad $(-)_\bot$

*Enrichment.* The order enrichment of $\mathbf{SSh}_{\omega\mathbf{CPO}}(C, \mathcal{J}, \mathcal{K})$ is an $\boldsymbol{\omega}$**CPO**-enrichment. Moreover, the partial map category inherits a potential **Pos**-enrichment: for $u, v : X \rightharpoonup Y$, write $u \sqsubseteq v$ to mean that there is some $i : D_u \to D_v$ such that $\partial_u = i; \partial_v$ and $\overline{u} \le i; \overline{v}$. The isomorphism $\mathbf{p}\mathfrak{D} \cong \mathbf{SSh}_{\omega\mathbf{CPO}}(C, \mathcal{J}, \mathcal{K})_\bot$ respects $\sqsubseteq$ and $\le$, i.e., $u \sqsubseteq v : X \rightharpoonup Y$ iff $\llcorner u \lrcorner \le \llcorner v \lrcorner$ as morphisms $X \to Y_\bot$ in $\mathbf{SSh}_{\omega\mathbf{CPO}}(C, \mathcal{J}, \mathcal{K})$, and so $\mathbf{p}\mathfrak{D}$ is $\boldsymbol{\omega}$**CPO**-enriched. We can also deduce this fact from more fundamental axioms. First, postcomposition with any admissible mono is full and its image is upper-closed. As a consequence of Fiore's Prop. 4.2.4, the order $\sqsubseteq$ is a partial order and **Pos**-enriches $\mathbf{p}\mathfrak{D}$. Denote the inverse map to representation by $\ulcorner - \urcorner : \mathbf{SSh}_{\omega\mathbf{CPO}}(C, \mathcal{J}, \mathcal{K})(X, Y_\bot) \to \mathbf{p}\mathfrak{D}(X, Y)$. Because $\ulcorner - \urcorner$ is monotone, the adjunction $J \dashv L : \mathbf{p}\mathfrak{D}$ is locally monotone by Fiore's Prop. 4.5.4, and, as a consequence $\mathbf{p}\mathfrak{D}$ is $\boldsymbol{\omega}$**CPO**-enriched by Fiore's Prop. 4.5.3.

Lemma 5.5. *Postcomposition $-; m$ with any admissible mono $m : A \hookrightarrow Y$ is full and its image is upper closed.*

Proof. First note that this is obviously true for $m = \top : \mathbb{1} \hookrightarrow \mathfrak{M}$.

Next, observe that we have a pullback

$$\begin{array}{ccc} A & \xrightarrow{!_A} & \mathbb{1} \\ {\scriptstyle m}\big\downarrow & \lrcorner & \big\downarrow{\scriptstyle \top} \\ Y & \xrightarrow[\chi_m]{} & \mathfrak{M}. \end{array}$$

Now, pullbacks in $\mathbf{SSh}_{\omega\mathbf{CPO}}(C, \mathcal{J}, \mathcal{K})$ are computed pointwise. Full monos with upper closed image are closed under pullback in $\boldsymbol{\omega}$**CPO**. Therefore, $m_C$ is a full mono and has an upper closed image for all $C$.

Suppose that $f; m \le g; m$, for $f, g \in \mathbf{Hom}(B, A)$. Then, in particular, $m_C(f_C(b)) \le m_C(g_C(b))$ for all $C$ and $b$. As $m_C$ is a full mono, we get that $f_C(b) \ge g_C$ for all $C$ and $b$, and therefore $f_C \le g_C$ by definition of the order on $\mathbf{Hom}(B, A)$. We see that $-; m$ is a full mono.

Now, suppose that $f; m \le g$ for some $f \in \mathbf{Hom}(B, A)$ and $g \in \mathbf{Hom}(B, Y)$. Then, $m_C(f_C(b)) \le g_C(b)$ for all $C$ and $b$. As $m_C$ has an upper closed image, we get a unique $h_C(b) \in A$ such that $m_C(h_C(b)) = g_C(b)$. As $m_C$ is a full mono, $h_C$ is an $\omega$-continuous function. Moreover, as $A$ is a subpresheaf of $Y$, it is a natural transformation. We see that $h \in \mathbf{Hom}(B, A)$ and $g = h; m$. Therefore, $-; m$ has an upper closed image. □

*Uniformity.* As $\mathbf{SSh}_{\omega\mathbf{CPO}}(C, \mathcal{J}, \mathcal{K})$ is cocomplete, it has local $\omega$-lubs, but these lubs can behave pathologically (See Fiore [Sec. 4.3.2]). The following *uniformity* axiom avoids such pathologies.

We write $(-)^+_{\mathcal{J}}$ for the functor from $\mathbf{PSh}(C)$ to $\mathcal{J}$-separated presheaves $\mathbf{SPSh}(C, \mathcal{J})$ on $C$ which is given by

$$P^+_{\mathcal{J}}C \stackrel{\text{def}}{=} \mathrm{colim}_{R\in\mathcal{J}C}\mathbf{Nat}(R, P)$$

(and similarly for $(-)^+_{\mathcal{K}}$). That is, the elements of $P^+_{\mathcal{J}}C$ are equivalence classes $[(R, x)]$ of natural transformations $x$ from some $\mathcal{J}$-covering sieve $R$ on $C$ to $P$, where we identify $x : R \longrightarrow P$ and $y : S \longrightarrow P$ iff there exists some $\mathcal{J}$-covering sieve $Q \subseteq R \cap S$ such that $x$ and $y$ agree on their restriction to $Q$. It is well-known that $a_{\mathcal{J}} \stackrel{\text{def}}{=} (-)^+_{\mathcal{J}}; (-)^+_{\mathcal{J}}$ gives a finite limit preserving left adjoint to the inclusion $\mathbf{Sh}(C, \mathcal{J}) \hookrightarrow \mathbf{PSh}(C)$ (see e.g. [MacLane and Moerdijk 2012], theorem III.5.1).

Lemma 5.6. *Suppose that $P \in \mathbf{PSh}(C)$ is $\mathcal{K}$-separated. Then, $P^+_{\mathcal{J}}$ is too.*

Proof. Let $x, y \in P^+_{\mathcal{J}}C$ and suppose that $P^+_{\mathcal{J}}(h)(x) = P^+_{\mathcal{J}}(h)(y)$ for all $h$ in some $Q \in \mathcal{K}C$. We want to show that $x = y$. Let us represent $x = \{x_f \mid f \in R\}$ and $y = \{y_g \mid g \in S\}$ for $R, S \in \mathcal{J}C$. Observe that $R \cap S \in \mathcal{J}C$. Let $D \xrightarrow{k} C \in R \cap S$. We are done if we can show that $x_k = y_k$. Observe that $k^*Q = \left\{E \xrightarrow{g} D \mid g;k \in Q\right\} \in \mathcal{K}D$. Let us note that $h = g;k \in Q$. Then, for $g \in k^*Q$, we have that $P(g)(x_k) = x_{g;k} = x_h = P^+_{\mathcal{J}}(h)(x) = P^+_{\mathcal{J}}(h)(y) = y_h = y_{g;k} = P(g)(y_k)$. As $P$ is $\mathcal{K}$-separated and $k^*Q \in \mathcal{K}D$, it follows that $x_k = y_k$. □

Corollary 5.7. $(-)^+_{\mathcal{J}}$ *gives a left adjoint to the inclusion* $\mathbf{SSh}(C, \mathcal{J}, \mathcal{K}) \hookrightarrow \mathbf{SPSh}(C, \mathcal{K})$.

Proof. By the previous, the left adjoint $a_{\mathcal{J}}$ restricts to give a left adjoint to the inclusion $\mathbf{SSh}(C, \mathcal{J}, \mathcal{K}) \hookrightarrow \mathbf{SPSh}(C, \mathcal{K})$.

Further, note that a $\mathcal{K}$-separated presheaf is, in particular, $\mathcal{J}$-separated. By [MacLane and Moerdijk 2012] lemma III.5.4, $P^+_{\mathcal{J}}$ is a $\mathcal{J}$-sheaf if $P$ is $\mathcal{J}$-separated. Therefore, $a_{\mathcal{J}} = (-)^+_{\mathcal{J}}; (-)^+_{\mathcal{J}} = (-)^+_{\mathcal{J}}$ when restricted to $\mathbf{SPSh}(C, \mathcal{K})$. □

Observe further that for a $\mathcal{J}$-separated (so, in particular, for a $\mathcal{K}$-separated) presheaf $P$, we have a canonical representative of each equivalence class $[(R, x)] \in P^+_{\mathcal{J}}C$. Indeed, given $(R, x)$, $(S, y)$, members of the same equivalence class in $P^+_{\mathcal{J}}C$, we can observe that $x$ and $y$ agree on the $\mathcal{J}$-covering sieve $R \cap S$. Let $D \xrightarrow{k} C \in R \cap S$. We want to show that $x_D(k) = y_D(k)$. As $P$ is $\mathcal{J}$-separated, it is enough to show that there is some $\mathcal{J}$-covering sieve $Q$ of $D$ such that $P(f)(x_D(k)) = P(f)(y_D(k))$ for all $E \xrightarrow{f} D \in Q$. As $(R, x)$ and $(S, y)$ are members of the same equivalence class, we know there is some $R \cap S \supseteq T \in \mathcal{J}C$ such that $x_E(h) = y_E(h)$ for all $h \in T$. Now, take $Q \stackrel{\text{def}}{=} k^*T = \left\{E \xrightarrow{f} D \mid f;k \in T\right\}$. Then, $P(f)(x_D(k)) = x_E(f;k) = y_E(f;k) = P(f)(y_D(k))$ for all $f \in Q$. It follows that $x$ and $y$ agree on $R \cap S$. As a consequence, we can represent the equivalence class $[(R, x)]$ canonically by its greatest member: $(R_{\text{top}}, x_{\text{top}})$, where $R_{\text{top}} \stackrel{\text{def}}{=} \bigcup \{R' \mid (R', x') \in [(R, x)]\}$ and $x_{\text{top}} = \text{glue}\,\{x' \mid (R', x') \in [(R, x)]\}$.

Lemma 5.8. *Admissible monos in* $\mathbf{SSh}_{\omega\mathbf{CPO}}(C, \mathcal{J}, \mathcal{K})$ *are, in each component, in particular, full embeddings of upwards closed subsets.*

Proof. Let $m : A \hookrightarrow Y$ be an admissible mono with characteristic function $\chi_m$. Therefore, $m$ arises as the pullback of $\top : \mathbb{1} \longrightarrow \mathfrak{M}$ along $\chi_m$. As pullbacks (as any limits) are computed pointwise in $\mathbf{SSh}_{\omega\mathbf{CPO}}(C, \mathcal{J}, \mathcal{K})$, it follows that for each $C \in C$, the following square is a pullback in $\boldsymbol{\omega}\mathbf{CPO}$.

$$\begin{array}{ccc} AC & \xrightarrow{!_{AC}} & \mathbb{1} \\ {\scriptstyle m_C}\downarrow & \lrcorner & \downarrow{\scriptstyle \top_C} \\ YC & \xrightarrow[(\chi_m)_C]{} & \mathfrak{M}C \end{array}$$

That is, $AC = \{y \in YC \mid (\chi_m)_C(y) = \mathrm{id}_C\}$, equipped with the induced order from $YC$ (immediately showing that $m_C$ is a full mono). As $\mathrm{id}_C$ is maximal in $\mathfrak{M}C$, monotonicity of $(\chi_m)_C$ gives us that $AC$ is upwards closed in $YC$: $(\chi_m)_C(y) = \mathrm{id}_C$ implies that $(\chi_m)_C(y') \geq \mathrm{id}_C$ hence $(\chi_m)_C(y') = \mathrm{id}_C$ for any $y' \geq y$. □

Lemma 5.9 (Uniformity). *Let $(i_{n+1} : D_n \rightarrowtail D_{n+1})_{n\in\mathbb{N}}$ be an $\omega$-chain of admissible monos in* $\mathbf{SSh}_{\omega\mathrm{CPO}}(\mathcal{C}, \mathcal{J}, \mathcal{K})$.

- *Every colimiting cocone $\left(D, (\mu_n : D_n \to D)_{n\in\mathbb{N}}\right)$ consists of admissible monos.*
- *The mediating morphism into any other cocone of admissible monos is also an admissible mono.*

Proof. Writing $\chi_{i_{n+1}}$ for the characteristic function $D_{n+1} \to \mathfrak{M}$ of $i_{n+1}$, let us define

$$DC \stackrel{\text{def}}{=} \left\{ \left(U_n \xrightarrow{m_n} C, \alpha_n\right)_{n\in\mathbb{N}} \middle| \forall n \in \mathbb{N}. m_n \in \mathfrak{M}C,\ m_n \leq m_{n+1},\ \sup_n m_n = \mathrm{id}_C,\ \alpha_n \in D_n(U_n),\right.$$
$$\left. D_{n+1}(m_n \leq m_{n+1})(\alpha_{n+1}) = i_{n+1}(\alpha_n),\ \chi_{i_{n+1}}(\alpha_{n+1}) = m_{n+1}^* m_n \right\}.$$

That is, its elements $\alpha$ consist of an $\omega$-chain $(U_n)_{n\in\mathbb{N}}$ in $\mathfrak{M}C$ with supremum $C$ (hence, which forms a $\mathcal{J}$-cover of $C$) together with a "matching family" of elements of $D_n$ with respect to this cover. We think of $U_n$ as the largest subobject of $C$ of elements which $\alpha$ maps to $D_n$ (if we think of $\alpha_C$ as a kind of abstraction of a function from $C$ to $D$). This definition should be reminiscent of that of $(-)_\perp$.

We can observe that $D$ defines a presheaf on $\mathcal{C}$ if we define for $C' \xrightarrow{f} C$:

$$D(f)\left(U_n \xrightarrow{m_n} C, \alpha_n\right)_{n\in\mathbb{N}} \stackrel{\text{def}}{=} \left(f^* m_n, D_n(m_n^* f)(\alpha_n)\right)_{n\in\mathbb{N}}.$$

Indeed, functoriality follows from the fact that pullbacks compose.

First, we demonstrate that $D$ is $\mathcal{K}$-separated. Let $R \in \mathcal{K}C$ and suppose that $D(f)((m_n, \alpha_n)_{n\in\mathbb{N}}) = D(f)((m'_n, \alpha'_n)_{n\in\mathbb{N}})$ for all $f \in R$. That is,

$$f^* m_n = f^* m'_n$$

and

$$D_n(m_n^* f)(\alpha_n) = D_n({m'_n}^* f)(\alpha'_n).$$

As $\mathfrak{M}$ is $\mathcal{K}$-separated, it follows that $m_n = m'_n$. Therefore,

$$D_n(m_n^* f)(\alpha_n) = D_n(m_n^* f)(\alpha'_n).$$

Observing that $m_n^* R \in \mathcal{K}$ and $D_n$ is $\mathcal{K}$-separated, it follows that $\alpha_n = \alpha'_n$. We see that $D$ is $\mathcal{K}$-separated (hence, in particular, $\mathcal{J}$-separated).

Let us show that $D$ is, in fact, a $\mathcal{J}$-sheaf. Let $R \in \mathcal{J}C$ and $\left(m_n^f, \alpha_n^f\right)_{n\in\mathbb{N}}$ a matching family of $D$ for $f \in R$. Then, as $\mathfrak{M}$ is a $\mathcal{J}$-sheaf and $m_n^- \in \mathbf{Nat}(R, \mathfrak{M})$, we can define

$$m_n \stackrel{\text{def}}{=} \mathrm{glue}^{\mathfrak{M}}_{f\in R} m_n^f.$$

Next, observe that $\alpha_n^{-;m_n} \in \mathbf{Nat}(m_n^* R, D_n)$ and $D_n$ is a $\mathcal{J}$-sheaf so we can define

$$\alpha_n \stackrel{\text{def}}{=} \mathrm{glue}^{D_n}_{g\in m_n^* R} \alpha_n^{g;m_n}.$$

As $\mathfrak{M}$ is an internal $\omega$-cpo in $\mathbf{Sh}(C, \mathcal{J})$, it follows that $m_n \leq m_{n+1}$ and $\sup_n m_n = \mathrm{id}_C$. Naturality of $i_{n+1}$ gives us that $D_{n+1}(m_n \leq m_{n+1}(\alpha_{n+1})) = i_{n+1}(\alpha_n)$. Finally, naturality of $\chi_{i_{n+1}}$ gives us that $\chi_{n+1}(\alpha_{n+1}) = m^*_{n+1} m_n$. We see that $(m_n, \alpha_n)_{n\in\mathbb{N}} \in DC$. Next, for $g \in R$,

$$\begin{aligned} D(g)((m_n, \alpha_n)_{n\in\mathbb{N}}) &= D(g)(\left(\mathrm{glue}^{\mathfrak{M}}_{f\in R} m^f_n, \mathrm{glue}_{h\in m^*_n R} \alpha^{h;m_n}_n\right)_{n\in\mathbb{N}}) \\ &= \left(g^* \mathrm{glue}^{\mathfrak{M}}_{f\in R} m^f_n, D_n(m^*_n g)(\mathrm{glue}^{D_n}_{h\in m^*_n R} \alpha^{h;m_n}_n\right)_{n\in\mathbb{N}}) \\ &= \left(m^g_n, D_n(m^*_n g)(\mathrm{glue}^{D_n}_{h\in m^*_n R} \alpha^{h;m_n}_n\right)_{n\in\mathbb{N}}) \\ &= \left(m^g_n, \alpha^g_n\right)_{n\in\mathbb{N}} . \end{aligned}$$

We see that $D$ is a $\mathcal{J}$-sheaf.

We equip $DC$ with the partial order structure

$$(m_n, \alpha_n)_{n\in\mathbb{N}} \leq \left(m'_n, \alpha'_n\right)_{n\in\mathbb{N}} \stackrel{\text{def}}{=} \forall n \in \mathbb{N}. m_n \leq^{\mathfrak{M}} m'_n \ \wedge \ \alpha_n \leq D_n(m_n \leq m'_n)(\alpha'_n).$$

Observe that $D(f)$ is a monotone function $DC' \longrightarrow DC$. Indeed, given $(m_n, \alpha_n)_{n\in\mathbb{N}} \leq \left(m'_n, \alpha'_n\right)_{n\in\mathbb{N}}$, we have that

$$\forall n \in \mathbb{N}. f^* m_n \leq f^* m'_n \ \wedge \ D_n(m^*_n f)(\alpha_n) \leq^{D_n} D_n(m'^*_n f)(\alpha'_n)$$

as $f^*$ is monotone and $D_n(m^*_n f)(\alpha'_n) = D_n(f^* m_n \leq f^* m_n')(D_n(m'^*_n f)(\alpha'_n))$. That is, $D$ defines a **Pos**-valued presheaf.

We show that $\leq^D$ forms a $\mathcal{J}$-sheaf, to conclude that $D$ is an object in $\mathbf{SSh}_{\mathbf{Pos}}(C, \mathcal{J}, \mathcal{K})$. Clearly, $\leq^D \subseteq D \times D$ is $\mathcal{K}$-separated as a subpresheaf of a separated presheaf. So we only need to show the existence of an amalgamation for each matching family $\left(\left(\left(m^f_n, \alpha^f_n\right)_{n\in\mathbb{N}}, \left(l^f_n, \beta^f{}_n\right)_{n\in\mathbb{N}}\right)\right)_{f\in R}$ for $\leq^D$ with respect to a cover $R \in \mathcal{J}C$. That is, we have, for all $D \xrightarrow{f} C$ in $R$ that

$$m^f_n \leq^{\mathfrak{M}} l^f_n$$

and

$$\alpha^f_n \leq^{D_n} D_n(m^f_n \leq l^f_n)(\beta^f_n).$$

Seeing that $D \times D$ is a $\mathcal{J}$-sheaf and this is, in particular, a matching family for $D \times D$, we know its amalgamation needs to be

$$(\left(m_n \stackrel{\text{def}}{=} \mathrm{glue}^{\mathfrak{M}}_{f\in R} m^f_n, \mathrm{glue}^{D_n}_{g\in m^*_n R} \alpha^{g;m_n}_n\right)_{n\in\mathbb{N}}, \left(l_n \stackrel{\text{def}}{=} \mathrm{glue}^{\mathfrak{M}}_{f\in R} l^f_n, \mathrm{glue}^{D_n}_{g\in l^*_n R} \beta^{g;l_n}_n\right)_{n\in\mathbb{N}}).$$

We just need to show that this pair is in $\leq^D$. That is, we need to show that

$$\mathrm{glue}^{\mathfrak{M}}_{f\in R} m^f_n \leq^{\mathfrak{M}} \mathrm{glue}^{\mathfrak{M}}_{f\in R} l^f_n$$

and

$$\mathrm{glue}^{D_n}_{g\in m^*_n R} \alpha^{g;m_n}_n \leq^{D_n} D_n(m_n \leq l_n)(\mathrm{glue}^{D_n}_{g\in l^*_n R} \beta^{g;l_n}_n).$$

The former follows as $\mathfrak{M}$ is an internal poset in $\mathbf{Sh}(C, \mathcal{J})$ by assumption. The latter follows as

$$\begin{aligned} D_n(m_n \leq l_n)(\mathrm{glue}^{D_n}_{g\in l^*_n R} \beta^{g;l_n}_n) &= \mathrm{glue}^{D_n}_{g\in l^*_n R} D_n(m^{g;l_n}_n \leq l^{g;l_n}_n) \beta^{g;l_n}_n \\ &\geq^{D_n} \mathrm{glue}^{D_n}_{g\in l^*_n R} \alpha^{g;l_n}_n, \end{aligned}$$

where we use the fact that $D_n$ is an internal poset in $\mathbf{Sh}(C, \mathcal{J})$.

Next, we can note that $DC$ is an $\omega$-cpo: given $\omega$-chain $\left(\left(U_n^k \xrightarrow{m_n^k} C, \alpha_n^k\right)_{n\in\mathbb{N}}\right)_{k\in\mathbb{N}}$, we define $\left(m_n^\omega, \alpha_n^\omega\right)_{n\in\mathbb{N}}$ by

$$U_n^\omega \xrightarrow{m_n^\omega} C \stackrel{\text{def}}{=} \sup_k (U_n^k \xrightarrow{m_n^k} C)$$
$$\alpha_n^\omega \stackrel{\text{def}}{=} \text{glue}_{k'\in\mathbb{N}} \sup_{k\geq k'}^{D_n} D_n(m_n^{k'} \leq m_n^k)(\alpha_n^k),$$

where we use the fact that $\left(m_n^{k'}\right)_{k'\in\mathbb{N}}$ covers $m_n^\omega = \sup_{k'} m_n^{k'}$. Now, clearly,

$$\begin{aligned} m_n^{k'} &\leq \sup_{k'} m_n^{k'} = m_n^\omega \\ \alpha_n^{k'} &= D_n(\text{id})(\alpha_n^{k'}) \\ &= D_n(m_n^{k'} \leq m_n^{k'})(\alpha_n^{k'}) \\ &\leq \sup_{k\geq k'} D_n(m_n^{k'} \leq m_n^k)(\alpha_n^k) \\ &= D_n(m_n^{k'} \leq m_n^\omega)(\text{glue}_{k'\in\mathbb{N}} \sup_{k\geq k'} D_n(m_n^{k'} \leq m_n^k)(\alpha_n^k)) \\ &= D_n(m_n^{k'} \leq m_n^\omega)(\alpha_n^\omega). \end{aligned}$$

We see that $\left(m_n^{k'}, \alpha_n^{k'}\right)_{n\in\mathbb{N}} \leq \left(m_n^\omega, \alpha_n^\omega\right)_{n\in\mathbb{N}}$ for all $k'$. Further, suppose that $\left(m'_n, \alpha'_n\right)_{n\in\mathbb{N}} \geq \left(m_n^{k'}, \alpha_n^{k'}\right)_{n\in\mathbb{N}}$ for all $k'$. Then,

$$m'_n \geq \sup_{k'} m_n^{k'} = m_n^\omega$$

and we derive the following inequalities

$$\begin{aligned} D_n(m'_n \geq m_n^k)(\alpha'_n) &\geq \alpha_n^k \\ D_n(m_n^{k'} \leq m_n^k)(D_n(m'_n \geq m_n^k)(\alpha'_n)) &\geq D_n(m_n^{k'} \leq m_n^k)(\alpha_n^k) \\ D_n(m'_n \geq m_n^{k'})(\alpha'_n) &\geq D_n(m_n^{k'} \leq m_n^k)(\alpha_n^k) \\ D_n(m'_n \geq m_n^{k'})(\alpha'_n) &\geq \sup_{k\geq k'}^{D_n} D_n(m_n^{k'} \leq m_n^k)(\alpha_n^k) \\ D_n(m_n^{k'} \leq m_n^\omega)(D_n(m'_n \geq m_n^\omega)) &\geq \sup_{k\geq k'}^{D_n} D_n(m_n^{k'} \leq m_n^k)(\alpha_n^k) \\ D_n(m'_n \geq m_n^\omega) &\geq \text{glue}_{k'} \sup_{k\geq k'}^{D_n} D_n(m_n^{k'} \leq m_n^k)(\alpha_n^k), \end{aligned}$$

where we use that $D$ is an $\mathcal{J}$-sheaf of posets, meaning that we can glue inequalities along $\mathcal{J}$-covers. We see that $\left(m_n^\omega, \alpha_n^\omega\right)_{n\in\mathbb{N}}$ is the sup of our $\omega$-chain. It follows that $DC$ is a $\omega$-cpo. Now, we calculate,

using functoriality of $D$, $\omega$-continuity of $D_n(g)$ and $\omega$-continuity of pullback that

$$
\begin{aligned}
&D(f)(\sup^{D}_{k'}\left(m_n^{k'},\alpha_n^{k'}\right)_{n\in\mathbb{N}}) = \\
&D(f)(\left(\sup_{k'} m_n^{k'}, \mathrm{glue}_{k'\in\mathbb{N}} \sup^{D_n}_{k\geq k'} D_n(m_n^{k'}\leq m_n^{k})(\alpha_n^{k})\right)_{n\in\mathbb{N}} = \\
&\left(f^{*}\sup_{k'} m_n^{k'}, D_n(m_n^{*} f)(\mathrm{glue}_{k'\in\mathbb{N}} \sup^{D_n}_{k\geq k'} D_n(m_n^{k'}\leq m_n^{k})(\alpha_n^{k}))\right)_{n\in\mathbb{N}} \\
&\left(\sup_{k'} f^{*} m_n^{k'}, \mathrm{glue}_{k'\in\mathbb{N}} \sup^{D_n}_{k\geq k'} D_n(m_n^{*} f)(D_n(m_n^{k'}\leq m_n^{k})(\alpha_n^{k}))\right)_{n\in\mathbb{N}} \\
&\left(\sup_{k'} f^{*} m_n^{k'}, \mathrm{glue}_{k'} \sup^{D_n}_{k\geq k'} D_n(f^{*}m_n^{k'}\leq f^{*}m_n^{k})(D_n(m_n^{k'*} f)(\alpha_n^{k'}))\right)_{n\in\mathbb{N}} = \\
&\sup^{D}_{k'}\left(f^{*}m_n^{k'}, D_n(m_n^{k'*} f)(\alpha_n^{k'})\right)_{n\in\mathbb{N}} = \\
&\sup^{D}_{k'} D(f)\left(m_n^{k'},\alpha_n^{k'}\right)_{n\in\mathbb{N}}.
\end{aligned}
$$

We see that $D(f)$ is $\omega$-continuous.

Next, we show how to define a cocone $(\mu_n)_{n\in\mathbb{N}}$ on $(i_{n+1} : D_n \rightarrowtail D_{n+1})_{n\in\mathbb{N}}$ with tip $D$. Note that any composition

$$i_{n,k} : D_n \rightarrowtail D_{n+k}$$

of elements of $(i_{n+1})_{n\in\mathbb{N}}$ is an admissible mono as admissible monos are closed under composition. In particular, $i_{n,k}$ has a characteristic function

$$\chi_{i_{n,k}} : D_{n+k} \longrightarrow \mathfrak{M}.$$

Let us formally set $\chi_{i_{n,k}} \stackrel{\mathrm{def}}{=} !_{D_{n+k}};\top$ in case $k \leq 0$. Then, observe that

$$\left(\chi_{i_{k,n-k}} : D_n \longrightarrow \mathfrak{M}\right)_{n\in\mathbb{N}}$$

defines a cocone on the diagram $(i_{n+1} : D_n \rightarrowtail D_{n+1})_{n\in\mathbb{N}}$.

Now, we can define $\mu_n : D_n \longrightarrow D$ as

$$\mu_n(\alpha) \stackrel{\mathrm{def}}{=} \left(\chi_{i_{k,n-k}}(\alpha), D_n(\chi_{i_{k,n-k}}(\alpha))(\alpha)\right)_{k\in\mathbb{N}}.$$

Observe that this is well-defined as

$$
\begin{aligned}
\chi_{i_{k,n-k}}(\alpha) &\leq \chi_{i_{k+1,n-k-1}}(\alpha) \\
\sup_k \chi_{i_{k,n-k}}(\alpha) &= \chi_{i_{n,n-n}}(\alpha) = \mathrm{id} \\
D_n(\chi_{i_{k,n-k}}(\alpha))(\alpha) &\in D_k
\end{aligned}
$$

$$
\begin{aligned}
D_{k+1}(\chi_{i_{k,n-k}}(\alpha)\leq \chi_{i_{k+1,n-k-1}}(\alpha))(D_n(\chi_{i_{k+1,n-k-1}}(\alpha))(\alpha)) &= D_n(\chi_{i_{k,n-k}}(\alpha)\leq \chi_{i_{k+1,n-k-1}}(\alpha))(D_n(\chi_{i_{k+1,n-k-1}}(\alpha))(\alpha)) \\
&= i_{k+1}(D_n(\chi_{i_{k,n-k}}(\alpha))(\alpha)).
\end{aligned}
$$

Observe that $\mu_n$ is full mono as

$$\mu_n(\alpha) = \left(\chi_{i_{k,n-k}}(\alpha), D_n(\chi_{i_{k,n-k}}(\alpha))(\alpha)\right)_{k\in\mathbb{N}}$$

has $\chi_{i_{k,n-k}}(\alpha) = \mathrm{id}$ and $D_n(\chi_{i_{k,n-k}}(\alpha))(\alpha) = \alpha$ for $k = n$. Therefore, $\mu_n(\alpha) \leq \mu_n(\alpha')$, i.e.

$$\left(\chi_{i_{k,n-k}}(\alpha), D_n(\chi_{i_{k,n-k}}(\alpha))(\alpha)\right)_{k\in\mathbb{N}} \leq \left(\chi_{i_{k,n-k}}(\alpha'), D_n(\chi_{i_{k,n-k}}(\alpha'))(\alpha')\right)_{k\in\mathbb{N}}$$

in particular implies (looking at the component $k = n$) that

$$\mathrm{id} \leq \mathrm{id} \text{ and } \alpha = D_n(\mathrm{id})(\alpha) \leq \alpha'.$$

We see that $\alpha \leq \alpha'$.

Then, defining

$$\chi_{\mu_n}((m_k, \alpha_k)_{k\in\mathbb{N}}) \stackrel{\text{def}}{=} m_n,$$

the following square is a pullback:

$$\begin{array}{ccc} D_n & \xrightarrow{!_{D_n}} & \mathbb{1} \\ {\scriptstyle \mu_n}\big\downarrow & \lrcorner & \big\downarrow{\scriptstyle \top} \\ D & \xrightarrow[\chi_{\mu_n}]{} & \mathfrak{M}. \end{array}$$

Indeed, suppose we are given $d : Z \longrightarrow D$ such that $d; \chi_{\mu_n} =!_Z; \top$. Then, writing $d_C(z) = (m_k, \alpha_k)_{k\in\mathbb{N}}$, we have that $m_n = \mathrm{id}_C$ and $\alpha_n \in D_n(C)$. Let us define $u_C(z) = \alpha_n$. Then, we have that

$$\begin{aligned}(\mu_n)_C(u_C(z)) &= \left(\chi_{i_{k,n-k}}(u_C(z)), D_n(\chi_{i_{k,n-k}}(u_C(z)))(u_C(z))\right)_{k\in\mathbb{N}} \\ &= \left(\chi_{i_{k,n-k}}(\alpha_n), D_n(\chi_{i_{k,n-k}}(\alpha_n))(\alpha_n)\right)_{k\in\mathbb{N}}.\end{aligned}$$

For $n \leq k$, observing that $\mathrm{id}_C = m_n \leq m_k$ gives us that $m_k = \mathrm{id}_C$:

$$\begin{aligned}(\chi_{i_{k,n-k}}(\alpha_n), D_n(\chi_{i_{k,n-k}}(\alpha_n))(\alpha_n)) &= (\mathrm{id}_C, D_n(\mathrm{id}_C)(\alpha_n)) \\ &= (\mathrm{id}_C, i_{n,k-n}(\alpha_n)) \\ &= (\mathrm{id}_C, \alpha_k) \\ &= (m_k, \alpha_k).\end{aligned}$$

On the other hand, for $n > k$, observing that $\chi_{i_{k,n-k}}(\alpha_n) = m_n^* m_k = m_k$, we have that

$$\begin{aligned}(\chi_{i_{k,n-k}}(\alpha_n), D_n(\chi_{i_{k,n-k}}(\alpha_n))(\alpha_n)) &= (m_k, D_n(m_k)(\alpha_n)) \\ &= (m_k, \alpha_k).\end{aligned}$$

It now follows that $d = u; \mu_n$ as $\mu_n$ is a full mono. $u$ is unique as $\mu_n$ is mono. Therefore, $\chi_{\mu_n}$ is the characteristic function for $\mu_n$ and $\mu_n$ is an admissible mono.

Next, we show that $(D, \mu)$ is colimiting. Suppose that $(E, \nu)$ is another cocone on $(i_{n+1} : D_n \rightarrowtail D_{n+1})_{n\in\mathbb{N}}$. We construct a unique mediating map $u : D \longrightarrow E$ such that $\mu_n; u = \nu_n$. Indeed, observe that

$$\begin{aligned}D(m_{k'})\,(m_k, \alpha_k)_{k\in\mathbb{N}} &= \left(m_{k'}^* m_k, D_k(m_k^* m_{k'})(\alpha_k)\right)_{k\in\mathbb{N}} \\ &= \begin{pmatrix} \mathrm{id}, D_k(m_{k'} \leq m_k)(\alpha_k) & \text{for } k' \leq k \\ m_k \leq m_{k'}, \alpha_k & \text{for } k' \geq k \end{pmatrix}_{k\in\mathbb{N}} \\ &= \left(\chi_{i_{k,k'-k}}(\alpha_{k'}), D_{k'}(\chi_{i_{k,k'-k}}(\alpha_{k'}))(\alpha_{k'})\right)_{k\in\mathbb{N}} \\ &= \mu_{k'}(\alpha_{k'}).\end{aligned}$$

Now, seeing that $(m_{k'})_{k'\in\mathbb{N}} \in \mathcal{J}$ and $D$ is a $\mathcal{J}$ sheaf, we see that

$$\begin{aligned}u((m_k, \alpha_k)_{k\in\mathbb{N}}) &= u(\mathrm{glue}_{k'} D(m_{k'})\,(m_k, \alpha_k)_{k\in\mathbb{N}}) \\ &= u(\mathrm{glue}_{k'} \mu_{k'}(\alpha_{k'})) \\ &= \mathrm{glue}_{k'} u(\mu_{k'}(\alpha_{k'})) \\ &= \mathrm{glue}_{k'} \nu_{k'}(\alpha_{k'}),\end{aligned}$$

where we use naturality of $u$. We see that $v_{k'}$ uniquely determines $u$. We show that $u$ is natural, using naturality of $v_{k'}$ and the fact that for each $C' \xrightarrow{f} C$, $(f^* m_{k'})_{k' \in \mathbb{N}}$ defines a $\mathcal{J}$-cover of $C'$:

$$\begin{aligned} E(f)(u\,(m_k, \alpha_k)_{k \in \mathbb{N}}) &= E(f)(\mathrm{glue}_{k' \in \mathbb{N}} v_{k'}(\alpha_{k'})) \\ &= \mathrm{glue}_{k' \in \mathbb{N}} E(m_{k'}^* f)(v_{k'}(\alpha_{k'})) \\ &= \mathrm{glue}_{k' \in \mathbb{N}} v_{k'}(D_{k'}(m_{k'}^* f)(\alpha_{k'})) \\ &= u\left(f^* m_k, D_k(m_k^* f)\alpha_k\right)_{k \in \mathbb{N}} \\ &= u(D(f)\,(m_k, \alpha_k)_{k \in \mathbb{N}}). \end{aligned}$$

Next, we show monotonicity of $u$. Suppose that $(m_k, \alpha_k)_{k \in \mathbb{N}} \leq (l_k, \beta_k)_{k \in \mathbb{N}}$. That, is $m_k \leq l_k$ and $\alpha_k \leq D_k(m_k \leq l_k)(\beta_k)$. We show that $u\,(m_k, \alpha_k)_{k \in \mathbb{N}} \leq u\,(l_k, \beta_k)_{k \in \mathbb{N}}$, i.e. $\mathrm{glue}_k v_k(\alpha_k) \leq \mathrm{glue}_k v_k(\beta_k)$. Observe that the fact that $E$ is an internal poset in $\mathbf{Sh}(C, \mathcal{J})$, tells us that it is enough to show that $v_k(\alpha_k) \leq D_k(m_k \leq l_k)(v_k(\beta_k))$, which is true by assumption. Next, we show $\omega$-continuity of $u$, using $\omega$-continuity of $v_k$:

$$\begin{aligned} u(\sup_i\,(m_k^i, \alpha_k^i)_{k \in \mathbb{N}}) &= u(\left(\sup_i m_k^i, \mathrm{glue}_{i'} \sup_{i \geq i'}^{D_k} D_k(m_k^{i'} \leq m_k^i)(\alpha_k^i)\right)_{k \in \mathbb{N}}) \\ &= \mathrm{glue}_{k'} v_{k'}(\mathrm{glue}_{i'} \sup_{i \geq i'}^{D_k} D_k(m_k^{i'} \leq m_k^i)(\alpha_k^i)) \\ &= \mathrm{glue}_{k'} v_{k'}(\sup_i \alpha_{k'}^i) \\ &= \sup_i \mathrm{glue}_{k'} v_{k'}(\alpha_{k'}^i) \\ &= \sup_i u\,(m_k^i, \alpha_k^i)_{k \in \mathbb{N}} \end{aligned}$$

Given any other cocone $(E, v)$ consisting of admissible monos, observe that the characteristic functions $\chi_{v_n}$ form an $\omega$-chain of maps $E \to \mathfrak{M}$. Let us define $\chi_v \stackrel{\text{def}}{=} \sup_n \chi_{v_n}$. We claim that $\chi_v$ is the characteristic map of the mediating morphism $u : D \to E$. Indeed, clearly $\mu_n; u; \chi_v = v_n; \chi_v \geq v_n \chi_{v_n} = !_{D_n}; \top = \mu_n; !_D; \top$. As $\mu_n$ are jointly epimorphic (as is the case for any colimiting cocone, but its universal property) , it follows that $u; \chi_v = !_D; \top$. Further, suppose that $c : Z \to E$ is such that $c; \chi_v = !_Z; \top$. Then, for all $\alpha \in ZC$, $\mathrm{id}_C = (\chi_v)_C(c_C(\alpha)) = \sup_n (\chi_{v_n})_C(c_C(\alpha))$. We see that $(\chi_{v_n})_C(c_C(\alpha)) : U_n^\alpha \to C$ is a cover of $C$. Moreover, $E((\chi_{v_n})_C(c_C(\alpha)))c_C(\alpha) = v_n(\alpha'_n)$ for a unique $\alpha'_n \in D_n U_n^\alpha$. Therefore, $\mu_n(\alpha'_n) \in DU_n^\alpha$. This is easily seen to be a matching family of $D$ for our cover, which lets us define $v : Z \to D$ by $v_C(\alpha) \stackrel{\text{def}}{=} \mathrm{glue}_n \mu_n(\alpha'_n)$. It follows immediately that

$$\begin{aligned} u_C(v_C(\alpha)) &= u_C(\mathrm{glue}_n \mu_n(\alpha'_n)) \\ &= \mathrm{glue}_n u_{U_n^\alpha}(\mu_n(\alpha'_n)) \\ &= \mathrm{glue}_n v_n(\alpha'_n) \\ &= \mathrm{glue}_n E((\chi_{v_n})_C(c_C(\alpha)))c_C(\alpha) \\ &= c_C(\alpha). \end{aligned}$$

$v$ is easily seen to be an $\omega$-continuous natural transformation (using that $v_n$ are full mono). It follows that $\chi_v$ is the characteristic function of $u$, showing that $u$ is an admissible mono.

It now follows that any colimiting cocone consists of admissible monos and that any mediating morphism w.r.t. any colimiting cocone is an admissible mono as any two colimiting cocones are related via canonical isomorphism. Indeed, any isomorphism is an admissible mono (with characteristic function the identity) and admissible monos are closed under composition.

□

*Simple datatypes.* The following axioms equip the domain structure with sufficient structure to interpret the simple type formers (finite products, variants, and function types). We need some care with function types, as in our case these will be effectful function types. Fiore's work lack an axiomatic account of computational effects, which predates the breakthroughs and canonicalisation of monads in the semantic developments of computational effects of the early 2000's (e.g., Levy's Call-by-push-value and Plot kin and Power's Algebraic effects), though it contains almost all the relevant results. We rectify the situation enough to fit our purposes and defer the most general treatment to future work.

*Unit type.* Let $\mathfrak{D}$ be a domain structure. Assume that $C_{\mathfrak{D}}$ has a terminal object $\mathbb{1}$. Then $\mathbb{1}$ is a *partial terminal* object in the category $\mathbf{p}\mathfrak{D}$ of partial maps: for every object $A$ there is a maximal morphism $\top : A \rightharpoonup \mathbb{1}$ w.r.t. the graph order $\subset$, as can be seen from the following diagram:

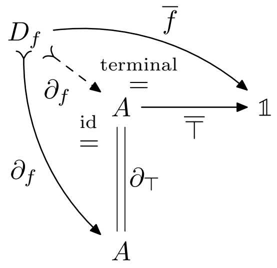


As we can see, $\top = J!$ is in fact total, and is the total terminal morphism. When $\mathfrak{D}$ is a order-enriched, as the order on partial maps contains the graph order, we deduce that $\top$ is maximal w.r.t. the enrichment ordering.

*Product types.* Let $\mathfrak{D}$ be a domain structure. Assume $C_{\mathfrak{D}}$ has a binary product $(A_1 \times A_2, \pi_1, \pi_2)$ for a pair of $C_{\mathfrak{D}}$ objects. Having such a product means we have a pairing operation giving a morphism $(u_1, u_2) : B \to A_1 \times A_2$ for every pair of maps $u_i : B \to A_i$, $i = 1, 2$. We extend this pairing operation to partial maps by setting the partial map $\langle\!\langle u_1, u_2 \rangle\!\rangle : B \rightharpoonup A_1 \times A_2$, for every pair of partial maps $u_i : B \rightharpoonup A_i$, $i = 1, 2$ according to the following diagram:

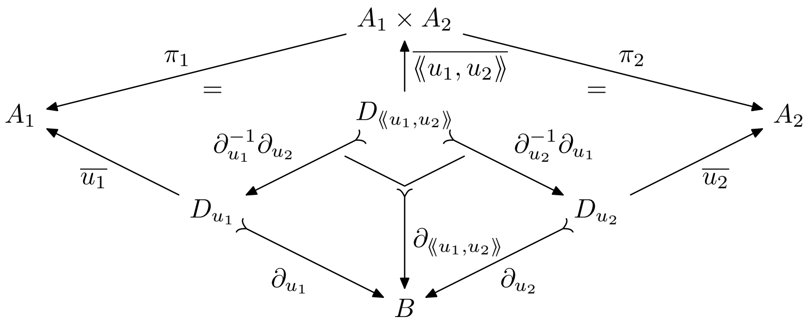

When $C_{\mathfrak{D}}$ has chosen binary products, we extend the resulting cartesian product functor $(\times)$ : $C_{\mathfrak{D}} \times C_{\mathfrak{D}} \to C_{\mathfrak{D}}$ to a functor $(\otimes) : \mathbf{p}\mathfrak{D} \times \mathbf{p}\mathfrak{D} \to \mathbf{p}\mathfrak{D}$ by setting $A_1 \otimes A_2 \stackrel{\text{def}}{=} A_1 \times A_2$ and $f_1 \otimes f_2 \stackrel{\text{def}}{=} \langle\!\langle J\pi_1; f_1, J\pi_2; f_2 \rangle\!\rangle$. The partial pairing $\langle\!\langle -, - \rangle\!\rangle$ is always monotone with respect to the graph order [Fiore 2004, Prop. 5.1.2], and so when $\mathfrak{D}$ is a **Pos**-domain structure, $(\otimes)$ is locally monotone. When $\mathfrak{D}$ is a uniform $\boldsymbol{\omega}$**CPO**-domain structure, $\mathbf{p}\mathfrak{D}$ is $\boldsymbol{\omega}$**CPO**-enriched with respect to the resulting

order, and $- \times A : \mathcal{C}_{\mathfrak{D}} \to \mathcal{C}_{\mathfrak{D}}$ preserves colimits of $\omega$-chains of embeddings, then $(\otimes)$ is locally continuous [Fiore 2004, Prop. 5.1.3].

Proposition 5.10. *The partial-pairing functor resulting from the $\mathfrak{M}$-classifiable $\boldsymbol{\omega}$**CPO**-domain structure is locally continuous.*

Proof. By lemma 5.9, the $\boldsymbol{\omega}\mathbf{CPO}$-domain structure $\mathfrak{D}$ is uniform. By proposition 2.7, $\mathbf{SSh}_{\omega\mathbf{CPO}}(C, \mathcal{J}, \mathcal{K})$ is cartesian closed, and so $- \times A$ is a left adjoint, and hence preserves arbitrary colimits, for every $A \in \mathbf{SSh}_{\omega\mathbf{CPO}}(C, \mathcal{J}, \mathcal{K})$. Therefore $(\otimes)$ is locally continuous. □

*Colimits.* To interpret variant types and recursive types, we will need the existence of certain colimits in the category of partial maps. We first treat them generally, and then specialise to the colimits we require.

Assuming representability ($J \dashv L : \mathbf{p}\mathfrak{D} \to \mathcal{C}_{\mathfrak{D}}$) and a terminal object in $\mathcal{C}_{\mathfrak{D}}$, we can constructs a colimit for $D : I \to \mathbf{p}\mathfrak{D}$ from a colimit for $D; L : I \to \mathcal{C}_{\mathfrak{D}}$ [Fiore 2004, Theorem 5.3.14].

Proposition 5.11. *The category of partial maps is cocomplete.*

Proof. By 5.3, the representability axiom holds, and by proposition 2.7, $\mathbf{SSh}_{\omega\mathbf{CPO}}(C, \mathcal{J}, \mathcal{K})$ is cocomplete and has a terminal object. Therefore every diagram in $\mathbf{p}\mathfrak{D}$ has a colimit. □

*Variants.* Assuming a terminal object, given a diagram $D : I \to \mathcal{C}_{\mathfrak{D}}$ with a colimit for $D; J : I \to \mathbf{p}\mathfrak{D}$, we have that in fact this colimit is in fact total and a colimit for $D$ in $\mathcal{C}_{\mathfrak{D}}$ [Fiore 2004, Prop. 5.2.4]. When the coproducts of $\mathcal{C}_{\mathfrak{D}}$ are $\boldsymbol{\omega}\mathbf{CPO}$-enriched, so are the coproducts in $\mathbf{p}\mathfrak{D}$ [Fiore 2004, Proposition 5.3.13].

As a consequence, the (finite) coproducts of the category of partial maps coincide with those of $\mathbf{SSh}_{\omega\mathbf{CPO}}(C, \mathcal{J}, \mathcal{K})$. For every (finite) set $I$, the locally continuous $I$-indexed coproduct functor $\sum_{i \in I} : \mathbf{SSh}_{\omega\mathbf{CPO}}(C, \mathcal{J}, \mathcal{K})^I \to \mathbf{SSh}_{\omega\mathbf{CPO}}(C, \mathcal{J}, \mathcal{K})$ extends to a locally continuous coproduct functor $\sum_{i \in I} : \mathbf{p}\mathfrak{D}^I \to \mathbf{p}\mathfrak{D}$, given on morphisms by $\sum_{i \in I} f_i \stackrel{\text{def}}{=} [\sum_{i in I} \partial_{f_i}, \sum_{i \in I} \overline{f_i}]$ [Fiore 2004, remark following Corollary 5.3.10].

*Exponentials.* A domain structure with partial products $\mathfrak{D}$ has *partial exponentials* when, for every object $A$, the parial product functor $- \otimes A : \mathcal{C}_{\mathfrak{D}} \to \mathbf{p}\mathfrak{D}$ has a right adjoint $A \rightharpoonup - : \mathbf{p}\mathfrak{D} \to \mathcal{C}_{\mathfrak{D}}$. In that case, we can extend this functor to a functor $- \rightharpoonup - : \mathbf{p}\mathfrak{D}^{\mathrm{op}} \times \mathbf{p}\mathfrak{D} \to \mathbf{p}\mathfrak{D}$ by setting $u \rightharpoonup v : (A \rightharpoonup B) \to (A' \rightharpoonup B')$ to be the adjoint mate of $(A \rightharpoonup B) \otimes A' \xrightarrow{\mathrm{id} \otimes u} (A \rightharpoonup B) \otimes A \xrightarrow{\mathrm{peval}} B \xrightarrow{v} B'$, where $\mathrm{peval} : (A \rightharpoonup B) \otimes A \rightharpoonup B$ is the counit of the adjunction [Fiore 2004, Proposition 5.2.1].

Assuming $\boldsymbol{\omega}\mathbf{CPO}$-enriched representability and $\boldsymbol{\omega}\mathbf{CPO}$-products, all partial exponentials exist, are locally continuous, and given by $A \rightharpoonup B := (B_\perp)^A$ [Fiore 2004, remark following Definition 5.2.3 together with Proposition 5.2.1]. As a consequence:

Proposition 5.12. *The category of partial maps is partially cartesian closed. The partial exponential $- \rightharpoonup - : \mathbf{p}\mathfrak{D}^{\mathrm{op}} \times \mathbf{p}\mathfrak{D} \to \mathbf{p}\mathfrak{D}$ is locally continuous.*

*Recursive types.* The following is a synthesis of Fiore's [Fiore 2004] and Levy's [Levy 2012] books.

When solving recursive domain equations (RDEs) for interpreting programming languages, we define denotations for values in a suitable category of total functions, and when we need to solve recursive domain equations for types, we do so within an expanded category.

Lemma 5.13. *Every partial map embedding is total: let $\mathfrak{D}$ be a* **Pos***-domain structure such that $\mathbf{p}\mathfrak{D}$ is* **Pos***-enriched. For every ep-pair $f : X \leftrightarrows Y$ in $\mathbf{p}\mathfrak{D}^{\mathrm{ep}}$, the embedding part is total $f^{\mathrm{e}} : X \hookrightarrow Y$.*

Proof. By Fiore's Prop. 5.4.2, there is an ep-pair $g : X \leftrightarrows D$ in $\mathcal{C}_{\mathfrak{D}}^{\mathrm{ep}}$, such that $f^{\mathrm{e}} = J(g^{\mathrm{e}}; n)$. □

Lemma 5.14. *Let $\mathfrak{D}$ be a domain structure, $\mathbb{1}$ be terminal and $\mathbb{0}$ be strict initial in $C$. Then the unique $? : \mathbb{0} \longrightarrow \mathbb{1}$ is admissible iff for every $X$, $? : \mathbb{0} \longrightarrow X$ is admissible.*

Proof. The ( $\Longleftarrow$ ) direction is immediate. For the converse, form the following pullback:

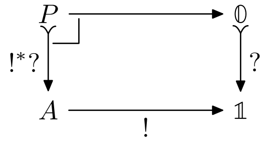


By the strictness of $\mathbb{0}$ and the top arrow, $P \cong \mathbb{0}$, and as the admissible monos are closed under, we conclude. □

Proposition 5.15. *Let $\mathfrak{D}$ be a* **Pos***-domain structure where $C_{\mathfrak{D}}$ is bi-cartesian closed, and $J \dashv L$ is a* **Pos***-adjunction. If the morphism $? : \mathbb{0} \longrightarrow \mathbb{1}$ is an admissible mono, then $\mathbb{0}$ is an ep-zero in* $\mathbf{p}\mathfrak{D}$.

Proof. By Fiore's Prop. 5.3.2(1), $\mathbb{0}$ is strict. By 5.14, $? : \mathbb{0} \longrightarrow X$ is admissible for every $X$. By Fiore's Cor. 5.3.4, $\mathbb{0}$ is a zero object in $\mathbf{p}\mathfrak{D}$. To conclude, we reproduce Fiore's argument (alluded to in his proof of Theorem 8.5.2). Every hom-poset $\mathbf{p}\mathfrak{D}(X, Y)$ has $\bot := [? : \mathbb{0} \rightarrowtail X, ? : \mathbb{0} \rightarrowtail Y]$ as a least element, as $\bot \subset_? u$ for every $u : X \rightharpoonup Y$, and bearing in mind that the order on partial maps contains the graph order:

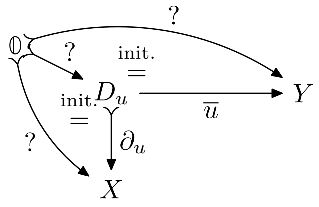


For every $X$, taking $! := [? : \mathbb{0} \rightarrowtail X, \mathrm{id}_{\mathbb{0}}] : X \rightharpoonup \mathbb{0}$, and calculating the composite $X \xrightharpoonup{!} \mathbb{0} \xrightarrow{?} Y$ shows it is $\bot$:

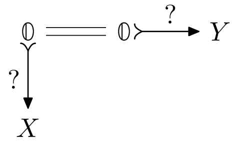


Therefore, by Fiore's Lemma 7.1.2(3) applied once to $\mathbf{p}\mathfrak{D}$ and once to $\mathbf{p}\mathfrak{D}^{\mathrm{op}}$, we have that $\mathbb{0}$ is an ep-zero in $\mathbf{p}\mathfrak{D}$. □

Theorem 5.16 (bilimit compact expansion via partial maps). *Let $\mathfrak{D}$ be a* $\omega$**CPO***-domain structure where:*

- *$C_{\mathfrak{D}}$ is bi-cartesian closed;*
- *$C_{\mathfrak{D}}$ has $\omega$-colimits of embeddings; and*
- *$\mathbf{p}\mathfrak{D}$ is* **Pos***-enriched and $J \dashv L$ is a* **Pos***-adjunction.*

*If the morphism $? : \mathbb{0} \longrightarrow \mathbb{1}$ is an admissible mono, then $J : C \longrightarrow \mathbf{p}\mathfrak{D}$ is a bilimit compact expansion.*

Proof. By 5.15, $\mathbb{0}$ is an ep-zero object in $\mathbf{p}\mathfrak{D}$. As we saw, the enrichment assumptions imply that $\mathbf{p}\mathfrak{D}$ is $\omega$**CPO**-enriched and $J : C \longrightarrow \mathbf{p}\mathfrak{D}$ is locally continuous and faithful. Fiore's Prop. 4.1.3 shows $J$ reflects the order. Fiore's Prop. 5.4.4, the assumption that $C$ has a terminal object, and the assumption on $\omega$-colimits in $C$ imply that $\mathbf{p}\mathfrak{D}$ has $\omega$-colimits of embeddings, and so $\mathbf{p}\mathfrak{D}$ is bilimit compact. To conclude, we need to show the closure condition of $J$ under mediating morphisms.

Consider the data as in the closure condition. By 5.13, the $\omega$-chains of embeddings $A^e$ and $B^e$ and the embedding cocones $D^e$ and $E^e$ lie in $C$ and by the limit-colimit coincidence, $JD$ and $JE$ are their colimits in $\mathbf{p}\mathfrak{D}$. Because $C$ has a terminal object, by Fiore's Prop. 5.2.4, the inclusion $J$ reflects colimits, and so $D$ and $E$ are in fact colimits in $C$. Because $\alpha$ lies in $C$ and natural w.r.t. the embedding diagrams, we have a mediating $A$-cocone morphism $m : D \to E$. Applying $J$, we have that $Jm$ is mediating, hence equal to $\mu$. □

Corollary 5.17 (Bilimit Compactness $\mathbf{SSh}_{\omega\mathbf{CPO}}(\mathcal{C},\mathcal{J},\mathcal{K})_\perp$). *The Kleisli adjunction* $\mathbf{SSh}_{\omega\mathbf{CPO}}(\mathcal{C},\mathcal{J},\mathcal{K}) \leftrightarrows \mathbf{SSh}_{\omega\mathbf{CPO}}(\mathcal{C},\mathcal{J},\mathcal{K})_\perp$ *gives a bilimit compact expansion that supports locally continuous (partial) finite products and coproducts and exponentials. In particular, it gives a sound model of FPC.*

In particular, we see that $\omega\mathbf{Diff} \to \omega\mathbf{Diff}_\perp$ and $\omega\mathbf{Qbs} \to \omega\mathbf{Qbs}_\perp$ are bilimit compact expansions. In the former, the admissible monos are easily seen to coincide with the *D-Scott open monos*: monos whose image is open in the D-topology of the diffeology as well as Scott open. In the latter, the admissible monos coincide with the *Borel-Scott open monos*: monos whose image is measurable in the canonical measurable space structure on the quasi-Borel space as well as Scott open.

Corollary 5.18 (Soundness). *$Sh_{\omega\mathbf{CPO}}(\mathcal{C},\mathcal{J},\mathcal{K})$ gives a sound model of FPC. That is, if $t$ evaluates to $v$ in the operational semantics, then $[\![t]\!] = [\![v]\!]$ for the canonical interpretation $[\![-]\!]$ in $Sh_{\omega\mathbf{CPO}}(\mathcal{C},\mathcal{J},\mathcal{K})$.*

Proof. This follows from [Fiore 2004, Theorem 9.1.4]. □

Lemma 5.19 (Absoluteness). *If we assume that $C$ has a terminal object $\mathbb{1}$ such that $\mathfrak{M}\mathbb{1}$ is finite (or, more generally, the top element of $\mathfrak{M}\mathbb{1}$ is inaccessible by lubs of $\omega$-chains), then the domain structure is absolute in the sense that* $\mathbf{Sh}_{\omega\mathbf{CPO}}(\mathcal{C},\mathcal{J},\mathcal{K})(\mathbb{1},F)$ *is inaccessible by lubs of $\omega$-chains in* $\mathbf{Sh}_{\omega\mathbf{CPO}}(\mathcal{C},\mathcal{J},\mathcal{K})(\mathbb{1},F_\perp)$.

Proof. By [Fiore 2004, Proposition 9.2.11], as we are working with a domain theoretic model of FPC, it is enough to show that $\mathrm{id}_{\mathbb{1}}$ is inaccessible in in the $\omega$-cpo of admissible subobjects of $\mathbb{1}$. Note that the $\omega$-cpo of admissible subobjects of $\mathbb{1}$ is precisely $\mathbf{Nat}(\mathbb{1},\mathfrak{M}) = \mathbf{Nat}(\mathbf{y}_{\mathbb{1}},\mathfrak{M}) = \mathfrak{M}\mathbb{1}$, by the Yoneda lemma. Finally, if $\mathfrak{M}\mathbb{1}$ is finite, its top element is clearly inaccessible by lubs of $\omega$-chains. □

Corollary 5.20 (Adequacy). *If we assume that $C$ has a terminal object $\mathbb{1}$ such that $\mathfrak{M}\mathbb{1}$ is finite and not a singleton, then $Sh_{\omega\mathbf{CPO}}(\mathcal{C},\mathcal{J},\mathcal{K})$ gives an adequate model of FPC. That is, if $t$ diverges in the operational semantics, then $[\![t]\!] = \perp$ in the denotational semantics.*

Proof. This follows from the previous lemma by [Fiore 2004, Theorem 9.2.19]. □

This is, in particular, the case for $\omega\mathbf{Qbs}$ and $\omega\mathbf{Diff}$.

## 6 TWO ORTHOGONAL FACTORIZATION SYSTEMS ON $\mathbf{SSh}_{\omega\mathbf{CPO}}(\mathcal{C},\mathcal{J},\mathcal{K})$

Recall the definition of an orthogonal factorization system, which we phrase slightly abstractly in order to be able to enrich it.

*Definition 6.1 ($\mathcal{V}$-Enriched Orthogonal Factorization System).* A *$\mathcal{V}$-enriched orthogonal factorization system* $(\mathcal{E},\mathcal{M})$ on a $\mathcal{V}$-enriched category $C$ consists of

- two $\mathcal{V}$-enriched full subcategories $\mathcal{E},\mathcal{M}$ of the $\mathcal{V}$-enriched arrow category $C/C$, such that their objects contain all isomorphisms and are closed under composition;
- a $\mathcal{V}$-enriched functor factor : $C/C \to \mathcal{E} \rtimes \mathcal{M}$, such that

$$\mathrm{factor};\mathrm{comp} = \mathrm{id}_{C/C} \qquad \mathrm{comp};\mathrm{factor} \cong \mathrm{id}_{\mathcal{E}\rtimes\mathcal{M}},$$

where we write $\mathcal{E} \rtimes \mathcal{M}$ for the $\mathcal{V}$-enriched pullback category of $\mathcal{E} \xrightarrow{\text{cod}} C$ and $\mathcal{M} \xrightarrow{\text{dom}} C$ and comp for the natural $\mathcal{V}$-enriched functor $\mathcal{E} \rtimes \mathcal{M} \to C/C$ which performs composition on objects.

It is an easy exercise to verify that this gives us back the usual notion of orthogonal factorization system in the case that $\mathcal{V} = \mathbf{Set}$. We will be particularly interested in the case of $\mathcal{V} = \boldsymbol{\omega}\mathbf{CPO}$. In more elementary terms, a $\boldsymbol{\omega}\mathbf{CPO}$-enriched orthogonal factorization system $(\mathcal{E}, \mathcal{M})$ on $C$ is equivalent to the following data:

- $\mathcal{E}$ is a lluf subcategory of $C$, containing all isomorphisms;
- $\mathcal{M}$ is a lluf subcategory of $C$, containing all isomorphisms;
- every morphism $f : X \to Z$ in $C$ factors as $f = e; m$ for some $e \in \mathcal{E}$ and $m \in \mathcal{M}$;
- in case $e; m; g_2 = g_1; e'; m'$, for $e, e' \in \mathcal{E}$ and $m, m' \in \mathcal{M}$, there exists a unique $h$ such that $e; h = g_1; e'$ and $h; m' = m; g_2$ (as shown below) and function $(g_1, g_2) \mapsto h$ is $\omega$-continuous.

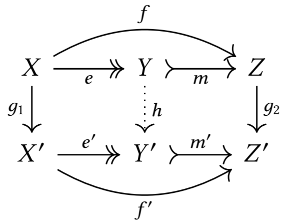


Corollary 6.2. *For a $\mathcal{V}$-enriched orthogonal factorization system $(\mathcal{E}, \mathcal{M})$ on $C$, $\mathcal{E}$ is a $\mathcal{V}$-enriched full coreflective subcategory of $C/C$ and $\mathcal{M}$ is a $\mathcal{V}$-enriched full reflective subcategory of $C/C$.*

Proof. This is clearly true if we replace $C/C$ with the equivalent $\mathcal{V}$-category $\mathcal{E} \rtimes \mathcal{M}$. □

Given a $B \in \mathbf{SSh}_{\omega\mathbf{CPO}}(C, \mathcal{J}, \mathcal{K})$, we define a closure operation $\mathrm{Cl}_{\mathcal{K}}$ on (not necessarily chain complete) subpresheaves $A$ in $\mathbf{PSh}(C)$, called the *$\mathcal{K}$-closure*: we take the closure under amalgamations of matching families for $\mathcal{K}$-covers which exist in $B$, i.e.

$$(\mathrm{Cl}_{\mathcal{K}} A)C \stackrel{\text{def}}{=} \left\{ \beta \in BC \mid \exists R \in \mathcal{K}C. \forall C_f \xrightarrow{f} C \in R. B(f)(\beta) \in AC_f \right\}.$$

We can similarly define the (smaller) *$\mathcal{J}$-closure*: we take the closure under amalgamations of matching families for $\mathcal{J}$-covers which exist in $B$ (i.e. $(\mathrm{Cl}_{\mathcal{J}} A)C \stackrel{\text{def}}{=} \left\{ \beta \in BC \mid \exists R \in \mathcal{J}C. \forall C_f \xrightarrow{f} C \in R. B(f)(\beta) \in AC_f \right\}$)
Finally, we can also define the *full $\omega$-chain-closure* $\mathrm{Cl}_{\omega} A$ of $A$ in $B$ as the smallest pointwise chain-complete subpresheaf of $B$ containing $A$ (under order induced by $B$ which makes $\mathrm{Cl}_{\omega} A$ a full subpresheaf of $B$). This $\omega$-chain-closure is well-studied and is widely known to exist (and can be constructed predicatively by a transfinite recursion, adding sups of any existing $\omega$-chains, until the construction stabilises).

Given a closure operator Cl, we call a subpresheaf $A$ of $B$ Cl-closed if $\mathrm{Cl}A = \mathrm{Cl}$. We define a composite closure operator $\mathrm{Cl}_{\omega\mathcal{K}}$ on subpresheaves $A$ of $B$ as sending $A$ to the smallest subpresheaf of $B$ containing $A$ that is both $\mathrm{Cl}_{\mathcal{K}}$-closed and $\mathrm{Cl}_{\omega}$-closed. We define $\mathrm{Cl}_{\omega\mathcal{J}}$ similarly, by replacing $\mathcal{K}$ with $\mathcal{J}$.

Lemma 6.3. *Given a $P \in \mathbf{SSh}_{\omega\mathbf{CPO}}(C, \mathcal{J}, \mathcal{K})$, for each subobject $m : A \hookrightarrow P$ in $\mathbf{PSh}(C)$, we have well-defined $\mathrm{Cl}_{\omega\mathcal{J}}(m)$, $\mathrm{Cl}_{\omega\mathcal{K}}(m)$ such that $m \leq \mathrm{Cl}_{\omega\mathcal{J}}(m) \leq \mathrm{Cl}_{\omega\mathcal{K}}(m)$.*

Proof. We first note that the set of $\mathcal{K}$-closed subobject containing $m$ is not empty as it contains $\mathrm{id}_P$. Next, we observe that any pointwise intersection (wide pullback) of full $\mathcal{K}$-closed subobject

is a full $\mathcal{K}$-closed mono. Therefore, we can define $\mathrm{Cl}_{\omega\mathcal{K}}(m)$ as the wide pullback of all $\mathcal{K}$-closed subobject containing $m$.

$\mathrm{Cl}_{\omega\mathcal{J}}(m)$ is defined analogously. Observing that any $\mathcal{K}$-closed subobject is also $\mathcal{J}$-closed (as $\mathcal{J} \subseteq \mathcal{K}$), it follows that $\mathrm{Cl}_{\omega\mathcal{J}}(m) \leq \mathrm{Cl}_{\omega\mathcal{K}}(m)$. □

As an alternative to the impredicative definition above, we can also equivalently construct the full $\mathcal{K}$-closure (and full $\mathcal{J}$-closure) predicatively as follows.

Lemma 6.4. *Given a $P \in \mathbf{SSh}_{\omega\mathbf{CPO}}(C, \mathcal{J}, \mathcal{K})$ and a subobject $m : A \hookrightarrow P$ in $\mathbf{PSh}(C)$, we can define the following ordinal indexed increasing sequence of subobjects of $P$, using transfinite recursion,*

$$A_0 \overset{\text{def}}{=} A$$

$$A_{S(\alpha)} \mid S(\alpha) \text{ a succesor ordinal} \overset{\text{def}}{=} \mathrm{Cl}_\omega \mathrm{Cl}_{\mathcal{K}} A_\alpha$$

$$A_\beta \mid \beta \text{ a limit ordinal} \overset{\text{def}}{=} \mathrm{Cl}_\omega \mathrm{Cl}_{\mathcal{K}} \cup_{\alpha<\beta} A_\alpha .$$

*Then, this sequence stabilises at some ordinal. The value it stabilises at is $\mathrm{Cl}_{\omega\mathcal{K}}A$.*

*$\mathrm{Cl}_{\omega\mathcal{J}}A$ can be constructed similarly if one replaces $\mathcal{K}$ with $\mathcal{J}$.*

Proof. The operations $\mathrm{Cl}_{\mathcal{K}}$ and $\mathrm{Cl}_\omega$ have the property that $A' \leq \mathrm{Cl}_{\mathcal{K}}A'$ and $A'' \leq \mathrm{Cl}_\omega A''$. Therefore, this defines an increasing sequence.

Moreover, suppose that $A_{S(\alpha)} = A_\alpha$ for some $\alpha$. Then, by transfinite induction, $A_\alpha = A_{\alpha'}$ for any $\alpha' \geq \alpha$. Indeed, $A_\alpha = A_\alpha$ and suppose that $A_\alpha = A_{\alpha''}$ for all $\alpha'' < \alpha'$. Then, $\alpha''$ is either a successor ordinal $S\alpha'''$, in which case $A_{\alpha''} = A_{S\alpha'''} = \mathrm{Cl}_\omega\mathrm{Cl}_{\mathcal{K}}A_{\alpha'''} = \mathrm{Cl}_\omega\mathrm{Cl}_{\mathcal{K}}A_\alpha = A_{S(\alpha)} = A_\alpha$, or it is a limit ordinal, in which case $A_{\alpha''} = \mathrm{Cl}_\omega\mathrm{Cl}_{\mathcal{K}} \bigcup_{\alpha'''<\alpha''} A_{\alpha'''} = \mathrm{Cl}_\omega\mathrm{Cl}_{\mathcal{K}} \bigcup_{\alpha'''<\alpha''} A_\alpha = \mathrm{Cl}_\omega\mathrm{Cl}_{\mathcal{K}}A_\alpha = A_{S\alpha} = A_\alpha$. That is, once the sequence stabilises, it remains stabilised.

Suppose that the sequence does not stabilise until the ordinal $\beta$. Then, $A\_$ is an injection from $\beta$ to the powerset of $| \cup_{C\in C} PC|$. Therefore, the sequence must stabilise at some ordinal $\beta$ of cardinality $\leq 2^{| \cup_{C\in C} PC|}$.

At this point, we have that $\mathrm{Cl}_\omega\mathrm{Cl}_{\mathcal{K}}A_\beta = A_\beta$. So, in particular, as both closure operators are increasing, $\mathrm{Cl}_{\mathcal{K}}A_\beta = A_\beta$ and so also $\mathrm{Cl}_\omega A_\beta = \mathrm{Cl}_\omega\mathrm{Cl}_{\omega\mathcal{K}}A_\beta = A_\beta$. We see that $A_\beta$ is both closed under sups of $\omega$-chains and under amalgamations which exist in $P$ of matching families w.r.t. $\mathcal{K}$-covers. That is, $A_\beta$ is $\mathrm{Cl}_{\omega\mathcal{K}}$-closed. This shows that $\mathrm{Cl}_{\omega\mathcal{K}}A \subseteq A_\beta$.

Conversely, observe that by transfinite induction, it follows that $A_\gamma \subseteq \mathrm{Cl}_{\omega\mathcal{K}}A$ for any ordinal $\gamma$. Therefore, $A_\beta \subseteq \mathrm{Cl}_{\omega\mathcal{K}}A$.

Precisely the same argument works if we replace $\mathcal{K}$ with $\mathcal{J}$. □

Lemma 6.5 (Functoriality of $\mathrm{Cl}_{\omega\mathcal{K}}$ and $\mathrm{Cl}_{\omega\mathcal{J}}$). *Given $B, B' \in \mathbf{SSh}_{\omega\mathbf{CPO}}(C, \mathcal{J}, \mathcal{K})$, $A, A' \in \mathbf{PSh}(C)$ (possibly non-full) subpresheaves of $B$ and $B'$ respectively, and $b : B \to B'$ an $\omega$-continuous natural transformation which restricts to $a : A \to A'$ as in the diagram below:*

$$\begin{array}{ccccc} A & \overset{i}{\rightarrowtail} & \mathrm{Cl}_{\omega\mathcal{K}}A & \overset{j}{\rightarrowtail} & B \\ {\scriptstyle a}\downarrow & & \downarrow{\scriptstyle \mathrm{Cl}_{\omega\mathcal{K}}a} & & \downarrow{\scriptstyle b} \\ A' & \underset{i'}{\rightarrowtail} & \mathrm{Cl}_{\omega\mathcal{K}}A' & \underset{j'}{\rightarrowtail} & B' \end{array}$$

*Then, $b$ also restricts to a morphism $\mathrm{Cl}_{\omega\mathcal{K}}a : \mathrm{Cl}_{\omega\mathcal{K}}A \to \mathrm{Cl}_{\omega\mathcal{K}}A'$.*

*Similarly, $b$ also restricts to a morphism $\mathrm{Cl}_{\omega\mathcal{J}}a : \mathrm{Cl}_{\omega\mathcal{J}}A \to \mathrm{Cl}_{\omega\mathcal{J}}A'$.*

Proof. We work with the predicative construction of $\mathrm{Cl}_{\omega\mathcal{K}}A$ given by lemma 6.4.

Now, by $\omega$-chain completeness of $\mathrm{Cl}_{\omega\mathcal{K}}A'$ and the fact that $\mathrm{Cl}_{\omega\mathcal{K}}A'$ contains all amalgamations of matching families w.r.t. $\mathcal{K}$-covers which exist in $B'$, $j; b$ restricts to $\mathrm{Cl}_{\omega\mathcal{K}}A'$. To be precise, this

follows by the following transfinite recursive construction. Clearly, $b$ restricts as $a_0 \stackrel{\text{def}}{=} a; i' : A_0 = A \to \mathrm{Cl}_{\omega\mathcal{K}}A'$. Let us turn to successor ordinals. Supposing that $b$ restricts to $a_\alpha : A_\alpha \to \mathrm{Cl}_{\omega\mathcal{K}}A'$, we have, by the fact that $\mathrm{Cl}_{\omega\mathcal{K}}A'$ contains all amalgamations of matching families w.r.t. $\mathcal{K}$-covers which exist in $B'$, that $b$ restricts to a unique $a'_\alpha : \mathrm{Cl}_{\mathcal{K}}A_\alpha \to \mathrm{Cl}_{\omega\mathcal{K}}A'$. (Indeed, suppose that $\gamma \in \mathrm{Cl}_{\mathcal{K}}A_\alpha C$. Then, $\gamma \in BC$ and there exists some $R \in \mathcal{K}C$ such that $B(f)(\gamma) \in A_\alpha C_f$ for all $C_f \xrightarrow{f} C \in R$. Therefore, by naturality of $b$, $b(\gamma) = \mathrm{glue}\,(b(\gamma_f))_{f\in R} = \mathrm{glue}\,(a_\alpha(\gamma_f))_{f\in R} \in \mathrm{Cl}_{\omega\mathcal{K}}A'$ as $\mathrm{Cl}_{\omega\mathcal{K}}A'$ is closed under amalgamations of matching families w.r.t. $\mathcal{K}$-covers which exist in $B'$. ) Further, $b$ restricts to a unique $a_{S(\alpha)} \stackrel{\text{def}}{=} {a'_\alpha}^\dagger : A_{S(\alpha)} = \mathrm{Cl}_\omega\mathrm{Cl}_{\mathcal{K}}A_\alpha \to \mathrm{Cl}_{\omega\mathcal{K}}A'$ as $b$ is $\omega$-continuous and it restricts to a unique $a'_\alpha : \mathrm{Cl}_{\mathcal{K}}A_\alpha \to \mathrm{Cl}_{\omega\mathcal{K}}A'$, while $\mathrm{Cl}_{\omega\mathcal{K}}A'$ is $\omega$-chain closed. Finally, at limit ordinals $\beta$, $b$ restricts to $a_\beta \stackrel{\text{def}}{=} (\cup_{\alpha<\beta}a_\alpha)'^\dagger$.

Precisely the same argument works for $\mathrm{Cl}_{\omega\mathcal{J}}$ if we replace $\mathcal{K}$ with $\mathcal{J}$. □

Given a closure operator Cl, we call a subobject $m : A \to P$ Cl-*dense* if $\mathrm{Cl}(m) = \mathrm{id}_P$. More generally, we call a morphism $f : P \to Q$ in $\mathbf{SSh}_{\omega\mathbf{CPO}}(C, \mathcal{J}, \mathcal{K})$ Cl-*dense* if its pointwise image is a Cl-dense subpresheaf of $Q$.

We note that we have a natural orthogonal factorization systems on categories of $\omega$-cpos in Grothendieck quasitoposes.

Theorem 6.6 (Factorization System 1 on $\mathbf{SSh}(C, \mathcal{J}, \mathcal{K})$). *For any category* $\mathbf{SSh}_{\omega\mathbf{CPO}}(C, \mathcal{J}, \mathcal{K})$ *of $\omega$-cpos in a Grothendieck quasitopos, choosing*

- $\mathrm{Cl}_{\omega\mathcal{K}}$*-dense morphisms as* $\mathcal{E}$*;*
- $\mathrm{Cl}_{\omega\mathcal{K}}$*-closed monos as* $\mathcal{M}$ *(or equivalently, morphisms which are strong monos in* $\mathbf{SSh}(C, \mathcal{J}, \mathcal{K})$ *and componentwise full);*

*defines a* $\omega$**CPO**-*enriched orthogonal factorization system* $(\mathcal{E}, \mathcal{M})$ *on* $\mathbf{SSh}_{\omega\mathbf{CPO}}(C, \mathcal{J}, \mathcal{K})$.

Proof. Observe that $\mathrm{Cl}_{\omega\mathcal{K}}$-closed monos $m : X \hookrightarrow Y$ between objects of $\mathbf{SSh}_{\omega\mathbf{CPO}}(C, \mathcal{J}, \mathcal{K})$ are precisely fully embedded $\omega$-chain-closed subpresheaves $X$ of $Y$ which are closed under any amalgamations of matching $\mathcal{K}$-families which exist in $Y$. Clearly, $\mathrm{Cl}_{\omega\mathcal{K}}$-closed monos contain all isomorphisms as isomorphisms are full and closed under any amalgamations which exist in their codomain. Now, suppose that $m : X \hookrightarrow Y$ and $n : Y \hookrightarrow Z$ are $\mathrm{Cl}_{\omega\mathcal{K}}$-closed monos. Clearly full monos compose, so $m; n$ consists of full monos in each component. Now, $X$ is $\omega$-chain closed by assumption. So the only thing to check is that $X$ is closed under any amalgamations of matching families which exist in $Z$. Let $R \in \mathcal{K}C$ and let $\gamma \in ZC$. Suppose that $Z(f)(\gamma) \in XC_f$ for each $C_f \xrightarrow{f} C \in R$. Then, in particular, $Z(f)(\gamma) \in YC_f$. Therefore, as $Y$ is $\mathrm{Cl}_{\omega\mathcal{K}}$-closed (and therefore $\mathrm{Cl}_{\mathcal{K}}$-closed) in $Z$, we have that $\gamma \in YC$. Now, $Y(f)(\gamma) = Z(f)(\gamma) \in XC_f$, so as $X$ is $\mathrm{Cl}_{\omega\mathcal{K}}$-closed (and therefore $\mathrm{Cl}_{\mathcal{K}}$-closed) in $Y$, it follows that $\gamma \in XC$.

Clearly, $\mathrm{Cl}_{\omega\mathcal{K}}$-dense morphisms contain all isomorphisms as isomorphisms have the identity as image inclusion. $\mathcal{E}$ is closed under composition: suppose we are given $\mathrm{Cl}_{\omega\mathcal{K}}$-dense morphisms $X \xrightarrow{f} Y \xrightarrow{g} Z$. Then,

$$\begin{aligned}\mathrm{Cl}_{\omega\mathcal{K}}\mathrm{Im}\,(f;g) &= \mathrm{Cl}_{\omega\mathcal{K}}g[\mathrm{Im}\,(f)] \\ &\quad \text{as } g \text{ is } \omega\text{-continuous and natural} \\ &\downarrow \\ &= \mathrm{Cl}_{\omega\mathcal{K}}g[\mathrm{Cl}_{\omega\mathcal{K}}\mathrm{Im}\,(f)] \\ &= \mathrm{Cl}_{\omega\mathcal{K}}g[Y] \\ &= \mathrm{Cl}_{\omega\mathcal{K}}\mathrm{Im}\,(g) \\ &= Z.\end{aligned}$$

We see that $f; g$ is $\mathrm{Cl}_{\omega\mathcal{K}}$-dense.

Suppose we are given $f : X \to Y$ in $\mathbf{SSh}_{\boldsymbol{\omega}\mathbf{CPO}}(C, \mathcal{J}, \mathcal{K})$. Using the usual image factorization on **Set** in each component, we can construct a factorization of $f = e; m$ where $e : X \to \mathrm{Im}\,(f)$ goes to the presheaf of $\omega$-cpos which is the (pointwise) image of $f$ and $m$ is the (pointwise) inclusion of the image in $Y$ which is a non-full mono. In particular, $\mathrm{Im}\,(f)$ is not an object of $\mathbf{SSh}_{\boldsymbol{\omega}\mathbf{CPO}}(C, \mathcal{J}, \mathcal{K})$ but merely an object of $\mathbf{PSh}(C)$. We can close it in $B$ using $\mathrm{Cl}_{\omega\mathcal{K}}$ to get an object of $\mathbf{SSh}_{\boldsymbol{\omega}\mathbf{CPO}}(C, \mathcal{J}, \mathcal{K})$, however. Given, another $f'$, $x$ and $y$ as below, we get a restriction of $y$ to $\mathrm{Im}\,((x, y)) : \mathrm{Im}\,(f) \to \mathrm{Im}\,(f')$, using the usual image factorizations on **Pos** in each component. By lemma 6.5, we now get a (unique) restriction of $y$ to an $\omega$-continuous natural transformation $\mathrm{Cl}_{\omega\mathcal{K}}(x, y)$ as below.

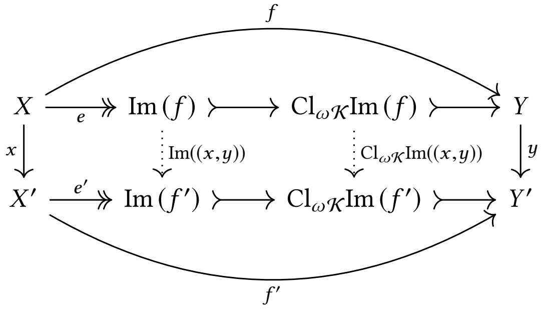


The description of $\mathrm{Cl}_{\omega\mathcal{K}}$-closed monos as strong full monos follows once we note that a mono is $\mathrm{Cl}_{\omega\mathcal{K}}$-closed iff it is both $\mathrm{Cl}_{\mathcal{K}}$-closed and $\mathrm{Cl}_{\omega}$-closed. $\mathrm{Cl}_{\mathcal{K}}$-closed monos are well-known (see e.g. [Johnstone 2002], Example A2.6.4(d)) to correspond to strong monos in $\mathbf{SSh}(C, \mathcal{J}, \mathcal{K})$. $\mathrm{Cl}_{\omega}$-closed monos are clearly precisely componentwise full monos in $\boldsymbol{\omega}\mathbf{CPO}$. □

Theorem 6.7 (Factorization System 2 on $\mathbf{SSh}(C, \mathcal{J}, \mathcal{K})$). *For any category* $\mathbf{SSh}_{\boldsymbol{\omega}\mathbf{CPO}}(C, \mathcal{J}, \mathcal{K})$ *of $\omega$-cpos in a Grothendieck quasitopos, choosing*

- $\mathrm{Cl}_{\omega\mathcal{J}}$*-dense morphisms as* $\mathcal{E}$*;*
- $\mathrm{Cl}_{\omega\mathcal{J}}$*-closed monos as* $\mathcal{M}$ *(or equivalently, morphisms which are monos in* $\mathbf{SSh}(C, \mathcal{J}, \mathcal{K})$*, i.e. componentwise injective, and componentwise full);*

*defines a* $\boldsymbol{\omega}\mathbf{CPO}$*-enriched orthogonal factorization system* $(\mathcal{E}, \mathcal{M})$ *on* $\mathbf{SSh}_{\boldsymbol{\omega}\mathbf{CPO}}(C, \mathcal{J}, \mathcal{K})$*.*

Proof. This is entirely analogous to the previous proof.

The description of $\mathrm{Cl}_{\omega\mathcal{J}}$-closed monos as strong full monos follows once we note that a mono is $\mathrm{Cl}_{\omega\mathcal{J}}$-closed iff it is both $\mathrm{Cl}_{\mathcal{J}}$-closed and $\mathrm{Cl}_{\omega}$-closed. Clearly, every mono in $\mathbf{SSh}(C, \mathcal{J}, \mathcal{K})$ is $\mathrm{Cl}_{\mathcal{J}}$-closed as the domain is a $\mathcal{J}$-sheaf. $\mathrm{Cl}_{\omega}$-closed monos are clearly precisely componentwise full monos in $\boldsymbol{\omega}\mathbf{CPO}$.

To see that the factorization is $\boldsymbol{\omega}\mathbf{CPO}$-enriched, note that $\mathrm{Cl}_{\omega\mathcal{K}}\mathrm{Im}\,((x, y))$ depends $\omega$-continuously on $y$ (hence on $(x, y)$) seeing that it is the restriction of $y$ between two *full* subpresheaves of the domain and codomain. □

Observe that on the category of quasi-Borel predomains we have worked with the ($\mathrm{Cl}_{\omega\mathcal{J}}$-dense morphisms, $\mathrm{Cl}_{\omega\mathcal{J}}$-closed monos)- factorization system in [Vákár et al. 2019] to construct a probabilistic powerdomain.

Both these factorization system has the following nice properties that make them suitable for constructing subscones for logical relations arguments over pure languages.

Proposition 6.8. *For the factorization systems* $(\mathcal{E}, \mathcal{M})$ *of (*$\mathrm{Cl}_{\omega\mathcal{K}}$*-dense morphisms,* $\mathrm{Cl}_{\omega\mathcal{K}}$*-closed monos) and (*$\mathrm{Cl}_{\omega\mathcal{J}}$*-dense morphisms,* $\mathrm{Cl}_{\omega\mathcal{J}}$*-closed monos) on* $\mathbf{SSh}_{\boldsymbol{\omega}\mathbf{CPO}}(C, \mathcal{J}, \mathcal{K})$*,* $\mathcal{E}$ *and* $\mathcal{M}$ *are closed under products.*

Proof. This follows as $\mathrm{Cl}_{\omega\mathcal{K}}(\prod_i A_i) = \prod_i \mathrm{Cl}_{\omega\mathcal{K}} A_i$ and $\mathrm{Cl}_{\omega\mathcal{J}}(\prod_i A_i) = \prod_i \mathrm{Cl}_{\omega\mathcal{J}} A_i$ for $A_i \subseteq B_i$, (indeed, the product order and lubs are componentwise; and amalgamations of matching families of product presheaves are componentwise;) while also $\mathrm{Im}\,(\prod_i f_i) = \prod_i \mathrm{Im}\,(f_i)$. □

As is standard, it follows that $\mathcal{M}$ is closed under exponentiation.

In case we want to use a factorization system to construct a subscone for logical relations arguments over languages with recursive types, it is natural to demand one more condition of a factorization system: compatibility with a bilimit compact expansion.

*Definition 6.9 ($\mathcal{J}$-Compatible Orthogonal Factorization System).* Given a bilimit compact expansion $\mathcal{J} : \mathcal{V} \hookrightarrow C$, a $\boldsymbol{\omega}$**CPO**-enriched factorization system on $C$ is called a *$\mathcal{J}$-compatible orthogonal factorization system* in case it restricts, along $\mathcal{J}$, to an orthogonal factorization system on $\mathcal{V}$ (which then will automatically be $\boldsymbol{\omega}$**CPO**-enriched as $\mathcal{J}$ is order-reflecting).

We next construct two such factorization systems on $\mathbf{SSh}(C, \mathcal{J}, \mathcal{K})_\perp$.

Given a subpresheaf $A$ (in $\mathbf{PSh}(C)$) of some $B_\perp$ in $\mathbf{SSh}(C, \mathcal{J}, \mathcal{K})$, we define the $\mathrm{Cl}_\perp$-closure of $A$ in $B_\perp$ by

$$(\mathrm{Cl}_\perp A)C \stackrel{\text{def}}{=} \left\{(U \xrightarrow{m} C, \beta) \in B_\perp C \mid (\mathrm{id}_U, \beta) \in AU\right\}.$$

Lemma 6.10. *$\mathrm{Cl}_\perp A$ defines a subpresheaf of $B$ such that $A \subseteq \mathrm{Cl}_\perp A$. In case $A$ is $\mathrm{Cl}_{\omega\mathcal{K}}$-closed or $\mathrm{Cl}_{\omega\mathcal{J}}$-closed, so is $\mathrm{Cl}_\perp A$.*

Proof. Let $C' \xrightarrow{f} C$. Suppose that $(U \xrightarrow{m} C, \beta) \in (\mathrm{Cl}_\perp A)C$. Then, $(\mathrm{id}_U, \beta) \in A$. Therefore, $B_\perp(f)(m, \beta) = (f^*m, B(m^*f)(\beta))$. Now, $(f^*m, B(m^*f)(\beta)) \in (\mathrm{Cl}_\perp A)C'$ iff $(\mathrm{id}_{f^*U}, B(m^*f)(\beta)) \in A(f^*U)$. This is true as $(m^*f)^*\mathrm{id}_U = \mathrm{id}_{f^*U}$ and $A$ is a subpresheaf of $B_\perp$ by assumption. This shows that $\mathrm{Cl}_\perp A$ is a subpresheaf of $B_\perp$.

Now, suppose that $(U \xrightarrow{m} C, \beta) \in AC$. Then, $(\mathrm{id}_U, \beta) = (m^*m, B(m^*m)(\beta)) = A(m)(m, \beta) \in AU$. Therefore, $(m, \beta) \in (\mathrm{Cl}_\perp A)C$. It follows that $A \subseteq \mathrm{Cl}_\perp A$.

Suppose that $A$ is $\mathrm{Cl}_{\omega\mathcal{K}}$-closed (resp. $\mathrm{Cl}_{\omega\mathcal{J}}$-closed). Let $\left((U_n \xrightarrow{m_n} C, \beta_n)\right)_{n\in\mathbb{N}}$ be an $\omega$-chain in $(\mathrm{Cl}_\perp A)C$ (i.e. $(\mathrm{id}_{U_n}, \beta_n) \in AU_n$). Then, there exists some lub $(U_\omega \xrightarrow{m_\omega} C, \beta_\omega)$ in $B_\perp C$. Observe that $m_n \leq m_\omega$ is a $\mathcal{J}$-cover hence in particular a $\mathcal{K}$-cover. $(\mathrm{id}_{U_n}, \beta_n)$ is a matching family in $A$ w.r.t. this cover which has amalgamation $(m_n \leq m_\omega, \beta_n)$ in $B_\perp$. As $A$ is $\mathrm{Cl}_\mathcal{K}$-closed (resp. $\mathrm{Cl}_\mathcal{J}$-closed), it follows that also $(m_n \leq m_\omega, \beta_n) \in AU_\omega$. Observe that $(m_n \leq m_\omega, \beta_n)$ defines an $\omega$-chain with lub $(\mathrm{id}_{U_\omega}, \beta_\omega)$ in $B_\perp U_\omega$. As $A$ is $\mathrm{Cl}_\omega$-closed, it follows that $(\mathrm{id}_{U_\omega}, \beta_\omega) \in AU_\omega$. Therefore, $(m_\omega, \beta_\omega) \in (\mathrm{Cl}_\perp A)C$. We see that $\mathrm{Cl}_\perp A$ is $\mathrm{Cl}_\omega$-closed.

Next, we show that it is also $\mathrm{Cl}_\mathcal{K}$-closed (resp. $\mathrm{Cl}_\mathcal{J}$-closed). Indeed, let $(U \xrightarrow{m} C, \beta) \in B_\perp C$ and let $R \in \mathcal{K}C$ (resp. $R \in \mathcal{J}C$) and suppose that $(f^*m, B(m^*f)(\beta)) = B_\perp(f)(m, \beta) \in (\mathrm{Cl}_\perp A)C_f$ for all $C_f \xrightarrow{f} C \in R$. That is, $B_\perp(m^*f)(\mathrm{id}_U, \beta) = (\mathrm{id}_{f^*U}, B(m^*f)(\beta)) \in A(f^*U)$. Equivalently, $B_\perp(g)(\mathrm{id}_U, \beta) =\in A(U_g)$ for all $U_g \xrightarrow{g} U$ in $f^*R \in \mathcal{K}U$ (resp. $f^*R \in \mathcal{J}U$), where we use that Grothendieck topologies are closed under pullback. As $A$ is $\mathrm{Cl}_\mathcal{K}$-closed (resp. $\mathrm{Cl}_\mathcal{J}$-closed), it now follows that $(\mathrm{id}_U, \beta) \in AU$. Therefore, $(m, \beta) \in (\mathrm{Cl}_\perp A)C$. We see that $\mathrm{Cl}_\perp A$ is $\mathrm{Cl}_\mathcal{K}$-closed (resp. $\mathrm{Cl}_\mathcal{J}$-closed). □

As a consequence, $\mathrm{Cl}_{\omega\mathcal{K}\perp} A \stackrel{\text{def}}{=} \mathrm{Cl}_\perp \mathrm{Cl}_{\omega\mathcal{K}} A$ defines the smallest subpresheaf of $B$ containing $A$ that is both $\mathrm{Cl}_\perp$-closed and $\mathrm{Cl}_{\omega\mathcal{K}}$-closed, and similarly for $\mathrm{Cl}_{\omega\mathcal{J}\perp} A \stackrel{\text{def}}{=} \mathrm{Cl}_\perp \mathrm{Cl}_{\omega\mathcal{J}} A$.

Given a subpresheaf $A$ of $B_\bot$, let us define

$$A^{\uparrow}C \overset{\mathrm{def}}{=} \{\alpha \in BC \mid (\mathrm{id}_C, \alpha) \in A\}$$

.

Lemma 6.11. *$A^{\uparrow}$ is a subpresheaf of $B$ and $\mathrm{Cl}_\bot A = A^{\uparrow}{}_\bot$.*

Proof. Suppose that $\alpha \in AC$ and $C' \xrightarrow{f} C$. (i.e. $(\mathrm{id}_C, \alpha) \in AC$) Then, $(\mathrm{id}_{C'}, B(f)(\alpha)) = (f^*\mathrm{id}_C, B(\mathrm{id}^*_C f)(\alpha)) = B_\bot(f)(\mathrm{id}_C, \alpha)$. As $A$ is a subpresheaf of $B_\bot$, it follows that $(\mathrm{id}_{C'}, B(f)(\alpha)) \in AC'$ hence $B(f)(\alpha) \in A^{\uparrow}C'$. We see that $A^{\uparrow}$ is a subpresheaf of $B$.

Now,

$$\begin{aligned}\mathrm{Cl}_\bot(A)C &= \left\{(U \xrightarrow{m} C, \beta) \in B_\bot C \mid (\mathrm{id}_U, \beta) \in AU\right\}\\ &= \left\{(U \xrightarrow{m} C, \beta) \in B_\bot C \mid \beta \in A^{\uparrow}U\right\}\\ &= A^{\uparrow}{}_\bot C.\end{aligned}$$

□

In particular, $A$ is $\mathrm{Cl}_\bot$-closed iff $A = A^{\uparrow}{}_\bot$ iff there exists an $A' \subseteq B$ such that $A = A'_\bot$.

Lemma 6.12. *Suppose we are given the commutative diagram below (without $\gg\!= y$),*

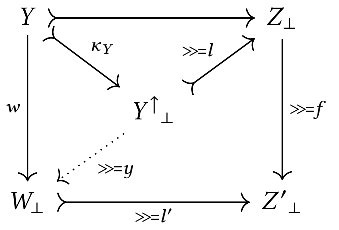


*then there exists a unique $y$ making the diagram commute.*

Proof. Uniqueness of $y$ is evident as $\gg\!= l'$ is a mono.

We show its existence. Indeed, suppose that $(U \xrightarrow{m} C, \alpha) \in Y^{\uparrow}{}_\bot C$, i.e. $(\mathrm{id}_U, \alpha) \in YU$. Then, $(f^1_U(\alpha), f^2_U(\alpha)) = (f^1_U(\alpha); \mathrm{id}_U, f^2_U(\alpha)) = (\gg\!= f)_U(\mathrm{id}_U, \alpha) \in W_\bot U$. Therefore, $f^2_U(\alpha) \in WU_\alpha$ where $U_\alpha$ is the domain of $f^1_U(\alpha)$. As a consequence $(\gg\!= f)_C(m, \alpha) = (f^1_U(\alpha); m, f^2_U(\alpha)) \in W_\bot C$. We see that $\gg\!= f$ restricts to a map $Y^{\uparrow}{}_\bot \to W_\bot$. This map is of the form $\gg\!= y$, where $y_C(\alpha) \overset{\mathrm{def}}{=} f_C(\alpha)$. □

This lets us define orthogonal factorization systems on $\mathbf{SSh}(C, \mathcal{J}, \mathcal{K})_\bot$.

Theorem 6.13 (Factorization Systems on $\mathbf{SSh}(C, \mathcal{J}, \mathcal{K})_\bot$). *Let us consider $\mathbf{SSh}(C, \mathcal{J}, \mathcal{K})_\bot$ as the subcategory of $\mathbf{SSh}(C, \mathcal{J}, \mathcal{K})$ on the objects of the form $A_\bot$ and morphisms of the form $\gg\!= f$.*

*Taking $(\mathcal{E}', \mathcal{M}')$ to consist of either*

- *$\mathrm{Cl}_{\omega\mathcal{K}\bot}$-dense morphisms as $\mathcal{E}'$;*
- *$\mathrm{Cl}_{\omega\mathcal{K}\bot}$-closed monos as $\mathcal{M}'$ (i.e. full strong monos with domain of the form $A_\bot$);*

*or*

- *$\mathrm{Cl}_{\omega\mathcal{J}\bot}$-dense morphisms as $\mathcal{E}'$;*
- *$\mathrm{Cl}_{\omega\mathcal{J}\bot}$-closed monos as $\mathcal{M}'$ (i.e. full monos with domain of the form $A_\bot$);*

*gives us two $\omega\mathbf{CPO}$-enriched orthogonal factorization systems on $\mathbf{SSh}(C, \mathcal{J}, \mathcal{K})_\bot$. Both are compatible with $\mathbf{SSh}(C, \mathcal{J}, \mathcal{K}) \hookrightarrow \mathbf{SSh}(C, \mathcal{J}, \mathcal{K})_\bot$.*

Proof. We do the proof for the first factorization system, but it is entirely analogous for the second.

Given $\gg\!= f : X_\perp \to Z_\perp$, we factor it as $e; m$ where $e \in \mathcal{E}$ is a $\mathrm{Cl}_{\omega\mathcal{K}}$-dense morphism and $m \in \mathcal{M}$ is a $\mathrm{Cl}_{\omega\mathcal{K}}$-closed mono.

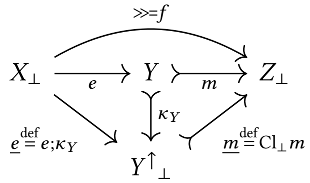


Let us write $\kappa_Y$ for the unique inclusion mono that witnesses $m \leq \mathrm{Cl}_\perp m$. We define $\underline{m}$ as $\mathrm{Cl}_\perp m$ and note that it is a $\mathrm{Cl}_{\omega\mathcal{K}\perp}$-closed mono, but lemma 6.10. Seeing that $e$ is $\mathrm{Cl}_{\omega\mathcal{K}}$-dense, we have that $\mathrm{Cl}_{\omega\mathcal{K}}\mathrm{Im}(e) = Y$. Therefore, $\mathrm{Cl}_{\omega\mathcal{K}\perp}\mathrm{Im}\left(\underline{e}\right) = \mathrm{Cl}_\perp\mathrm{Cl}_{\omega\mathcal{K}}\mathrm{Im}\left(\underline{e}\right) = \mathrm{Cl}_\perp(\mathrm{Cl}_{\omega\mathcal{K}}(\kappa_Y[\mathrm{Im}\left(\underline{e}\right)])) = \mathrm{Cl}_\perp(\kappa_Y(\mathrm{Cl}_{\omega\mathcal{K}}\mathrm{Im}\left(\underline{e}\right))) = \mathrm{Cl}_\perp(\kappa_Y(Y)) = Y^{\uparrow}{}_\perp$. We see that $\underline{e}$ is $\mathrm{Cl}_{\omega\mathcal{K}\perp}$-dense.

As a subset inclusion of a $\mathrm{Cl}_\perp$-closed subpresheaf, $\underline{m} = \gg\!= (q; \mathrm{return}_Z)$ where $q$ is the inclusion $Y^{\uparrow} \hookrightarrow Z$. Let us write $l \stackrel{\text{def}}{=} q; \mathrm{return}_Z = \mathrm{return}_{Y^{\uparrow}}; \underline{m}$. That is, $\underline{m} = \gg\!= l$.

Now, $\gg\!= (\mathrm{return}_X; \underline{e}); \gg\!= l = \gg\!= (\mathrm{return}_X; \underline{e}; \gg\!= l) = \gg\!= (\mathrm{return}_X; \gg\!= f) = \gg\!= f = \underline{e}; \gg\!= l$. As $\gg\!= l$ is a mono, it follows that $\underline{e} = \gg\!= k$ for $k = \mathrm{return}_X; \underline{e}$.

By the functoriality of the factorization system $(\mathcal{E}, \mathcal{M})$=($\mathrm{Cl}_{\omega\mathcal{K}}$-dense, $\mathrm{Cl}_{\omega\mathcal{K}}$-closed mono) factorization system on $\mathbf{SSh}(\mathcal{C}, \mathcal{J}, \mathcal{K})$, it follows that we get a unique $h : Y \to Y'$ making the diagram below commute.

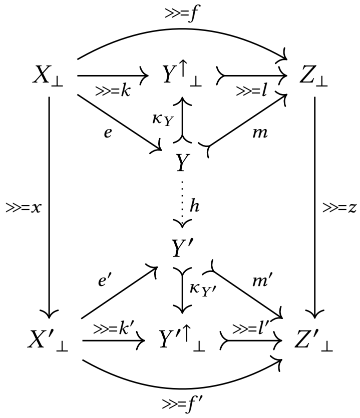


Now, by lemma 6.12, $h; \kappa_{Y'} : Y \to Y'^{\uparrow}{}_\perp$ has a unique extension to a morphism $\gg\!= y : Y^{\uparrow}{}_\perp \to Y'^{\uparrow}{}_\perp$ such that $\kappa_Y; \gg\!= y = h; \kappa_{Y'}$ and $\gg\!= y; \gg\!= l' = \gg\!= l; \gg\!= z$. Therefore, $\gg\!= k; \gg\!= y = e; \kappa_Y; \gg\!= y = e; h; \kappa_{Y'} = \gg\!= x; e'; \kappa_{Y'} = \gg\!= x; \gg\!= k'$. We see that the factorization $\gg\!= f \mapsto (\gg\!= k, \gg\!= l)$ extends to a functor.

To see $\boldsymbol{\omega}\mathbf{CPO}$-enrichment, we need to show that $\gg\!= y$ depends $\omega$-continuously on $(\gg\!= x, \gg\!= z)$. This is obvious as $\gg\!= y$ is the restriction of $\gg\!= z$ to full subpresheaves of the domain and codomain.

Finally, observe that given an $f : X \to Y$ in $\mathbf{SSh}_{\omega\mathbf{CPO}}(C, \mathcal{J}, \mathcal{K})$, we have that $\mathrm{Im}\,(f)_\perp = \mathrm{Im}\,(f_\perp)$. Indeed,

$$\begin{aligned}\mathrm{Im}\,(f)_\perp C &= \left\{(m, \beta) \mid U \xrightarrow{m} C \in \mathfrak{M}, \exists \alpha \in XU.\beta = f_U(\alpha) \in\right\}\\ &= \{(m, \beta) \mid \exists (n, \alpha) \in X_\perp C.(m, \beta) = (n, f_U(\alpha))\}\\ &= \{(m, \beta) \mid \exists (n, \alpha) \in X_\perp C.(m, \beta) = (f_\perp)_C(n, \alpha)\}\\ &= \mathrm{Im}\,(f_\perp)\,C\end{aligned}$$

Therefore, using the fact that $\mathrm{Cl}_\perp$ preserves $\mathrm{Cl}_{\omega\mathcal{K}}$-closedness:

$$\begin{aligned}(\mathrm{Cl}_{\omega\mathcal{K}}\mathrm{Im}\,(f))_\perp &= \mathrm{Cl}_{\omega\mathcal{K}\perp}\mathrm{Im}\,(f)\\ &= \mathrm{Cl}_{\omega\mathcal{K}\perp}(\mathrm{Cl}_\perp\mathrm{Im}\,(f))\\ &= \mathrm{Cl}_{\omega\mathcal{K}\perp}(\mathrm{Im}\,(f)_\perp)\\ &= \mathrm{Cl}_{\omega\mathcal{K}\perp}\mathrm{Im}\,(f_\perp)\,.\end{aligned}$$

It follows that the ($\mathrm{Cl}_{\omega\mathcal{K}}$-dense, $\mathrm{Cl}_{\omega\mathcal{K}}$-closed mono) factorization $e; m$ of $f : X \to Y$ gives rise to the ($\mathrm{Cl}_{\omega\mathcal{K}\perp}$-dense, $\mathrm{Cl}_{\omega\mathcal{K}\perp}$-closed mono) factorization $e_\perp; m_\perp$ of $f_\perp$. It follows that it is compatible with $\mathbf{SSh}(C, \mathcal{J}, \mathcal{K}) \hookrightarrow \mathbf{SSh}(C, \mathcal{J}, \mathcal{K})_\perp$.

□

Proposition 6.14. *Consider* $\mathbf{SSh}_{\omega\mathbf{CPO}}(C, \mathcal{J}, \mathcal{K})$ *with either of its two canonical factorization systems* $(\mathcal{E}, \mathcal{M})$*, together with the corresponding compatible factorization system* $(\mathcal{E}', \mathcal{M}')$ *on* $\mathbf{SSh}_{\omega\mathbf{CPO}}(C, \mathcal{J}, \mathcal{K})_\perp$ *(see theorem 6.13). Then, we have that*

*(1)* $\mathcal{M}; \mathrm{return} \subseteq \mathcal{M}'$*;*
*(2)* $\mathcal{M}' \subseteq \mathcal{M}; \mathrm{return}$*;*
*(3)* $\mathcal{M}_\perp \subseteq \mathcal{M}$*.*

Proof. We consider the case where $(\mathcal{E}, \mathcal{M})$ is the ($\mathrm{Cl}_{\omega\mathcal{K}}$-dense, $\mathrm{Cl}_{\omega\mathcal{K}}$-closed mono) factorization system (in which case $(\mathcal{E}', \mathcal{M}')$ is the ($\mathrm{Cl}_{\omega\mathcal{K}\perp}$-dense, $\mathrm{Cl}_{\omega\mathcal{K}\perp}$-closed mono)-factorization system). The proofs for the ($\mathrm{Cl}_{\omega\mathcal{J}}$-dense, $\mathrm{Cl}_{\omega\mathcal{J}}$-closed mono) factorization system are almost identical.

(1) Suppose that $m : A \rightarrowtail B$ is a $\mathrm{Cl}_{\omega\mathcal{K}}$-closed mono. We need to show that $m; \mathrm{return}_B$ is a $\mathrm{Cl}_{\omega\mathcal{K}\perp}$-closed mono.
First, we show $\mathrm{return}_B$ is a $\mathrm{Cl}_{\mathcal{K}}$-closed mono. Let $(m, \alpha) \in B_\perp C$ and $R \in \mathcal{K}C$ such that $\forall f \in R.(f^*m, B(m^*f)(\alpha)) = B_\perp(f)(m, \alpha) \in B$. That is, $f^*m = \mathrm{id}$. Meanwhile, $f^*m = \mathrm{id}$ forms a matching family for $\mathfrak{M}$ w.r.t. $R$. Now, $m$ and id are both amalgamations for this matching family. As $\mathfrak{M}$ is $\mathcal{K}$-separated, they coincide. We see that $(m, \alpha) = (\mathrm{id}, \alpha) \in B$.
Second, we show that $\mathrm{return}_B$ is a $\mathrm{Cl}_\omega$-closed mono. First, observe that $\mathrm{return}_B$ is a full mono: $\mathrm{return}_B(\alpha) \leq \mathrm{return}_B(\alpha')$ means $(\mathrm{id}, \alpha) \leq (\mathrm{id}, \alpha)$ which means $\mathrm{id} \leq \mathrm{id}$ and $\alpha \leq B(\mathrm{id} \leq \mathrm{id})(\alpha') = \alpha'$. Let $\left(\alpha^i\right)_{i\in\mathbb{N}}$ be an $\omega$-chain in $B_\perp$ with lub $\alpha$. Suppose that $\alpha^i \in B$ for all $i \in \mathbb{N}$. As $B$ is $\omega$-chain-closed by assumption and $\alpha^i$ is an $\omega$-chain in $B$ by fullness of $\mathrm{return}_B$, it follows that also $\alpha \in B$.
It now follows that $\mathrm{return}_B$ is $\mathrm{Cl}_{\omega\mathcal{K}}$-closed. As $\mathrm{Cl}_{\omega\mathcal{K}}$-closed monos compose, $m; \mathrm{return}$ is also $\mathrm{Cl}_{\omega\mathcal{K}}$-closed.
We claim that $m; \mathrm{return} \mapsto\gg= (m; \mathrm{return})$ is precisely the $\mathrm{Cl}_\perp$-closure. If we show that, it follows that $m; \mathrm{return}$ is $\mathrm{Cl}_{\omega\mathcal{K}\perp}$-closed, as $\mathrm{Cl}_\perp$-closure preserves $\mathrm{Cl}_{\omega\mathcal{K}}$-closedness. To see that it is this closure, note that $A = (A_\perp)^\uparrow$ as its inclusion in $B$ factors over return.
(2) Suppose that $\gg= m' : A^\uparrow{}_\perp \rightarrowtail B_\perp$ is $\mathrm{Cl}_{\omega\mathcal{K}\perp}$-closed. Clearly, $m' = m; \mathrm{return}$ for some mono $m : A^\uparrow \rightarrowtail B$. Indeed, $A^\uparrow C = \{\alpha \in AC \mid \exists \beta \in BC.m'(\alpha) = (\mathrm{id}_C, \beta)\}$, so we can define $m(\alpha) = \mathrm{snd}(m'(\alpha))$. We claim that $m$ is a $\mathrm{Cl}_{\omega\mathcal{K}}$-closed mono. To see that $m$ is a full mono, suppose that

$m(\alpha) \leq^{B} m(\alpha')$. Then, $\gg\!= m'(\mathrm{id}, \alpha) = (\mathrm{id}, m(\alpha)) \leq^{B_\perp} (\mathrm{id}, m(\alpha')) = \gg\!= m'(\mathrm{id}, \alpha')$. As $\gg\!= m'$ is a full mono, by assumption, it follows that $(\mathrm{id}, \alpha) \leq^{A^{\uparrow}{}_{\perp}} (\mathrm{id}, \alpha')$. Therefore, $\alpha \leq^{A^{\uparrow}} \alpha'$. Suppose that $\left(\alpha^i\right)_{i \in \mathbb{N}}$ is an $\omega$-chain in $B$ such that $\alpha^i \in A^{\uparrow}$ for all $i$. Then, $\alpha^i$ is an $\omega$-chain in $A^{\uparrow}$. It follows that $m$ is $\mathrm{Cl}_{\omega}$-closed once we show that $A^{\uparrow}$ is $\omega$-chain-closed. Now, $(\mathrm{id}, \alpha^i)$ defines an $\omega$-chain in $A^{\uparrow}{}_{\perp} = A$. As $A$ is $\omega$-chain-closed by assumption, we have a lub $(m, \alpha)$, which we have shown to have the property that $m = \sup_i \mathrm{id} = \mathrm{id}$. Therefore, $\alpha \in A^{\uparrow}$. Finally, we show that $m$ is $\mathrm{Cl}_{\mathcal{K}}$-closed. Suppose that $R \in \mathcal{K}C$, $\beta \in BC$ and for all $C' \xrightarrow{f} C \in R$ $B(f)(\beta) \in A^{\uparrow}C'$. Then, $(\mathrm{id}_{C'}, B(f)(\beta)) \in AC'$. We have an amalgamation $(\mathrm{id}, \beta)$ in $B$. As $A$ is $\mathrm{Cl}_{\mathcal{K}}$-closed in $B$ by assumption, we have that $(\mathrm{id}, \beta) \in AC$. Therefore, $\beta \in A^{\uparrow}$.

(3) Suppose that $m : A \rightarrowtail B \in \mathcal{M}$. We have shown that also $\mathrm{return}_B \in \mathcal{M}$. Therefore, $m; \mathrm{return}_B \in \mathcal{M}$, i.e. $m; \mathrm{return}_B$ is a $\mathrm{Cl}_{\omega\mathcal{K}}$-closed mono. We have further observed that $m_\perp = \gg\!= (m; \mathrm{return}_B)$ is the $\mathrm{Cl}_\perp$-closure of $m; \mathrm{return}_B$. We have already seen that $\mathrm{Cl}_\perp$-closure preserves $\mathrm{Cl}_{\omega\mathcal{K}}$-closedness. Therefore, $m_\perp = \gg\!= (m; \mathrm{return}_B)$ is a $\mathrm{Cl}_{\omega\mathcal{K}}$-closed mono, hence a member of $\mathcal{M}$.

□

## 7 BILIMIT COMPACT SCONING

We can extend the standard sconing (Artin gluing) techniques as discussed in e.g. [Carboni and Johnstone 1995; Johnstone et al. 2007; Mitchell and Scedrov 1992] to apply to the categorical structure of bilimit compact expansions. This lets us formulate logical relations arguments for recursive types.

Recall that the basic idea of sconing is that one starts off with a functor $\mathcal{C}_1 \xrightarrow{F} \mathcal{C}_2$. Under suitable restrictions on $F$ and $\mathcal{C}_1$, the comma category $\mathcal{C}_2/F$, also known as the *scone* of $F$, lifts the categorical structure present in $\mathcal{C}_2$. This gives us a way of building new categorical models from existing ones. For the following, we recall that $\mathcal{C}_2/F$ has objects $(C_2, f, C_1)$, where $C_2$ is an object in $\mathcal{C}_2$, $C_1$ is an object in $\mathcal{C}_1$ and $f : C_2 \to FC_1$ is a morphism in $\mathcal{C}_2$. Morphisms in $\mathcal{C}_2/F$ from $(C_2, f, C_1)$ to $(C_2', f', C_1')$ are pairs $(g_2, g_1)$ of a morphism $C_2 \xrightarrow{g_2} C_2'$ in $\mathcal{C}_2$ and a morphism $C_1 \xrightarrow{g_1} C_1'$ in $\mathcal{C}_1$, such that $f; Fg_1 = g_2; f'$.

Proposition 7.1 (Well-known,[Carboni and Johnstone 1995; Rydeheard and Burstall 1988]). *Supposing that $\mathcal{C}_1$ and $\mathcal{C}_2$ are cocomplete, we have that $\mathcal{C}_2/F$ is cocomplete. Supposing that $\mathcal{C}_1$ and $\mathcal{C}_2$ are cartesian closed, $\mathcal{C}_2$ has pullbacks and $F$ preserves finite products, then $\mathcal{C}_2/F$ is cartesian closed. Finally, the forgetful functors $\mathcal{C}_2/F \longrightarrow \mathcal{C}_1$ and $\mathcal{C}_2/F \longrightarrow \mathcal{C}_1$ preserve all of this categorical structure.*

Let us observe that any subcategory $\mathcal{C} \hookrightarrow \mathcal{D}$ factors uniquely as a lluf embedding followed by a full embedding $\mathcal{C} \xhookrightarrow{\text{lluf}} \mathbf{Mix}(\mathcal{C}, \mathcal{D}) \xhookrightarrow{\text{full}} \mathcal{D}$, thus uniquely defining an intermediate subcategory $\mathbf{Mix}(\mathcal{C}, \mathcal{D})$ between $\mathcal{C}$ and $\mathcal{D}$.

Theorem 7.2 (Sconing for Bilimit Compact Expansions). *Suppose we are given a pair of locally continuous functors $(F_V, F_C)$ from a bilimit compact expansion $\mathcal{J}_1 : \mathcal{V}_1 \hookrightarrow \mathcal{C}_1$ to a bilimit compact expansion $\mathcal{J}_2 : \mathcal{V}_2 \hookrightarrow \mathcal{C}_2$ such that the following diagram commutes:*

$$\begin{array}{ccc} \mathcal{V}_1 & \xhookrightarrow{\mathcal{J}_1} & \mathcal{C}_1 \\ \downarrow{\scriptstyle F_V} & & \downarrow{\scriptstyle F_C} \\ \mathcal{V}_2 & \xhookrightarrow{\mathcal{J}_2} & \mathcal{C}_2 \end{array}$$

*and such that $F_C$ is $\boldsymbol{\omega}\mathbf{CPO}_\perp$-enriched (i.e. it is strict) Then, the embedding*

$$\mathcal{V}_2/F_V \hookrightarrow C_2/F_C$$

$$(V_2, f, V_1) \longmapsto (\mathcal{J}_2 V_2, \mathcal{J}_2 f, \mathcal{J}_1 V_1)$$

*(which is well-defined as $\mathcal{J}_2(F_V V_1) = F_C(\mathcal{J}_1 V_1)$) determines a bilimit compact expansion* $\mathcal{J}_2/F : \mathcal{V}_2/F_V \hookrightarrow \mathbf{Mix}(\mathcal{V}_2/F_V, C_2/F_C)$.

Proof. First, we show that $\mathbf{Mix}(\mathcal{V}_2/F_V, C_2/F_C)$ (and by essentially the same argument also $\mathcal{V}_2/F_V$, using the $\boldsymbol{\omega}$**CPO**-enrichment of $\mathcal{V}_2$ and $\mathcal{V}_1$) are $\boldsymbol{\omega}$**CPO**-enriched. Observe that we have that

$$\mathbf{Mix}(\mathcal{V}_2/F_V, C_2/F_C)((C_2, f, C_1), (C_2', f', C_1')) \stackrel{\text{def}}{=} \left\{(g_2, g_1) \in C_2(C_2, C_2') \times C_1(C_1, C_1') \mid f; Fg_1 = g_2; f'\right\}.$$

In particular, $C_2$ immediately inherits the poset-enriched structure of $C_2 \times C_1$. To show that it also inherits the $\boldsymbol{\omega}$**CPO**-enriched structure of $C_2 \times C_1$, we need to show that the condition $f; Fg_1 = g_2; f'$ is preserved under sups of $\omega$-chains. Therefore, suppose we have an $\omega$-chain $\left((g_2^n, g_1^n)\right)_{n \in \mathbb{N}}$ in $\mathbf{Mix}(\mathcal{V}_2/F_V, C_2/F_C)((C_2, f, C_1), (C_2', f', C_1'))$. Then, we have that $f; Fg_1^n = g_2^n; f'$. But this implies that $f; F(\bigvee_n g_1^n) = f; \bigvee_n F(g_1^n) = \bigvee_n f; F(g_1^n) = \bigvee_n (g_2^n; f') = (\bigvee_n g_2^n); f'$, as $C_1$ and $C_2$ are $\boldsymbol{\omega}$**CPO**-enriched (meaning that composition is $\omega$-continuous) and $F$ is locally continuous. We see that $\mathbf{Mix}(\mathcal{V}_2/F_V, C_2/F_C)$ and similarly also $\mathcal{V}_2/F_V$ are $\boldsymbol{\omega}$**CPO**-enriched.

Second, we show that $\mathbf{Mix}(\mathcal{V}_2/F_V, C_2/F_C)$ is bilimit compact. We claim that $(\mathbb{0}, ?_{F_V \mathbb{0}}, \mathbb{0})$ gives an ep-zero object for $\mathbf{Mix}(\mathcal{V}_2/F_V, C_2/F_C)$, where $?_{F_V \mathbb{0}}$ is the unique morphism $\mathbb{0} \to F_C \mathbb{0}$ in $\mathcal{V}_2$. Indeed, let $(C_2, f, C_1)$ be any object in $C_2/F_C$. Then, we get a unique morphism $\mathbb{0} \xrightarrow{\perp^{\mathrm{e}}} C_1$ in $C_1$ and a unique morphism $\mathbb{0} \xrightarrow{\perp^{\mathrm{e}}} C_2$ in $C_2$, both of which are embeddings, while also $\perp^{\mathrm{e}}; f = ?_{F_V \mathbb{0}}; F_C \perp^{\mathrm{e}}$, by initiality of $\mathbb{0}$ in $\mathcal{V}_2$. That is, we have a unique morphism $(\perp^{\mathrm{e}}, \perp^{\mathrm{e}}) : (\mathbb{0}, ?_{F_V \mathbb{0}}, \mathbb{0}) \to (C_2, f, C_1)$, showing that $(\mathbb{0}, ?_{F_V \mathbb{0}}, \mathbb{0})$ is the initial object in $\mathbf{Mix}(\mathcal{V}_2/F_V, C_2/F_C)$. Moreover, as $\mathbf{Mix}(\mathcal{V}_2/F_V, C_2/F_C)$ has the product order of $C_2 \times C_1$ on its homsets and as $(\perp^{\mathrm{e}}, \perp^{\mathrm{e}})$ consists of two embeddings, it is itself an embedding. Similarly, as $\mathbb{0}$ and $\mathbb{0}$ are zero objects in $C_2$ and $C_1$, we also get unique morphisms $C_2 \xrightarrow{\perp^{\mathrm{p}}} \mathbb{0}$ and $C_1 \xrightarrow{\perp^{\mathrm{p}}} \mathbb{0}$, both of which are projections, while also $\perp^{\mathrm{p}}; ?_{F_V \mathbb{0}} = f; F_C \perp^{\mathrm{p}}$ (because $F_C$ is strict while composition in $\mathcal{V}_2$ is also strict). That is, we have a unique morphism $(\perp^{\mathrm{p}}, \perp^{\mathrm{p}}) : (C_2, f, C_1) \to (\mathbb{0}, ?_{F_V \mathbb{0}}, \mathbb{0})$, showing that $(\mathbb{0}, ?_{F_V \mathbb{0}}, \mathbb{0})$ is the terminal object in $\mathbf{Mix}(\mathcal{V}_2/F_V, C_2/F_C)$. Moreover, as $\mathbf{Mix}(\mathcal{V}_2/F_V, C_2/F_C)$ has the product order of $C_2 \times C_1$ on its homsets and as $(\perp^{\mathrm{p}}, \perp^{\mathrm{p}})$ consists of two projections, it is itself a projection. It follows that $(\mathbb{0}, ?_{F_V \mathbb{0}}, \mathbb{0})$ is an ep-zero object in $\mathbf{Mix}(\mathcal{V}_2/F_V, C_2/F_C)$.

Next, let $\left(\left((C_2^n, f^n, C_1^n)\right)_{n \in \mathbb{N}}, \left((g_2^n, g_1^n)\right)_{n \in \mathbb{N}}\right)$ be an $\omega$-chain of ep-pairs in $\mathbf{Mix}(\mathcal{V}_2/F_V, C_2/F_C)$. Let $(C_2^\omega, d_2)$ be the bilimit of $\left(g_2^n\right)_{n \in \mathbb{N}}$ (which we know exists in $C_2$) and let $(C_1^\omega, d_1)$ be the bilimit of $\left(g_1^n\right)_{n \in \mathbb{N}}$ (which we know exists in $C_1$). As $F_C$ is locally continuous, $\left(F_C g_1^n\right)_{n \in \mathbb{N}}$ defines an $\omega$-chain of ep-pairs with bilimit $(F_V C_1^\omega, F_C d_1)$. Then,

$$g_2^{n\mathrm{e}}; f^{n+1} = f^n; F_C g_1^{n\mathrm{e}} \quad \text{and} \quad g_2^{n\mathrm{p}}; f^n = f^{n+1}; F_C g_1^{n\mathrm{p}}.$$

As $\mathcal{V}_2 \hookrightarrow \mathcal{J}_2$ is a bilimit compact expansion and $f^n \in \mathcal{V}_2$, we have that $d_2^{n\mathrm{p}}; f^n; F_C d_1^{n\mathrm{e}}$ defines an $\omega$-chain in $C_2(C_2^\omega, F_C C_1^\omega)$ with lub $f^\omega \in \mathcal{V}_2(C_2^\omega, F_V C_1^\omega)$. Then, $((C_2^\omega, f^\omega, C_1^\omega), (d_2, d_1))$ is a bilimit in $\mathbf{Mix}(\mathcal{V}_2/F_V, C_2/F_C)$. Indeed, this follows from the fact that $(C_2^\omega, d_2)$ and $(C_1^\omega, d_1)$ are bilimits, once we show that $(d_2^{n\mathrm{e}}, d_1^{n\mathrm{e}}) \in \mathbf{Mix}(\mathcal{V}_2/F_V, C_2/F_C)((C_2^n, f^n, C_1^n), (C_2^\omega, f^\omega, C_1^\omega))$ (and similarly for

the corresponding projections). This holds as

$$\begin{aligned} d_2^{ne}; f^\omega &= d_2^{ne}; \bigvee_m d_2^{mp}; f^m; F_C d_1^{me} \\ &= \bigvee_m d_2^{ne}; d_2^{mp}; f^m; F_C d_1^{me} \\ &= \bigvee_m d_2^{ne}; d_2^{mp}; f^m; F_C d_1^{me} \\ &= f^n; F_C d_1^{ne} \end{aligned}$$

and

$$\begin{aligned} d_2^{np}; f^n &= \bigvee_m (d_2^{mp}; f^m; F_C(d_1^{me}; d_1^{np})) \\ &= \bigvee_m (d_2^{mp}; f^m; F_C d_1^{me}; F_C d_1^{np}) \\ &= (\bigvee_m d_2^{mp}; f^m; F_C d_1^{me}); F_C d_1^{np} \\ &= f^\omega; F_C d_1^{np}. \end{aligned}$$

Third, we show that $\mathcal{J}_2/F : \mathcal{V}_2/F_V \hookrightarrow \mathbf{Mix}(\mathcal{V}_2/F_V, \mathcal{C}_2/F_C); (V_2, f, V_1) \mapsto (\mathcal{J}_2 V_2, \mathcal{J}_2 f, \mathcal{J}_1 V_1)$ is a bilimit compact expansion. Observe that this functor is defined as $(V_2, f, V_1) \mapsto (\mathcal{J}_2 V_2, f, \mathcal{J}_1 V_1)$. As $\mathcal{J}_2$ and $\mathcal{J}_1$ are defined to be identity on objects, locally continuous, and order reflecting, it follows that the embedding is as well. The order reflecting part perhaps requires some more elaboration. This follows because $\mathbf{Mix}(\mathcal{V}_2/F_V, \mathcal{C}_2/F_C)$ has an order reflecting faithful functor into $\mathcal{C}_2 \times \mathcal{C}_1$ given by $(C_2, f, C_1) \mapsto (C_2, C_1)$. Let $((A_2, f, A_1), (a_2, a_1))$ and $((B_2, g, B_1), (b_2, b_1))$ be two ep-pair $\omega$-chains in $\mathbf{Mix}(\mathcal{V}_2/F_V, \mathcal{C}_2/F_C)$ with bilimits $((D_2, \phi, D_1), (d_2, d_1))$ and $((E_2, \psi, E_1), (e_2, e_1))$ and let us consider a countable collection of $\mathcal{V}_2/F_V$-morphisms $(\alpha_2^n, \alpha_1^n) : (A_2^n, f^n, A_1^n) \to (B_2^n, g^n, B_1^n)$ such that

$$\begin{aligned} (a_2^{ne}, a_1^{ne}); \mathcal{J}_2/F(\alpha_2^{n+1}, \alpha_1^{n+1}) &= \mathcal{J}_2/F(\alpha_2^n, \alpha_1^n); (b_2^{ne}, b_1^{ne}) \\ (a_2^{np}, a_1^{np}); \mathcal{J}_2/F(\alpha_2^n, \alpha_1^{n+1}) &= \mathcal{J}_2/F(\alpha_2^{n+1}, \alpha_1^{n+1}); (b_2^{np}, b_1^{np}). \end{aligned}$$

We need to show that there is some $\mathcal{V}_2/F_V$-morphism $(f_2, f_1) : (D_2, \phi, D_1) \to (E_2, \psi, E_1)$ such that $\mathcal{J}_2/F(f_2, f_1) = \bigvee_n (d_2^{np}, d_1^{np}); (\alpha_2^n, \alpha_1^n); (e_2^{ne}, e_1^{ne})$. Now, we know that $\mathcal{J}_2/F$ lifts the bilimit compact expansion $\mathcal{J}_2 \times \mathcal{J}_1$ (as we know bilimit compact expansions to be closed under finite products). Therefore, we know that there exists an $(f_2, f_1) : (D_2, D_1) \to (E_2, E_1)$ such that $\mathcal{J}_2 \times \mathcal{J}_1(f_2, f_1) = \bigvee_n (d_2^{np}, d_1^{np}); (\alpha_2^n, \alpha_1^n); (e_2^{ne}, e_1^{ne})$. We are done once we can show that this $(f_2, f_1)$ actually is a

morphism $(D_2, \phi, D_1) \to (E_2, \psi, E_1)$, hence that $f_2; \psi = \phi; F_C f_1$. This follows as

$$\begin{aligned} f_2; \psi &= (\bigvee_n d_2^{n\mathrm{p}}; \alpha_2^n; e_2^{n\mathrm{e}}); \psi \\ &= \bigvee_n (d_2^{n\mathrm{p}}; \alpha_2^n; e_2^{n\mathrm{e}}); \psi \\ &= \bigvee_n \phi; F_C(d_1^{n\mathrm{p}}; \alpha_1^n; e_1^{n\mathrm{e}}) \\ &= \phi; \bigvee_n F_C(d_1^{n\mathrm{p}}; \alpha_1^n; e_1^{n\mathrm{e}}) \\ &= \phi; F_C \bigvee_n (d_1^{n\mathrm{p}}; \alpha_1^n; e_1^{n\mathrm{e}}) \\ &= \phi; F_C f_1. \end{aligned}$$

□

In case we have a nice factorization system $(\mathcal{E}, \mathcal{M})$ on $C_2$, we often want to consider the full subcategory of the scone $C_2/F_C$ on the objects in $\mathcal{M}$. We call this category the *subscone* of $F_C$ and denote it $C_2//F_C$. In practice, $\mathcal{M}$ usually consists of some class of monos, meaning that we can think of $C_2//F_C$ as a category where the objects are objects $C_1$ of $C_1$ together with predicates on $F_C C_1$ and morphisms are simply morphisms of $C_1$ that respect these predicates. From now, we shall restrict our attention to subscones for factorization systems $(\mathcal{E}, \mathcal{M})$ such that $\mathcal{M}$ consists of monos. That is, $C_2//F_C$ is some category of logical relations.

Proposition 7.3 (Well-known). *For any orthogonal factorization system $(\mathcal{E}, \mathcal{M})$ on $C_2$ and a functor $F_C : C_1 \to C_2$, the subscone $C_2//F_C$ is a reflective subcategory of $C_2/F_C$. As a consequence, $C_2//F_C$ has limits and colimits of any shape that $C_2/F_C$ has. The forgetful functor $C_2//F_C \to C_1$ preserves limits and colimits.*

Proof. This is a straightforward consequence of corollary 6.2. □

Proposition 7.4 (Well-known, [Johnstone et al. 2007]). *In case $C_2/F_C$ is cartesian closed and the left-class $\mathcal{E}$ of the factorization system is closed under binary products (as a consequence, the right class $\mathcal{M}$ of the factorization system is closed under exponentiation ) we have that $C_2//F_C$ is cartesian closed. The forgetful functor $C_2//F_C \to C_1$ preserves exponentials.*

Summing up, we have that $C_2/F_C$ and $C_2//F_C$ are cartesian closed and cocomplete if $C_1$ and $C_2$ are and $C_2$ has pullbacks and $F_C$ preserves finite products and $\mathcal{E}$ is closed under binary products. This allows us to interpret various pure type formers in the scone and subscone, giving us reasoning methods about these type formers.

We now discuss how to think of this subscone in the context of bilimit compact categories and how this leads to a logical relations technique for reasoning about recursive types.

Theorem 7.5 (Subsconing for Bilimit Compact Expansions). *Suppose the scone $\mathcal{J}_2/F : \mathcal{V}_2/F_V \hookrightarrow \mathbf{Mix}(\mathcal{V}_2/F_V, C_2/F_C)$ is a bilimit compact expansion and we have a $\mathcal{J}_2$-compatible orthogonal factorization system $(\mathcal{E}', \mathcal{M}')$ on $C_2$ (which therefore restricts to a $\boldsymbol{\omega}\mathbf{CPO}$-enriched factorization system $(\mathcal{E}, \mathcal{M})$ on $\mathcal{V}_2$). Then, the subscone $\mathcal{J}_2//F : \mathcal{V}_2//F_V \hookrightarrow \mathbf{Mix}(\mathcal{V}_2//F_V, C_2//F_C)$ is a bilimit compact expansion.*

Proof. By corollary 6.2, we have that $\mathcal{M}'$ forms a full reflective $\boldsymbol{\omega}\mathbf{CPO}$-enriched subcategory of $C_2/C_2$.

Observe that we have a locally continuous functor $\mathcal{C}_2/F_C \to \mathcal{C}_2/\mathcal{C}_2$ which sends an object $(C_2, f, C_1)$ to $f$ and a morphism $(g_2, g_1)$ to the square $(g_2, F_C g_1)$. This lets us define $\mathcal{C}_1//F_C$ as the pullback

$$\begin{array}{ccc} \mathcal{C}_2//F_C & \longrightarrow & \mathcal{M}' \\ \big\downarrow \text{full} & & \big\downarrow \text{full} \\ \mathcal{C}_2/F_C & \longrightarrow & \mathcal{C}_2/\mathcal{C}_2. \end{array}$$

We can observe that the reflector $a$ restricts to yield a $\boldsymbol{\omega}$**CPO**-enriched left adjoint to the inclusion $\mathcal{C}_2//F_C \hookrightarrow \mathcal{C}_2/F_C$. Indeed, $a$ sends $(g_2, h) \in \mathcal{C}_2/\mathcal{C}_2(f, f')$ to $(\alpha(g_2), h) \in \mathcal{M}(m, m')$ where $f = e; m$ and $f' = e'; m'$ are the $(\mathcal{E}', \mathcal{M}')$-factorizations of $f$ and $f'$. Therefore, we obtain a $\boldsymbol{\omega}$**CPO**-enriched left adjoint to the inclusion $\mathcal{C}_2//F_C \hookrightarrow \mathcal{C}_2/F_C$ mapping $(g_2, g_1) \in \mathcal{C}_2/F_C((C_2, f, C_1), (C_2', f', C_1'))$ to $(\alpha(g_2), g_1) \in \mathcal{C}_2//F_C((D_2, m, C_1), (D_2', m', C_1'))$, where $f$ factors as $e; m$ and $f'$ as $e'; m'$.

Similarly, observe that we have a locally continuous functor $\mathcal{V}_2/F_V \to \mathcal{V}_2/\mathcal{V}_2$ which sends an object $(V_2, f, V_1)$ to $f$ and a morphism $(g_2, g_1)$ to the square $(g_2, F_V g_1)$. This lets us define $\mathcal{V}_2//F_V$ as the pullback

$$\begin{array}{ccc} \mathcal{V}_2//F_V & \longrightarrow & \mathcal{M} \\ \big\downarrow \text{full} & & \big\downarrow \text{full} \\ \mathcal{V}_2/F_V & \longrightarrow & \mathcal{V}_2/\mathcal{V}_2. \end{array}$$

We can observe that the reflector $a$ of $\mathcal{M}$ in $\mathcal{V}_2/\mathcal{V}_2$ restricts to yield a $\boldsymbol{\omega}$**CPO**-enriched left adjoint to the inclusion $\mathcal{V}_2//F_V \hookrightarrow \mathcal{V}_2/F_V$. Indeed, $a$ sends $(\mathcal{J}_2(g_2), \mathcal{J}_2(h)) \in \mathcal{C}_2/\mathcal{C}_2(f, f')$ to $(\mathcal{J}_2(\alpha(g_2)), \mathcal{J}_2(h)) \in \mathcal{M}(m, m')$ where $f = e; m$ and $f' = e'; m'$ are the $(\mathcal{E}, \mathcal{M})$-factorizations of $f$ and $f'$. Therefore, we obtain a $\boldsymbol{\omega}$**CPO**-enriched left adjoint to the inclusion $\mathcal{V}_2//F_V \hookrightarrow \mathcal{V}_2/F_V$ mapping $(g_2, g_1) \in \mathcal{V}_2/F_V((V_2, f, V_1), (V_2', f', V_1'))$ to $(\alpha(g_2), g_1) \in \mathcal{V}_2//F_V((W_2, m, V_1), (W_2', m', V_1'))$, where $f$ factors as $e; m$ and $f'$ as $e'; m'$.

Here, we observe that the reflection $\mathcal{C}_2/F_C \to \mathcal{C}_2//F_C$ restricts to the one $\mathcal{V}_2/F_V \to \mathcal{V}_2//F_V$ as $(\mathcal{E}, \mathcal{M})$ is the restriction of $(\mathcal{E}', \mathcal{M}')$ to $\mathcal{V}_2$. Therefore, we also get a reflection $\mathbf{Mix}(\mathcal{V}_2/F_V, \mathcal{C}_2/F_C) \to \mathbf{Mix}(\mathcal{V}_2//F_V, \mathcal{C}_2//F_C)$. Now we can apply lemma 3.1 to conclude. □

Combining theorems 7.2 and 7.5, we get the following.

Corollary 7.6. *Suppose we are given a pair of locally continuous functors $(F_V, F_C)$ from a bilimit compact expansion $\mathcal{J}_1 : \mathcal{V}_1 \hookrightarrow \mathcal{C}_1$ to a bilimit compact expansion $\mathcal{J}_2 : \mathcal{V}_2 \hookrightarrow \mathcal{C}_2$ such that the following diagram commutes:*

$$\begin{array}{ccc} \mathcal{V}_1 & \xhookrightarrow{\mathcal{J}_1} & \mathcal{C}_1 \\ \big\downarrow F_V & & \big\downarrow F_C \\ \mathcal{V}_2 & \xhookrightarrow{\mathcal{J}_2} & \mathcal{C}_2. \end{array}$$

*And suppose we are given a $\mathcal{J}_2$-compatible factorization system $(\mathcal{E}, \mathcal{M})$ on $\mathcal{C}_2$. Then, the subscone $\mathcal{J}_2//F : \mathcal{J}_2//(F_V; \mathcal{J}_2) \hookrightarrow \mathcal{C}_2//F_C$ is a bilimit compact expansion.*

In case we are working with $\mathcal{V}_2 = \boldsymbol{\omega}\mathbf{CPO}$ and $\mathcal{C}_2 = \boldsymbol{\omega}\mathbf{CPO}_\perp$ with the usual factorization system of (dense epis, full monos), the subscone will consist of chain closed subsets in $\mathcal{V}_2$ and chain closed bottom containing (also known as admissible) subsets in $\mathcal{C}_2$.

We will in particular be interested in applying the theorem above to a category of $\omega$-cpos in a Grothendieck quasitopos with one of the two canonical factorization systems.

*Definition 7.7 (Distributive law of monads).* Suppose we are given two categories each equipped with a monad, $(\mathcal{C}, \mathcal{S}, \mathrm{return}^{\mathcal{S}}, \mu^{\mathcal{S}})$ and $(\mathcal{D}, \mathcal{T}, \mathrm{return}^{\mathcal{T}}, \mu^{\mathcal{T}})$, together with a functor $F : \mathcal{C} \to \mathcal{D}$. Then,

a natural transformation $\sigma : F; T \longrightarrow S; F$ is called a *distributive law* if it satisfies:

$$\begin{array}{ccc} F & \xrightarrow{\mathrm{return}^T} & F;T \\ & \searrow^{F\mathrm{return}^S} & \downarrow \sigma \\ & & S;F \end{array} \qquad \begin{array}{ccccc} F;T & \xleftarrow{\mu^T_F} & F;T^2 & \xrightarrow{T\sigma} & S;F;T \\ \sigma \downarrow & & & \swarrow \sigma_S & \\ S;F & \xleftarrow[F\mu^S]{} & S^2;F & & \end{array}$$

Distributive laws naturally arise for the following reason.

Lemma 7.8 ([Appelgate 1965]). *Distributive laws $\sigma : F; T \longrightarrow S; F$ are in 1-1 correspondence with liftings of $F : C \longrightarrow \mathcal{D}$ to a functor between the Eilenberg-Moore categories: $G : C^S \longrightarrow \mathcal{D}^T$ such that*

$$\begin{array}{ccc} C & \xrightarrow{F} & \mathcal{D} \\ \uparrow & & \uparrow \\ C^S & \xrightarrow[G]{} & \mathcal{D}^T \end{array}$$

In many cases, we obtain bilimit compact expansions from Kleisli adjunctions for some partiality monad. We turn to that case next.

Theorem 7.9 (Monad Liftings). *Let $\mathcal{V}_1, \mathcal{V}_2$ be $\boldsymbol{\omega}$**CPO**-enriched categories. Suppose that $((-)^1_\perp, \mathrm{return}^1, \mu^1)$ is a locally continuous monad on $\mathcal{V}_1$ and $((-)^2_\perp, \mathrm{return}^2, \mu^2)$ is a locally continuous monad on $\mathcal{V}_2$. Suppose further, that we are given a locally continuous functor $F_V : \mathcal{V}_1 \longrightarrow \mathcal{V}_2$ together with a distributive law $\sigma : F_V; (-)^2_\perp \longrightarrow (-)^1_\perp; F_V$. Then, we obtain a locally continuous monad $(-)_{\tilde{\perp}}$ (which lifts $(-)^2_\perp$ and $(-)^1_\perp$) on $\mathcal{V}_2/F_V$ by defining*

$$(V_2, f, V_1)_{\tilde{\perp}} \overset{\mathrm{def}}{=} (V_2{}^2_\perp, f^2_\perp; \sigma, V_1{}^1_\perp)$$

$$\tilde{\mathrm{return}}_{(V_2,f,V_1)} \overset{\mathrm{def}}{=} (\mathrm{return}_{V_2}, \mathrm{return}_{V_1})$$

$$\tilde{\mu}_{(V_2,f,V_1)} \overset{\mathrm{def}}{=} (\mu_{V_2}, \mu_{V_1}).$$

*For any $\boldsymbol{\omega}$**CPO**-enriched orthogonal factorization system $(\mathcal{E}, \mathcal{M})$ on $\mathcal{V}_2$ such that $\mathcal{M}$ is closed under $(-)^2_\perp$ and contains $\sigma$, $(-)_{\tilde{\perp}}$ restricts to a locally continuous monad on $\mathcal{V}_2//F_V$ which is a lifting of the monad $(-)^2_\perp$.*

*Now, suppose that $(-)^1_\perp$ and $(-)^2_\perp$ are strong monads with strengths $t^1$ and $t^2$, respectively, such that $\mathrm{id} \times \sigma; F(t^1) = t^2; \sigma$. In case $\mathcal{V}_1$ and $\mathcal{V}_2$ have finite products and $F_V$ preserves them, $(-)_{\tilde{\perp}}$ gives a strong monad on $\mathcal{V}_2/F_V$. If we further assume that $\mathcal{M}$ is closed under finite products, $(-)_{\tilde{\perp}}$ gives a strong monad on $\mathcal{V}_2//F_V$. The strength of $(-)_{\tilde{\perp}}$ is given by the pair $(t^2, t^1)$.*

Proof. The claims about $(-)_{\tilde{\perp}}$ on $\mathcal{V}_2/F_V$ are all shown in detail in [Goubault-Larrecq et al. 2002] with the exception that local continuity of $(-)_{\tilde{\perp}}$ is not shown. Observe that sups of $\omega$-chains $(g^n_2, g^n_1)_{n\in\mathbb{N}}$ in $\mathcal{V}_2/F_V$ are computed as they are in $\mathcal{V}_2 \times \mathcal{V}_1$, while $(-)_{\tilde{\perp}}$ acts as the locally continuous monad $(-)^2_\perp \times (-)^1_\perp$. We see that $(-)_{\tilde{\perp}}$ is locally continuous on $\mathcal{V}_2/F_V$.

Clearly, $(-)_{\tilde{\perp}}$ restricts to a monad on the full (reflective) subcategory $\mathcal{M} \cap \mathcal{V}_2/F_V = \mathcal{V}_2//F_V \hookrightarrow \mathcal{V}_2/F_V$ in case $\mathcal{M}$ is closed under $(-)^2_\perp$ and it contains $\sigma$. To see that $(-)_{\tilde{\perp}}$ is also locally continuous on $\mathcal{V}_2//F_V$ observe that $(-)^{\mathcal{V}_2//F_V}_{\tilde{\perp}}$ equals $i; (-)^{\mathcal{V}_2/F_V}_{\tilde{\perp}}; a$ where $a \dashv i : \mathcal{V}_2//F_V \leftrightarrows \mathcal{V}_2/F_V$ is the reflexive embedding which is locally continuous by the assumption that $(\mathcal{E}, \mathcal{M})$ is a $\boldsymbol{\omega}$**CPO**-enriched factorization system. □

*Definition 7.10 (Co-distributive law of monads).* Suppose we are given two categories each equipped with a monad, $(C, S, \mathrm{return}^S, \mu^S)$ and $(\mathcal{D}, T, \mathrm{return}^T, \mu^T)$, together with a functor $F$ :

$\mathcal{C} \to \mathcal{D}$. Then, a natural transformation $\tau : S; F \to F; T$ is called a *co-distributive law* if it satisfies:

$$\begin{array}{ccc} F & \xrightarrow{\text{return}^T} & F;T \\ & \searrow^{F\text{return}^S} & \uparrow \tau \\ & & S;F \end{array} \qquad \begin{array}{ccccc} F;T & \xleftarrow{\mu^T_F} & F;T^2 & \xleftarrow{T\tau} & S;F;T \\ \uparrow \tau & & & \nearrow \tau_S & \\ S;F & \xleftarrow[F\mu^S]{} & S^2;F & & \end{array}$$

Co-distributive laws naturally arise for the following reason.

Lemma 7.11 ([Mulry 1993]). *Co-distributive laws $\tau : S; F \to F; T$ are in 1-1 correspondence with extensions of $F : \mathcal{C} \to \mathcal{D}$ to a functor between the Kleisli categories: $H : \mathcal{C}_S \to \mathcal{D}_T$ such that*

$$\begin{array}{ccc} \mathcal{C} & \xrightarrow{F} & \mathcal{D} \\ \downarrow & & \downarrow \\ \mathcal{C}_S & \xrightarrow[H]{} & \mathcal{D}_T. \end{array}$$

*Here, we have that $H(A \xrightarrow{f} SB) \stackrel{\text{def}}{=} FA \xrightarrow{Ff} F(SB) \xrightarrow{\tau} T(FB)$.*

We can easily see from the definition of $H$ in the lemma above that if we start with a locally continuous functor $F$ and $S$ and $T$ are locally continuous monads, then $H$ will be locally continuous.

Suppose that we are in the situation of theorem 7.9 and we have a right inverse $\tau$ to $\sigma$ (making $\sigma$ a split mono) which is a co-distributive law. Then, we get a functor $F_C : \mathcal{V}_{1\perp} \to \mathcal{V}_{2\perp}$ between the Kleisli categories of $(-)^1_\perp$ and $(-)^2_\perp$ by $F_C(A \xrightarrow{f} B^1_\perp) \stackrel{\text{def}}{=} F_V(A) \xrightarrow{F_V(f)} F_V(B^1_\perp) \xrightarrow{\tau} (F_V B)^2_\perp$. Then, we have a commutative diagram

$$\begin{array}{ccc} \mathcal{V}_1 & \xhookrightarrow{\mathcal{J}_1} & \mathcal{V}_{1\perp} \\ \downarrow F_V & & \downarrow F_C \\ \mathcal{V}_2 & \xhookrightarrow{\mathcal{J}_2} & \mathcal{V}_{2\perp}. \end{array}$$

The question rises what happens in case the Kleisli adjunctions give bilimit compact expansions of $\mathcal{V}_1$ and $\mathcal{V}_2$. In that setting, we have two candidates for bilimit compact expansions of the (sub)scones $\mathcal{V}_2/F_V$ and $\mathcal{V}_2//F_V$:

- by theorems 7.2 and 7.5, the (sub)scones induced by the functors $\mathcal{J}_1$, $\mathcal{J}_2$ and $F_V$ and $F_C$:
$$\mathcal{J}_2/F : \mathcal{V}_2/F_V \hookrightarrow \mathbf{Mix}(\mathcal{V}_2/F_V, C_2/F_C)$$
$$\mathcal{J}_2//F : \mathcal{V}_2//F_V \hookrightarrow \mathbf{Mix}(\mathcal{V}_2//F_V, C_2//F_C)$$
- by theorem 7.9, the Kleisli adjunctions for the induced monads $(-)_{\tilde{\perp}}$ on $\mathcal{V}_2/F_V$ and $\mathcal{V}_2//F_V$:
$$\mathcal{V}_2/F_V \hookrightarrow (\mathcal{V}_2/F_V)_{\tilde{\perp}}$$
$$\mathcal{V}_2//F_V \hookrightarrow (\mathcal{V}_2//F_V)_{\tilde{\perp}}.$$

As we'll see, in general, they need not coincide.

Proposition 7.12. *Let $\mathcal{J}_1 : \mathcal{V}_1 \to C_1 = \mathcal{V}_{1\perp}$ and $\mathcal{J}_2 : \mathcal{V}_2 \to C_2 = \mathcal{V}_{2\perp}$ be bilimit compact expansions given by the Kleisli adjunctions of some locally continuous monads $(-)_\perp$. And suppose that we are given a functor $F_V : \mathcal{V}_1 \to \mathcal{V}_2$ with a split mono distributive law $\sigma : F_V; (-)^2_\perp \to (-)^1_\perp; F_V$ whose right inverse $\tau$ is a co-distributive law such that the induced functor $F_C : C_1 \to C_2$ is $\omega\mathbf{CPO}_\perp$-enriched. Then, we have a commutative square of $\omega\mathbf{CPO}$-enriched functors where the horizontal ones are lluf and faithful and right one is faithful, order-reflecting and bijective on objects and, in case $\sigma$ is an iso, also full in the enriched sense:*

$$\begin{array}{ccc} \mathcal{V}_2/F_V & \xhookrightarrow{\text{lluf}} & (\mathcal{V}_2/F_V)_{\tilde{\bot}} \\ \Big\| & & \Big\downarrow \text{lluf} \\ \mathcal{V}_2/F_V & \xhookrightarrow[\text{lluf}]{\mathcal{J}_2/F} & \mathbf{Mix}(\mathcal{V}_2/F_V, C_2/F_C). \end{array}$$

*That is, the Kleisli adjunction on the scone is equivalent to a lluf subcategory of the scone of the bilimit compact expansion. This subcategory coincides with the entire category if $\sigma$ is an iso.*

*Let $(\mathcal{E}', \mathcal{M}')$ be a $\mathcal{J}_2$-compatible $\omega$CPO-enriched factorization system on $C_2$ which restricts to $(\mathcal{E}, \mathcal{M})$ on $\mathcal{V}_2$. Moreover, assume that $\mathcal{M}$ is closed under $(-)_\bot$ and $\sigma \in \mathcal{M}$, so that $(-)_{\tilde{\bot}}$ restricts to $\mathcal{V}_2//F_V$. Then, the diagram above restricts to the subscones*

$$\begin{array}{ccc} \mathcal{V}_2//F_V & \xhookrightarrow{\text{lluf}} & (\mathcal{V}_2//F_V)_{\tilde{\bot}} \\ \Big\| & & \Big\downarrow \text{lluf} \\ \mathcal{V}_2//F_V & \xhookrightarrow[\text{lluf}]{\mathcal{J}_2/F} & \mathbf{Mix}(\mathcal{V}_2//F_V, C_2//F_C). \end{array}$$

*Again, in case $\sigma$ is full, $\mathbf{Mix}(\mathcal{V}_2//F_V, C_2//F_C)$ and $(\mathcal{V}_2//F_V)_{\tilde{\bot}}$ coincide.*

Proof. First, let us consider the scone. Observe that the total map categories $\mathcal{V}_2/F_V$ coincide. Therefore, we turn our attention to comparing the partial map categories $(\mathcal{V}_2/F_V)_{\tilde{\bot}}$ and $\mathbf{Mix}(\mathcal{V}_2/F_V, C_2/F_C)$.

Observe that objects in $(\mathcal{V}_2/F_V)_{\tilde{\bot}}$ are triples $(X_2, X_2 \xrightarrow{f} F_V X_1, X_1)$ and morphisms are pairs $(g_2, g_1)$ such that the following square commutes

$$\begin{array}{ccccc} (X_2)_\bot & \xrightarrow{f_\bot} & (F_V X_2')_\bot & \xrightarrow{\sigma} & F_V((X_1)_\bot) \\ {\scriptstyle g_2}\Big\uparrow & & & & \Big\uparrow{\scriptstyle F_V g_1} \\ X_2' & & \xrightarrow[f']{\hspace{6em}} & & F_V X_1'. \end{array}$$

Meanwhile, objects in $\mathbf{Mix}(\mathcal{V}_2/F_V, C_2/F_C)$ are triples $(X_2, X_2 \xrightarrow{\tilde{f}} F_V X_1, X_1)$ and morphisms are pairs $(g_2, g_1)$ such that the following square commutes

$$\begin{array}{ccc} (X_2)_\bot & \xrightarrow{\tilde{f}_\bot} & (F_V X_1)_\bot \\ {\scriptstyle g_2}\Big\uparrow & & \Big\uparrow{\scriptstyle F_V g_1;\tau} \\ X_2' & \xrightarrow[\tilde{f}']{} & (F_V X_1'). \end{array}$$

Therefore we obtain a functor $(\mathcal{V}_2/F_V)_{\tilde{\bot}} \to \mathbf{Mix}(\mathcal{V}_2/F_V, C_2/F_C)$ by acting on objects and morphisms as the identity: indeed, $g_2; f_\bot; \sigma = f'; F_V g_1$ implies that

$$\begin{aligned} g_2; f_\bot &= g_2; f_\bot; \sigma; \tau \\ &= f'; F_V g_1; \tau \\ &= f'; F_V g_1; \tau, \end{aligned}$$

using the fact that $\tau$ is right inverse to $\sigma$. This functor is evidently bijective on objects, faithful, locally continuous, and order reflecting. To see that it is full if $\sigma$ is an iso, note that $g_2; f_\bot = f'; F_V g_1; \tau$

implies that

$$\begin{aligned} g_2; f_\perp; \sigma &= f'; F_V g_1; \tau; \sigma \\ &\quad \overset{\text{using } \tau;\sigma = \mathrm{id}}{\downarrow} \\ &= f'; F_V g_1. \end{aligned}$$

In case $\sigma$ is not an iso, observe that the homset $(\mathcal{V}_2/F_V)_{\tilde{\perp}}(f', f)$ consists precisely of those $(g_2, g_1)$ in $\mathbf{Mix}(\mathcal{V}_2/F_V, C_2/F_C)(f', f)$ such that $f'; F_V g_1; \tau; \sigma = f'; F_V g_1$.

Next, let us consider the subscone. Observe that the total map categories $\mathcal{V}_2//F_V$ coincide. Therefore, we turn our attention to comparing the partial map categories $(\mathcal{V}_2//F_V)_{\tilde{\perp}}$ and $\mathbf{Mix}(\mathcal{V}_2//F_V, C_2//F_C)$.

Observe that objects in $(\mathcal{V}_2//F_V)_{\tilde{\perp}}$ are triples $(X_2, X_2 \xrightarrow{m} F_V X_1, X_1)$ with $m \in \mathcal{M}$ and morphisms are pairs $(g_2, g_1)$ such that the following square commutes

$$\begin{array}{ccccc} (X_2)_\perp & \xrightarrow{m_\perp} & (F_V X_2')_\perp & \xrightarrow{\sigma} & F_V((X_1)_\perp) \\ {\scriptstyle g_2}\uparrow & & & & \uparrow{\scriptstyle F_V g_1} \\ X_2' & & \xrightarrow[m']{} & & F_V X_1'. \end{array}$$

Meanwhile, objects in $\mathbf{Mix}(\mathcal{V}_2//F_V, C_2//F_C)$ are triples $(X_2, X_2 \xrightarrow{\tilde{m}} F_V X_1, X_1)$ such that $\tilde{m} \in \mathcal{M}$ and morphisms are pairs $(g_2, g_1)$ such that the following square commutes

$$\begin{array}{ccc} (X_2)_\perp & \overset{\tilde{m}_\perp}{\rightarrowtail} & (F_V X_1)_\perp \\ {\scriptstyle g_2}\uparrow & & \uparrow{\scriptstyle F_V g_1;\tau} \\ X_2' & \underset{}{\overset{\tilde{m}'}{\rightarrowtail}} & F_V X_1'. \end{array}$$

Therefore our previous enriched faithful (and full in case $\sigma$ is an iso) functor $(\mathcal{V}_2/F_V)_{\tilde{\perp}} \to \mathbf{Mix}(\mathcal{V}_2/F_V, C_2/F_C)$ restricts to one $(\mathcal{V}_2//F_V)_{\tilde{\perp}} \to \mathbf{Mix}(\mathcal{V}_2//F_V, C_2//F_C)$. Again, it is bijective on objects. □

As the previous proposition shows that $(\mathcal{V}_2/F_V)_{\tilde{\perp}}$ might in general be a proper subcategory of $\mathbf{Mix}(\mathcal{V}_2/F_V, C_2/F_C)$, we cannot directly conclude from theorem 7.2 that it is bilimit compact. Therefore, we separately consider bilimit compactness of $(\mathcal{V}_2/F_V)_{\tilde{\perp}}$.

Theorem 7.13 (Bilimit Compactness of Lifted Kleisli Category). *Suppose the conditions of theorem 7.9 are met such that we obtain a lifted locally continuous monad $(-)_{\tilde{\perp}}$ on the scone $\mathcal{V}_2/F_V$. Let us further assume that*

*(1) every embedding $a^e$ in $(\mathcal{V}_1)_\perp$ is a morphism in $\mathcal{V}_1$ (factors over* return*);*
*(2) $F_V(\perp^p) = \perp^p; (?_{F_V \mathbb{0}})_\perp; \sigma$;*
*(3) $\sigma$ is a split mono with right inverse $\tau$ which is a codistributive law $(-)_\perp; F_V \to F_V; (-)_\perp$;*

*And suppose that the Kleisli adjunctions for $(-)^1_\perp$ and $(-)^2_\perp$ give bilimit compact expansions. Then, the Kleisli adjunction of $(-)_{\tilde{\perp}}$ also gives a bilimit compact expansion.*

*Further, if we are given a $\boldsymbol{\omega}$***CPO***-enriched factorization system $(\mathcal{E}, \mathcal{M})$ on $\mathcal{V}_2$ such that $\sigma \in \mathcal{M}$ and $\mathcal{M}$ is closed under $(-)^2_\perp$, we have seen in theorem 7.9 that $(-)_{\tilde{\perp}}$ restricts to the subscone $\mathcal{V}_2//F_V$. Then its Kleisli adjunction also gives a bilimit compact expansion.*

Proof. We will use assumption (1) throughout and write ep-pairs $a$ in $\mathcal{V}_1$ as $(a^e; \mathrm{return}; a^p)$.

We have already seen that $\mathcal{V}_2/F_V$ is $\boldsymbol{\omega}\mathbf{CPO}$-enriched and that $(-)_{\tilde{\perp}}$ gives a $\boldsymbol{\omega}\mathbf{CPO}$-enriched monad. Therefore, the Kleisli category $(\mathcal{V}_2/F_V)_{\tilde{\perp}}$ is $\boldsymbol{\omega}\mathbf{CPO}$-enriched.

We show that $(\mathcal{V}_2/F_V)_{\tilde{\perp}}$ is bilimit compact.

First, we claim that $(\mathbb{0}, ?_{F_V\mathbb{0}}, \mathbb{0})$ gives an ep-zero object for $(\mathcal{V}_2/F_V)_{\tilde{\bot}}$, where $?_{F_V\mathbb{0}}$ is the unique morphism $\mathbb{0} \longrightarrow F_V\mathbb{0}$. (Noting that the zero object of $(\mathcal{V}_2)_\bot$ has to coincide with the initial object of $\mathcal{V}_2$.) Indeed, let $(C_2, f, C_1)$ be any object in $(\mathcal{V}_2/F_V)_{\tilde{\bot}}$. Then, we get a unique morphism $\mathbb{0} \xrightarrow{\bot^{\mathrm{e}};\mathrm{return}} (C_1)_\bot$ in $\mathcal{V}_1$ and a unique morphism $\mathbb{0} \xrightarrow{\bot^{\mathrm{e}}} (C_2)_\bot$ in $\mathcal{V}_2$, both of which are embeddings, while the diagram below commutes by initiality of $\mathbb{0}$ in $\mathcal{V}_2$:

$$\begin{array}{ccccc}
(C_2)_\bot & \xrightarrow{f_\bot} & (F_V C_1)_\bot & \xrightarrow{\sigma} & F_V(C_1)_\bot \\
\uparrow{\scriptstyle \bot^{\mathrm{e}}} & & & & \uparrow{\scriptstyle F_V(\bot^{\mathrm{e}};\mathrm{return})} \\
\mathbb{0} & & \xrightarrow[?_{F_V\mathbb{0}}]{} & & F_V\mathbb{0}.
\end{array}$$

We see that $(\mathbb{0}, ?_{F_V\mathbb{0}}, \mathbb{0})$ is an initial object in $(\mathcal{V}_2/F_V)_{\tilde{\bot}}$ and every morphism into it is an embedding, as the pair of two embeddings. To see that it is also terminal, observe that we have unique morphisms $\bot^{\mathrm{p}} : C_2 \longrightarrow \mathbb{0}_\bot$ in $(\mathcal{V}_2)_\bot$ and $\bot^{\mathrm{p}} : C_1 \longrightarrow \mathbb{0}_\bot$ in $(\mathcal{V}_1)_\bot$ and that the following diagram commutes, where the left triangle commutes by terminality of $\mathbb{0}$ in $(\mathcal{V}_2)_\bot$ and the right quadrangle commutes by assumption (2):

$$\begin{array}{ccccc}
\mathbb{0}_\bot & \xrightarrow{(?_{F_V\mathbb{0}})_\bot} & (F_V\mathbb{0})_\bot & \xrightarrow{\sigma} & F_V(\mathbb{0}_\bot) \\
\uparrow{\scriptstyle \bot^{\mathrm{p}}} & \nwarrow{\scriptstyle \bot^{\mathrm{p}}} & & & \uparrow{\scriptstyle F_V(\bot^{\mathrm{p}})} \\
C_2 & & \xrightarrow[f]{} & & F_V C_1.
\end{array}$$

As a pair of projections, every morphism into $(\mathbb{0}, ?_{F_V\mathbb{0}}, \mathbb{0})$ is a projection. We see that $(\mathbb{0}, ?_{F_V\mathbb{0}}, \mathbb{0})$ is an ep-zero object.

Next, suppose that $((C_2^n, f^n, C_1^n)_{n\in\mathbb{N}}, (g_2^n, g_1^n)_{n\in\mathbb{N}})$ is an $\omega$-chain of ep-pairs in $(\mathcal{V}_2/F_V)_{\tilde{\bot}}$. In particular, $(g_2^n)_{n\in\mathbb{N}}$ is an $\omega$-chain of ep-pairs in $\mathcal{V}_{2\bot}$ and $(g_1^n)_{n\in\mathbb{N}}$ is an $\omega$-chain of ep-pairs in $\mathcal{V}_{1\bot}$ while $(*)$

$$\begin{array}{ccccc}
(C_2^{n+1})_\bot & \xrightarrow{{f^{n+1}}_\bot} & (F_V C_1^{n+1})_\bot & \xrightarrow{\sigma} & F_V((C_1^{n+1})_\bot) \\
\uparrow{\scriptstyle g_2^{n\mathrm{e}}} & & & & \uparrow{\scriptstyle F_V(g_1^{n\mathrm{e}};\mathrm{return})} \\
C_2^n & & \xrightarrow[f^n]{} & & F_V C_1^n
\end{array}
\qquad
\begin{array}{ccccc}
(C_2^n)_\bot & \xrightarrow{{f^n}_\bot} & (F_V C_1^n)_\bot & \xrightarrow{\sigma} & F_V((C_1^n)_\bot) \\
\uparrow{\scriptstyle g_2^{n\mathrm{p}}} & & & & \uparrow{\scriptstyle F_V g_1^{n\mathrm{p}}} \\
C_2^{n+1} & & \xrightarrow[f^{n+1}]{} & & F_V C_1^{n+1}.
\end{array}$$

Let $(C_2^\omega, d_2)$ be the bilimit of $(g_2^n)_{n\in\mathbb{N}}$ in $(\mathcal{V}_2)_\bot$ and let $(C_1^\omega, d_1)$ be the bilimit of $(g_1^n)_{n\in\mathbb{N}}$ in $(\mathcal{V}_1)_\bot$. Observe that, by assumption (3), the codistributive law $\tau$ gives us a locally continuous functor $F_C : \mathcal{V}_{1\bot} \longrightarrow \mathcal{V}_{2\bot}$ which acts on objects as $F_V$ and morphisms as $f \mapsto F_V(f); \tau$ while it acts on total morphisms $f;\mathrm{return}$ as $F_V(f;\mathrm{return}); \tau = F_V(f);\mathrm{return}$. As $F_C$ is locally continuous, it preserves bilimits, so $(F_C g_1^n)_{n\in\mathbb{N}}$ is an $\omega$-chain of ep-pairs in $\mathcal{V}_{2\bot}$ with bilimit $(F_V C_1^\omega, (F_C d_1^n)_{n\in\mathbb{N}})$.

Observe that $(f^n)_{n\in\mathbb{N}}$ defines a natural transformation $g_2 \longrightarrow F_C g_1$ in the sense that

$$\begin{aligned}
g_2^{n\mathrm{e}}; {f^{n+1}}_\bot &= f^n; F_V(g_1^{n\mathrm{e}}; \mathrm{return}); \tau = f^n; F_C(g_1^{n\mathrm{e}}; \mathrm{return}) \\
g_2^{n\mathrm{p}}; {f^n}_\bot &= f^{n+1}; F_V g_1^{n\mathrm{p}}; \tau = f^{n+1}; F_C g_1^{n\mathrm{p}}.
\end{aligned}$$

Indeed, we obtain these equations by postcomposing the two commuting squares $(*)$ with $\tau$ and using the fact that $\tau$ is right inverse to $\sigma$.

As $\mathcal{V}_{2\bot}$ is a bilimit compact expansion of $\mathcal{V}_2$, we now obtain a (unique) $f^\omega : C_2^\omega \longrightarrow F_V C_1^\omega$ such that

$$f^\omega; \mathrm{return} = \bigvee_n d_2^{n\mathrm{p}}; {f^n}_\bot; \gg\!= F_C(d_1^{n\mathrm{e}}; \mathrm{return}) = \bigvee_n d_2^{n\mathrm{p}}; {f^n}_\bot; F_V(d_1^{n\mathrm{e}})_\bot.$$

Now, it follows that $\mathcal{V}_2/F_{V\,\tilde{\bot}}$ is bilimit compact once we show that the following diagrams commute:

$$\begin{array}{ccccc}
(C_2^{\omega})_{\bot} & \xrightarrow{f^{\omega}{}_{\bot}} & (F_V C_1^{\omega})_{\bot} & \xrightarrow{\sigma} & F_V((C_1^{\omega})_{\bot}) \\
{\scriptstyle d_2^{n\mathrm{e}}}\uparrow & & & & \uparrow{\scriptstyle F_V(d_1^{n\mathrm{e}};\mathrm{return})} \\
C_2^n & & \xrightarrow[f^n]{\qquad\qquad} & & F_V C_1^n
\end{array}
\qquad
\begin{array}{ccccc}
(C_2^{n})_{\bot} & \xrightarrow{f^{n}{}_{\bot}} & (F_V C_1^{n})_{\bot} & \xrightarrow{\sigma} & F_V((C_1^{n})_{\bot}) \\
{\scriptstyle d_2^{n\mathrm{p}}}\uparrow & & & & \uparrow{\scriptstyle F_V d_1^{n\mathrm{p}}} \\
C_2^{\omega} & & \xrightarrow[f^{\omega}]{\qquad\qquad} & & F_V C_1^{\omega}.
\end{array}$$

Indeed, it then follows that $(f^{\omega}, (d_2, d_1))$ is a bilimit for $\big((f^n, (g_2^n, g_1^n))\big)_{n\in\mathbb{N}}$.

We verify that they commute:

$$\begin{aligned}
f^{\omega}; F_V(d_1^{n\mathrm{p}}) &= f^{\omega}; \mathrm{return}; \sigma; F_V(\gg\!= d_1^{n\mathrm{p}}) \\
&= \left(\bigvee_k d_2^{k\mathrm{p}}; f^k{}_{\bot}; F_V(d_1^{k\mathrm{e}})_{\bot}\right); \sigma; F_V(\gg\!= d_1^{n\mathrm{p}}) \\
&= \left(\bigvee_k d_2^{k\mathrm{p}}; f^k{}_{\bot}; F_V(d_1^{k\mathrm{e}})_{\bot}; \sigma\right); F_V(\gg\!= d_1^{n\mathrm{p}}) \\
&= \left(\bigvee_k d_2^{k\mathrm{p}}; f^k{}_{\bot}; \sigma; F_V(d_1^{k\mathrm{e}}{}_{\bot})\right); F_V(\gg\!= d_1^{n\mathrm{p}}) \\
&= \left(\bigvee_k d_2^{k\mathrm{p}}; f^k{}_{\bot}; \sigma; F_V(d_1^{k\mathrm{e}}{}_{\bot}; \gg\!= d_1^{n\mathrm{p}})\right) \\
&= d_2^{n\mathrm{p}}; f^n{}_{\bot}; \sigma
\end{aligned}$$

and

$$\begin{aligned}
f^n; F_V(d_1^{n\mathrm{e}}; \mathrm{return}) &= f^n; F_V(d_1^{n\mathrm{e}}); F_V\mathrm{return} \\
&= f^n; F_V\mathrm{return}; F_V((d_1^{n\mathrm{e}})_{\bot}) \\
&= f^n; \mathrm{return}; \sigma; F_V((d_1^{n\mathrm{e}})_{\bot}) \\
&= \mathrm{return}; f^n{}_{\bot}; \sigma; F_V((d_1^{n\mathrm{e}})_{\bot}) \\
&= \mathrm{return}; f^n{}_{\bot}; F_V(d_1^{n\mathrm{e}})_{\bot}; \sigma \\
&= \big(\mathrm{return}; f^n{}_{\bot}; F_V(d_1^{n\mathrm{e}})_{\bot}\big); \sigma \\
&= \left(\bigvee_k d_2^{n\mathrm{e}}; \gg\!= d_2^{k\mathrm{p}}; f^k{}_{\bot}; F_V(d_1^{k\mathrm{e}})_{\bot}\right); \sigma \\
&= d_2^{n\mathrm{e}}; \gg\!= \left(\bigvee_k d_2^{k\mathrm{p}}; f^k{}_{\bot}; F_V(d_1^{k\mathrm{e}})_{\bot}\right); \sigma \\
&= d_2^{n\mathrm{e}}; \gg\!= (f^{\omega}; \mathrm{return}); \sigma \\
&= d_2^{n\mathrm{e}}; f^{\omega}{}_{\bot}; \sigma.
\end{aligned}$$

We see that $\mathcal{V}_2/F_{V\,\tilde{\bot}}$ is bilimit compact.

Next, we show that $\mathcal{V}_2/F_V \hookrightarrow \mathcal{V}_2/F_{V\,\tilde{\bot}}$ is a bilimit compact expansion. By theorem 7.2 and proposition 7.12, we have that $\mathcal{J}_2/F : \mathcal{V}_2/F_V \hookrightarrow \mathcal{V}_2/F_{V\,\tilde{\bot}} \hookrightarrow \mathbf{Mix}(\mathcal{V}_2/F_V, \mathcal{V}_{2\bot}/F_C)$ is a bilimit compact expansion and $\mathcal{V}_2/F_{V\,\tilde{\bot}} \hookrightarrow \mathbf{Mix}(\mathcal{V}_2/F_V, \mathcal{V}_{2\bot}/F_C)$ is identity-on-objects, locally continuous and order reflecting. As a consequence $J : \mathcal{V}_2/F_V \hookrightarrow \mathcal{V}_2/F_{V\,\tilde{\bot}}$ is also identity-on-objects, locally continuous and order reflecting. Suppose that we have ep-pair $\omega$-chains $(A, a)$, $(B, b)$ in $\mathcal{V}_2/F_{V\,\tilde{\bot}}$ with bilimits $(D, d)$, $(E, e)$, and countable collection of $\mathcal{V}_2/F_V$-morphisms $(\alpha_n : A_n \to B_n)_{n\in\mathbb{N}}$ such

that for all $n$:

$$a^{\mathrm{e}}_n; J\alpha_{n+1} = J\alpha_n; b^{\mathrm{e}}_n, \qquad a^{\mathrm{p}}_n; J\alpha_n = J\alpha_{n+1}; b^{\mathrm{p}}_n.$$

Then, as $\mathcal{V}_2/F_{V\,\tilde{\bot}} \hookrightarrow \mathbf{Mix}(\mathcal{V}_2/F_V, \mathcal{V}_{2\bot}/F_C)$ is locally continuous, $(A, a)$, $(B, b)$ also define $\omega$-chains in $\mathbf{Mix}(\mathcal{V}_2/F_V, \mathcal{V}_{2\bot}/F_C)$ with bilimits $(D, d)$, $(E, e)$, satisfying the same equations. As $\mathcal{J}_2/F$ is a bilimit compact expansion, we have a (unique) $\mathcal{V}_2/F_V$-morphism $f : D \to E$ such that $(\mathcal{J}_2/F)f = \bigvee_n d^{\mathrm{p}}_n; \alpha_n; e^{\mathrm{e}}_n$ and so also $Jf = \bigvee_n d^{\mathrm{p}}_n; \alpha_n; e^{\mathrm{e}}_n$ as $\mathcal{V}_2/F_{V\,\tilde{\bot}} \hookrightarrow \mathbf{Mix}(\mathcal{V}_2/F_V, \mathcal{V}_{2\bot}/F_C)$ is locally continuous. We see that $J$ is a bilimit compact expansion.

Finally, we observe that $\mathcal{V}_2//F_V$ is a $\boldsymbol{\omega}$**CPO**-enriched reflective subcategory of $\mathcal{V}_2/F_V$ as $(\mathcal{E}, \mathcal{M})$ is a $\boldsymbol{\omega}$**CPO**-enriched orthogonal factorization system. Further, in case $(-)_{\tilde{\bot}}$ restricts to $\mathcal{V}_2//F_V$, we have that $\mathcal{V}_2/F_{V\,\tilde{\bot}}(f', m)$ for $m \in \mathcal{M}$ consists of morphisms $(g_2, g_1)$ such that the following square in $\mathcal{V}_2$ commutes, where we write $m' \stackrel{\text{def}}{=} m^2_\bot; \sigma$ and we note that also $m' \in \mathcal{M}$:

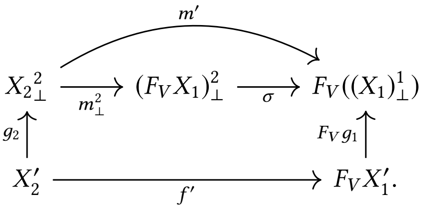


As $(\mathcal{E}, \mathcal{M})$ is an $\boldsymbol{\omega}$**CPO**-enriched orthogonal factorization system on $\mathcal{V}_2$, these are in natural 1-1 correspondence with commuting diagrams

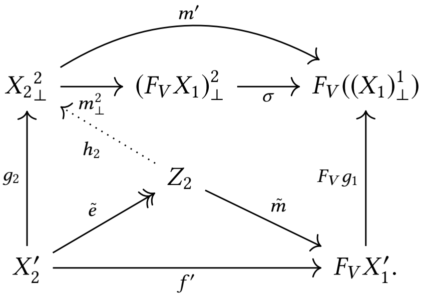


where the assignment $(g_2, g_1) \mapsto h_2$ is $\omega$-continuous. We see that $\mathcal{V}_2//F_{V\,\tilde{\bot}}$ is a $\boldsymbol{\omega}$**CPO**-enriched reflective full subcategory of $\mathcal{V}_2/F_{V\,\tilde{\bot}}$ and that the following square commutes:

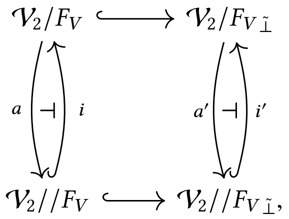


Therefore, it immediately follows by lemma 3.1 that $\mathcal{V}_2//F_V \hookrightarrow \mathcal{V}_2//F_{V\,\tilde{\bot}}$ is also a bilimit compact expansion. □

## 8 CORRECTNESS OF AD FOR RECURSIVE TYPES

In this section, we prove the correctness of forward-mode AD for a language with term and type recursion. We will be a bit sparse on details as this part of the development is almost identical to that for a fine-grain CBV language with iteration, which we have discussed in detail. The only

difference is that we first need to argue that the Kleisli adjunction for our lifted monad on the subscone gives a bilimit compact expansion. The rest then follows as before.

Consider the category $\omega\mathbf{Diff}$ of diffeological predomains with its canonical partiality monad $(-)^1_\perp$ induced by the diffeological space $\mathfrak{M}$ of open subsets: $\mathcal{P}^U_{\mathfrak{M}} \stackrel{\text{def}}{=} O_U$ (where $\mathcal{P}^f_{\mathfrak{M}}(V) \stackrel{\text{def}}{=} f^{-1}(V)$). By the previous development, we know it gives a model of fine-grain CBV FPC over a ground type $\mathbb{R}$ and some $n$-ary total and partial operations op on $\mathbb{R}$. The same is trivially true for the product category $\omega\mathbf{Diff} \times \omega\mathbf{Diff}$.

Further, let us consider the category $\mathbf{Sh}_{\omega\mathbf{CPO}}(O_\mathbb{R})$ of internal $\omega$-cpos in the category $\mathbf{Sh}(O_\mathbb{R})$ of sheaves on the frame of opens of $\mathbb{R}$. We can equip this by its canonical partiality monad $(-)^2_\perp$ induced by the sheaf $\mathfrak{M}$ of open subsets $\mathfrak{M}U = O_U$. This again, gives us a second model of fine-grain CBV FPC.

Observe that the $\mathbb{R}$-indexed plots define a locally continuous functor

$$\mathcal{P}_- \times \mathcal{P}_- : \omega\mathbf{Diff} \times \omega\mathbf{Diff} \to \mathbf{Sh}_{\omega\mathbf{CPO}}(O_\mathbb{R})(X_1, X_2) \qquad \mapsto (U \mapsto \mathcal{P}^U_{X_1} \times \mathcal{P}^U_{X_2})$$

for which we have a distributive law

$$\sigma_{X_1,X_2} : (\mathcal{P}_{X_1} \times \mathcal{P}_{X_2})^2_\perp \subseteq \mathcal{P}_{X_1{}^1_\perp} \times \mathcal{P}_{X_2{}^1_\perp}$$
$$(U \in O_W, (\alpha \in \mathcal{P}^U_{X_1}, \beta \in \mathcal{P}^U_{X_2})) \mapsto ((U, \alpha), (U, \beta)).$$

Lemma 8.1. *$\sigma$ is a distributive law of strong monads.*

Proof. $\sigma$ is clearly natural and $\omega$-continuous in each component. Indeed, it is the inclusion of a full sub-cpo.

We verify the laws in the $W$-component of the corresponding natural transformations.

$$\begin{aligned}
\sigma(\mathrm{return}^2(a_1, a_2)) &= \sigma((W, (a_1, a_2))) \\
&= ((W, a_1), (W, a_2)) \\
&= (\mathcal{P}_- \times \mathcal{P}_-)(\mathrm{return}^1 \times \mathrm{return}^1)(a_1, a_2) \\
\sigma(\mu^2(U, (V, (a_1, a_2)))) &= \sigma((V, (a_1, a_2))) \\
&= ((V, a_1), (V, a_2)) \\
&= (\mathcal{P}_- \times \mathcal{P}_-)(\mu^1 \times \mu^1)(((U, (V, a_1)), (U, (V, a_2)))) \\
&(\mathcal{P}_- \times \mathcal{P}_-)(\mu^1 \times \mu^1)(\sigma(\sigma^1_\perp)(U, (V, (a_1, a_2)))) \\
\sigma(\mathrm{strength}^2((a_1, a_2), (U, (a_1', a_2')))) &= \sigma((U, ((a_1, a_1'), (a_2, a_2')))) \\
&= ((U, (a_1, a_1')), (U, (a_2, a_2'))) \\
&= (\mathcal{P}_- \times \mathcal{P}_-)(\mathrm{strength}^1 \times \mathrm{strength}^1)((a_1, a_2), ((U, a_1'), (U, a_2'))) \\
&= (\mathcal{P}_- \times \mathcal{P}_-)(\mathrm{strength}^1 \times \mathrm{strength}^1)((\mathrm{id} x \sigma)((a_1, a_2), (U, (a_1', a_2')))).
\end{aligned}$$

□

Observe that we have a right inverse $\tau$ to $\sigma$, which is a codistributive law:

$$\tau_{X_1,X_2} : \mathcal{P}_{X_1{}^1_\perp} \times \mathcal{P}_{X_2{}^1_\perp} \to (\mathcal{P}_{X_1} \times \mathcal{P}_{X_2})^2_\perp$$
$$((U \in O_W, \alpha \in \mathcal{P}^U_{X_1}), (V, \beta \in \mathcal{P}^V_{X_2})) \mapsto (U \cap V, (\alpha|_{U \cap V}, \beta|_{U \cap V})).$$

Lemma 8.2. *$\tau$ defines a right inverse to $\sigma$ and it is a codistributive law of monads.*

Proof. Naturality of $\tau$ is obvious. To derive componentwise $\omega$-continuity, the observation is that $O_\mathbb{R}$ forms a complete Heyting algebra. As a consequence, $U \mapsto U \cap V$ has a right adjoint,

meaning that $(U, V) \mapsto U \cap V$ preserves all lubs. $\omega$-continuity now follows because the restriction maps are $\omega$-continuous as we are working with $\omega$-diffeological spaces:

$$\begin{aligned}
\bigvee_i \tau(((U_i, a_i), (V_i b_i))) &= \bigvee_i (U_i \cap V_i, (a_i|_{U_i \cap V_i}, b_i|_{U_i\cap V_i}))\\
&= (\bigvee_i U_i \cap V_i, \mathrm{glue}_i \bigvee_{i'\geq i} (a_{i'}|_{U_{i'}\cap V_{i'}}, b_{i'}|_{U_{i'}\cap V_{i'}}))\\
&= (\bigvee_i U_i \cap V_i, (\mathrm{glue}_i \bigvee_{i'\geq i} a_{i'}|_{U_{i'}\cap V_{i'}}, \mathrm{glue}_i \bigvee_{i'\geq i} b_{i'}|_{U_{i'}\cap V_{i'}}))\\
&= (\bigvee_i U_i \cap V_i, ((\mathrm{glue}_i \bigvee_{i'\geq i} a_{i'}|_{U_i}|_{\bigvee_k U_k \cap V_k}), (\mathrm{glue}_i \bigvee_{i'\geq j} b_{i'}|_{V_i}|_{\bigvee_k U_k\cap V_k})))\\
&= (\bigvee_i U_i \cap V_i, ((\mathrm{glue}_i \bigvee_{i'\geq i} a_{i'}|_{U_i}|_{\bigvee_k U_k \cap V_k}), (\mathrm{glue}_i \bigvee_{i'\geq j} b_{i'}|_{V_i}|_{\bigvee_k U_k\cap V_k})))\\
&= (\bigvee_i U_i \cap V_i, ((\mathrm{glue}_i \bigvee_{i'\geq i} a_{i'}|_{U_i})|_{\bigvee_i U_i \cap V_i}, (\mathrm{glue}_j \bigvee_{j'\geq j} b_{j'}|_{V_j})_{\bigvee_i U_i\cap V_i}))\\
&= ((\bigvee_i U_i) \cap (\bigvee_j V_j), ((\mathrm{glue}_i \bigvee_{i'\geq i} a_{i'}|_{U_i})|_{(\bigvee_i U_i)\cap(\bigvee_j V_j)}, (\mathrm{glue}_j \bigvee_{j'\geq j} b_{j'}|_{V_j})_{(\bigvee_i U_i)\cap(\bigvee_j V_j)}))\\
&= \tau((\bigvee_i U_i, \mathrm{glue}_i \bigvee_{i'\geq i} a_{i'}|_{U_i}), (\bigvee_j V_j, \mathrm{glue}_j \bigvee_{j'\geq j} b_{j'}|_{V_j}))\\
&= \tau(\bigvee_i ((U_i, a_i), (V_i b_i))).
\end{aligned}$$

We verify the laws in the $W$-component of the corresponding natural transformations. $\tau(\sigma(U, (a, b))) = \tau((U, a), (U, b)) = ((U \cap U), (a|_{U\cap U}, b|_{U\cap U})) = (U, (a, b))$. Further,

$$\begin{aligned}
\tau((\mathcal{P}_- \times \mathcal{P}_-)(\mathrm{return}^1 \times \mathrm{return}^1)(a_1, a_2)) &= \tau((W, a_1), (W, a_2))\\
&= (W, (a_1, a_2))\\
&= \mathrm{return}^2(a_1, a_2)\\
\mu^2(\tau^2_\perp(\tau((U, (U', a_1)), (V, (V', a_2))))) &= \mu^2(\tau^2_\perp(\tau(U \cap V, ((U', a_1)|_{U\cap V}, (V', a_2)|_{U\cap V}))))\\
&= \mu^2(U \cap V, (U' \cap V', (a_1|_{U\cap V}|_{U'\cap V'}, a_2|_{U\cap V}|_{U'\cap V'})))\\
&= (U' \cap V', (a_1|_{U'\cap V'}, a_2|_{U'\cap V'}))\\
&= \tau((U', a_1), (V', a_2))\\
&= \tau((\mathcal{P}_- \times \mathcal{P}_-)(\mu^1 \times \mu^1)((U, (U', a_1)), (V, (V', a_2)))).
\end{aligned}$$

□

Further, we can observe that $\sigma$ is a full mono, that every split mono in $\omega\mathbf{Diff}_\perp \times \omega\mathbf{Diff}_\perp$ is total, and that

$$(\mathcal{P}_- \times \mathcal{P}_-)(\perp^{\mathrm{p}}) = \perp^{\mathrm{p}}; (?)_\perp; \sigma$$

(indeed, both equal $((\emptyset, \emptyset), (\emptyset, \emptyset))$).

Lemma 8.3. *Suppose that $f$ is a split mono (in particular, the embedding part of an ep-pair) in $\mathbf{SSh}_{\omega\mathrm{CPO}}(\mathcal{C}, \mathcal{J}, \mathcal{K})_\perp$. Then, $f$ factors over* return.

Proof. Indeed, let $g$ be a right inverse to $f$. Then,

$$\begin{aligned}(\mathrm{id}, \alpha) &= \mathrm{return}\,\alpha \\ &= (f; \ggg= g)(\alpha) \\ &= (\ggg= g)(f^1(\alpha), f^2(\alpha)) \\ &= (g^1(f^2(\alpha)); f^1(\alpha), g^2(f^2(\alpha))).\end{aligned}$$

In particular, $g^1(f^2(\alpha)); f^1(\alpha) = \mathrm{id}$, $f^1(\alpha)$ is a split epi. However, $f^1(\alpha)$ is a mono (in $\mathfrak{M}$), by assumption, so $f^1(\alpha)$ is an iso. We see that $f$ factors over return. □

Therefore, by proposition 6.8 and theorems 7.9 and 7.13, we have the following.

Corollary 8.4. *Let us consider the ($\mathrm{Cl}_{\omega\mathcal{J}}$-dense, $\mathrm{Cl}_{\omega\mathcal{J}}$-closed mono) factorization system on* $\mathbf{Sh}_{\omega\mathbf{CPO}}(\mathcal{O}_\mathbb{R})$. *We obtain a strong monad lifting $(-)_{\tilde{\bot}}$ of $(-)^1_\bot$ and $(-)^2_\bot$ to the subscone* $\mathbf{Sh}_{\omega\mathbf{CPO}}(\mathcal{O}_\mathbb{R})//\mathcal{P}^\mathbb{R}_- \times \mathcal{P}^\mathbb{R}_-$ *(which will automatically be commutative). Moreover, the Kleisli adjunction for this monad gives a bilimit compact expansion.*

To be explicit, the category $\mathbf{Sh}_{\omega\mathbf{CPO}}(\mathcal{O}_\mathbb{R})//\mathcal{P}^\mathbb{R}_- \times \mathcal{P}^\mathbb{R}_-$ of logical relations has objects which are triples $(X_1, X_2, R)$ where $X_1, X_2$ are diffeological predomains and $R$ is a tuple of binary relations $\left(R^U \subseteq \mathcal{P}^U_{X_1} \times \mathcal{P}^U_{X_2}\right)_{U \in \mathcal{O}_\mathbb{R}}$ such that

- each $R^U$ is closed under $\omega$-chains in $\mathcal{P}^U_{X_1} \times \mathcal{P}^U_{X_2}$;
- $R$ forms a presheaf on $\mathcal{O}_\mathbb{R}$: given $(\alpha, \beta) \in R^U$ and $V \in \mathcal{O}_U$, then $(\alpha|_V, \beta|_V) \in R^V$;
- $R$ forms a sheaf on $\mathcal{O}_\mathbb{R}$: given a $V \in \mathcal{O}_\mathbb{R}$, an open cover $\mathcal{U}$ of $V$ and plots $(\alpha, \beta) \in \mathcal{P}^V_{X_1} \times \mathcal{P}^V_{X_2}$ such that $(\alpha|_U, \beta|_U) \in R^U$ for all $U \in \mathcal{U}$, then also $(\alpha, \beta) \in R^V$.

Morphisms $(X_1, X_2, R) \to (Y_1, Y_2, S)$ in $\mathbf{Sh}_{\omega\mathbf{CPO}}(\mathcal{O}_\mathbb{R})//\mathcal{P}^\mathbb{R}_- \times \mathcal{P}^\mathbb{R}_-$ are pairs of morphisms $f_1 : X_1 \to Y_1$ and $f_2 : X_2 \to Y_2$ in $\omega\mathbf{Diff}$ such that for all $U \in \mathcal{O}_\mathbb{R}$, for all $(x_1, x_2) \in R^U$, $(g_1(x_1), g_2(x_2)) \in S^U$. Explicitly, the lifted monad $(-)_{\tilde{\bot}}$ on $\mathbf{Sh}_{\omega\mathbf{CPO}}(\mathcal{O}_\mathbb{R})//\mathcal{P}^\mathbb{R}_- \times \mathcal{P}^\mathbb{R}_-$ defines

$$R^U_{\tilde{\bot}} = \left\{(\alpha_1, \alpha_2) \in \mathcal{P}^U_{X_{1\bot}} \times \mathcal{P}^U_{X_{2\bot}} \mid \alpha_1^{-1}(X_1) = \alpha_2^{-1}(X_2) \quad \wedge \quad (\alpha_1|_{\alpha_1^{-1}(X_1)}, \alpha_2|_{\alpha_2^{-1}(X_2)}) \in R^{\alpha_1^{-1}(X_1)}\right\}.$$

Further, by propositions 7.3 and 7.4, it follows that the subscone $\mathbf{Sh}_{\omega\mathbf{CPO}}(\mathcal{O}_\mathbb{R})//\mathcal{P}^\mathbb{R}_- \times \mathcal{P}^\mathbb{R}_-$ lifts the bicartesian closed structure of $\omega\mathbf{Diff} \times \omega\mathbf{Diff}$.

Corollary 8.5. $\mathbf{Sh}_{\omega\mathbf{CPO}}(\mathcal{O}_\mathbb{R})//\mathcal{P}^\mathbb{R}_- \times \mathcal{P}^\mathbb{R}_-$ *gives a model of CBV FPC, which lifts the model in* $\omega\mathbf{Diff} \times \omega\mathbf{Diff}$.

Now, consider CBV FPC extended with a type **real** of real numbers and some total and partial operations op. Observe that we have a natural interpretation $[\![-]\!]$ of this language in $\omega\mathbf{Diff}$ by setting $[\![\mathbf{real}]\!] = \mathbb{R}$ and by interpreting each operation op by a total or partial smooth function of the correct arity. If we have a forward-mode AD macro $\overrightarrow{\mathcal{D}}$ on our language, which is structure preserving[4] we can define an interpretation $([\![-]\!], [\![\overrightarrow{\mathcal{D}}(-)]\!])$ of our language in $\omega\mathbf{Diff} \times \omega\mathbf{Diff}$. As long as we have chosen our semantics for the operations op to have the correct derivatives, meaning

[4]Here, the novel part is that $\overrightarrow{\mathcal{D}}$ is defined on recursive type constructors and destructors as follows:

$$\overrightarrow{\mathcal{D}}_\mathcal{V}(v.\mathbf{roll}\tau) \stackrel{\mathrm{def}}{=} \overrightarrow{\mathcal{D}}_\mathcal{V}(v).\mathbf{roll}\overrightarrow{\mathcal{D}}(\tau)$$

$$\overrightarrow{\mathcal{D}}_C(\mathbf{case}\ v\ \mathbf{of\ roll}\ x \to t) \stackrel{\mathrm{def}}{=} \mathbf{case}\ \overrightarrow{\mathcal{D}}_\mathcal{V}(v)\ \mathbf{of\ roll}\ x \to \overrightarrow{\mathcal{D}}_C(t).$$

Observe that this induces the following AD rule for term recursion (which can be defined as sugar in FPC):

$$\overrightarrow{\mathcal{D}}_C(\mu x.t) = \mu x.\overrightarrow{\mathcal{D}}_C(t).$$

that $[\![\partial_i \mathrm{op}(x_1, \ldots, x_n)]\!] = \nabla_i [\![\mathrm{op}(x_1, \ldots, x_n)]\!]$, we can lift this interpretation to an interpretation $(\!|-|\!)$ in $\mathbf{Sh}_{\omega\mathrm{CPO}}(\mathcal{O}_{\mathbb{R}})//\mathcal{P}^{\mathbb{R}}_{-} \times \mathcal{P}^{\mathbb{R}}_{-}$ by defining

$$(\!|\mathbf{real}|\!)^V \stackrel{\text{def}}{=} \left\{(f, (f, \nabla f)) \mid f \in \mathcal{P}^V_{\mathbb{R}}\right\} \subseteq \mathcal{P}^V_{\mathbb{R}} \times \mathcal{P}^V_{\mathbb{R}\times\mathbb{R}}.$$

Corollary 8.6. *We obtain an interpretation $(\!|-|\!)$ of CBV FPC over a ground type* **real** *with total and partial operations* op *in* $\mathbf{Sh}_{\omega\mathrm{CPO}}(\mathcal{O}_{\mathbb{R}})//\mathcal{P}^{\mathbb{R}}_{-} \times \mathcal{P}^{\mathbb{R}}_{-}$*, which lifts the interpretation* $([\![-]\!], [\![\overrightarrow{\mathcal{D}}(-)]\!])$ *in* $\omega\mathbf{Diff} \times \omega\mathbf{Diff}$.

Note that this result is interesting as $\omega\mathbf{Diff}$ has the category **Man** of manifolds and smooth functions as a full subcategory and the interpretation $[\![-]\!]$ of values between first-order types lies in **Man**. Moreover, $\omega\mathbf{Diff}_\perp$ has the category of $\mathbf{Man}_\perp$ of manifolds and smooth partial functions defined on open domain as a full subcategory and the interpretation $[\![-]\!]$ of computations between first-order types lies in $\mathbf{Man}_\perp$. As a consequence, the following result follows, as it did for the language with iteration. (Where we define the canonical isomorphisms $\phi^{\overrightarrow{\mathcal{D}}\mathcal{T}}_\tau : [\![\overrightarrow{\mathcal{D}}(\tau)]\!] \to \mathcal{T}([\![\tau]\!])$ as usual.)

Theorem 8.7 (Semantic correctness of $\overrightarrow{\mathcal{D}}$ (full)). *For any ground type $\tau$, any first order context $\Gamma$ and any value $\Gamma \vdash^v v : \tau$ or computation $\Gamma \vdash^c t : \tau$, the syntactic translation $\overrightarrow{\mathcal{D}}$ coincides with the tangent bundle functor, modulo the canonical isomorphisms:*

$$\begin{array}{ccc} [\![\overrightarrow{\mathcal{D}}(\Gamma)]\!] & \xrightarrow{[\![\overrightarrow{\mathcal{D}}_{\mathcal{V}}(v)]\!]} & [\![\overrightarrow{\mathcal{D}}(\tau)]\!] \\ \phi^{\overrightarrow{\mathcal{D}}\mathcal{T}}_{\Gamma}\downarrow\cong & & \cong\downarrow\phi^{\overrightarrow{\mathcal{D}}\mathcal{T}}_{\tau} \\ \mathcal{T}([\![\Gamma]\!]) & \xrightarrow[\mathcal{T}([\![v]\!])]{} & \mathcal{T}([\![\tau]\!]) \end{array} \qquad \begin{array}{ccc} [\![\overrightarrow{\mathcal{D}}(\Gamma)]\!] & \xrightarrow{[\![\overrightarrow{\mathcal{D}}_{C}(t)]\!]} & [\![\overrightarrow{\mathcal{D}}(\tau)]\!]_\perp \\ \phi^{\overrightarrow{\mathcal{D}}\mathcal{T}}_{\Gamma}\downarrow\cong & & \cong\downarrow{\phi^{\overrightarrow{\mathcal{D}}\mathcal{T}}_{\tau}}_{\perp} \\ \mathcal{T}([\![\Gamma]\!]) & \xrightarrow[\mathcal{T}([\![t]\!])]{} & \mathcal{T}([\![\tau]\!])_\perp \end{array}$$

Finally, as long as we choose a sensible interpretation for our operations, in which the denotational and operational semantics agree, we can see that the semantics of our language in $\omega\mathbf{Diff}$ is adequate (by an extension of corollary 5.20, to the ground type **real** and our operations op). Therefore, the denotational semantics can only prove equations which are also contextual equivalences of the operational semantics. This is in particular true for our correctness equations for AD.

Moreover, the model soundly interprets the $\beta\eta$-equational theory of fine-grain FPC (as does any bilimit compact expansion with partial products, coproducts and exponentials). As a consequence, it does not distinguish programs which are optimized via $\beta\eta$-conversion.

## REFERENCES


Jiří Adámek, J Adamek, J Rosicky, et al. 1994. *Locally presentable and accessible categories.* Vol. 189. Cambridge University Press.

Harry Wesley Appelgate. 1965. *Acyclic models and resolvent functors.* Ph.D. Dissertation. Columbia University.

Francis Borceux. 1994. *Handbook of Categorical Algebra: Volume 2, Categories and Structures.* Vol. 50. Cambridge University Press.

Aurelio Carboni and Peter Johnstone. 1995. Connected limits, familial representability and Artin glueing. *Mathematical Structures in Computer Science* 5, 4 (1995), 441–459.

Marcelo P Fiore. 2004. *Axiomatic domain theory in categories of partial maps.* Vol. 14. Cambridge University Press.

Richard Garner and Stephen Lack. 2012. Grothendieck quasitoposes. *Journal of Algebra* 355, 1 (2012), 111–127.

Jean Goubault-Larrecq, Slawomir Lasota, and David Nowak. 2002. Logical relations for monadic types. In *International Workshop on Computer Science Logic.* Springer, 553–568.

Peter T Johnstone. 2002. *Sketches of an elephant: A topos theory compendium.* Vol. 2. Oxford University Press.

Peter T Johnstone, Stephen Lack, and P Sobocinski. 2007. Quasitoposes, Quasiadhesive Categories and Artin Glueing. In *Proc. CALCO 2007.*

Paul Blain Levy. 2012. *Call-by-push-value: A Functional/imperative Synthesis.* Vol. 2. Springer Science & Business Media.

Saunders MacLane and Ieke Moerdijk. 2012. *Sheaves in geometry and logic: A first introduction to topos theory*. Springer Science & Business Media.

John C Mitchell and Andre Scedrov. 1992. Notes on sconing and relators. In *International Workshop on Computer Science Logic*. Springer, 352–378.

Philip S Mulry. 1993. Lifting theorems for Kleisli categories. In *International Conference on Mathematical Foundations of Programming Semantics*. Springer, 304–319.

Erik Palmgren and Viggo Stoltenberg-Hansen. 1990. Domain interpretations of Martin-Löf's partial type theory. *Annals of Pure and Applied Logic* 48, 2 (1990), 135–196.

Andrew M Pitts. 1996. Relational properties of domains. *Inform. Comput.* 127, 2 (1996), 66–90.

David E Rydeheard and Rod M Burstall. 1988. *Computational category theory*. Vol. 152. Prentice Hall Englewood Cliffs.

Michael B. Smyth and Gordon D. Plotkin. 1982. The category-theoretic solution of recursive domain equations. *SIAM J. Comput.* 11, 4 (1982), 761–783.

Matthijs Vákár, Ohad Kammar, and Sam Staton. 2019. A domain theory for statistical probabilistic programming. *Proceedings of the ACM on Programming Languages* 3, POPL (2019), 36.
